# Supplementary material for: A low cost singular value decomposition based data assimilation technique for analysis of heterogeneous combustion data
Source: arXiv:2503.24064 source file (2025-03-31)
Supplement: Supplementary file 1 [file Appendix.pdf]

Laminar co-flow flame with methane and nitrogen as fuel. (Reconstruction comparison)

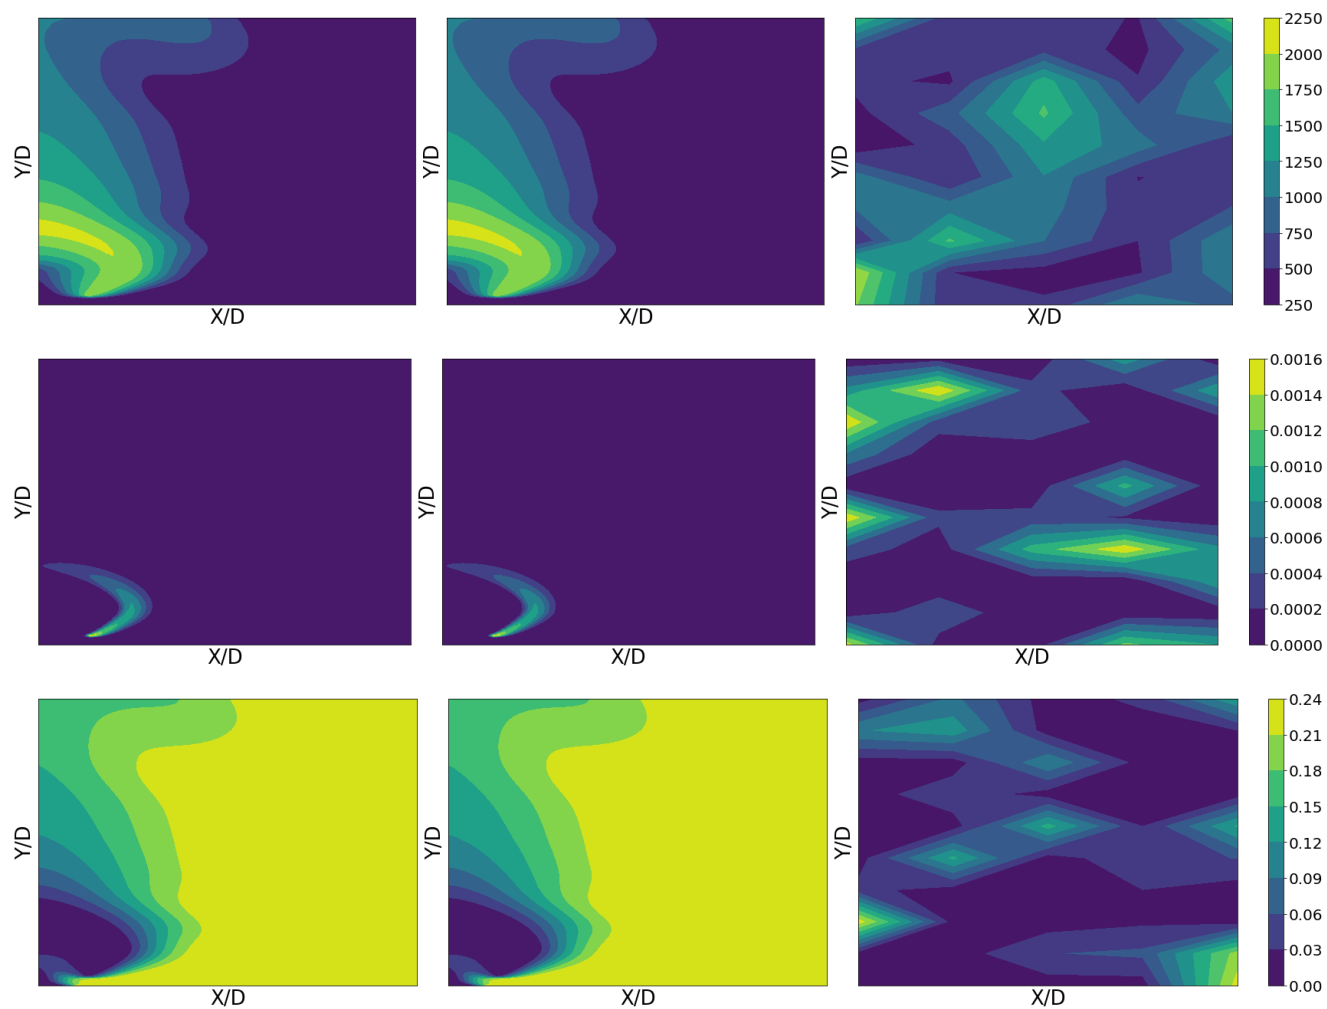

Reconstruction lcSVD optimum sensors (left), ground truth (middle) and downsampled matrix (right) for variables  $T, O, O_2$  (top to bottom) in a laminar co-flow flame with methane and nitrogen as fuel.

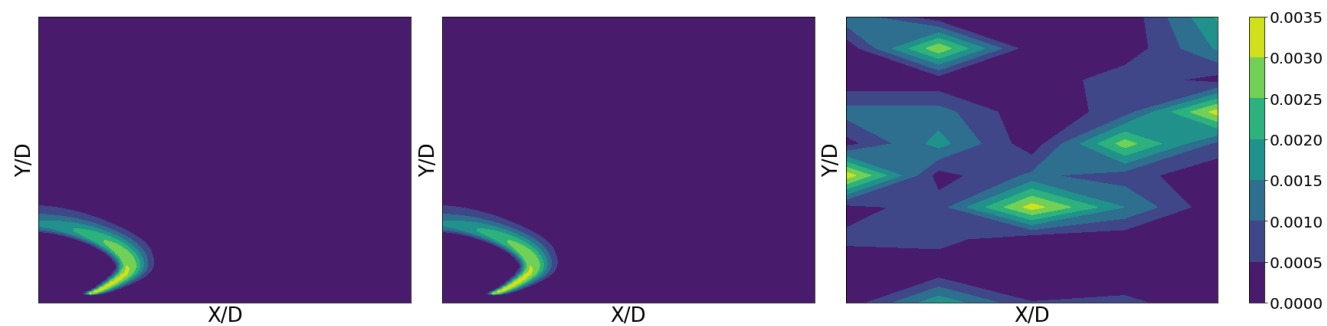

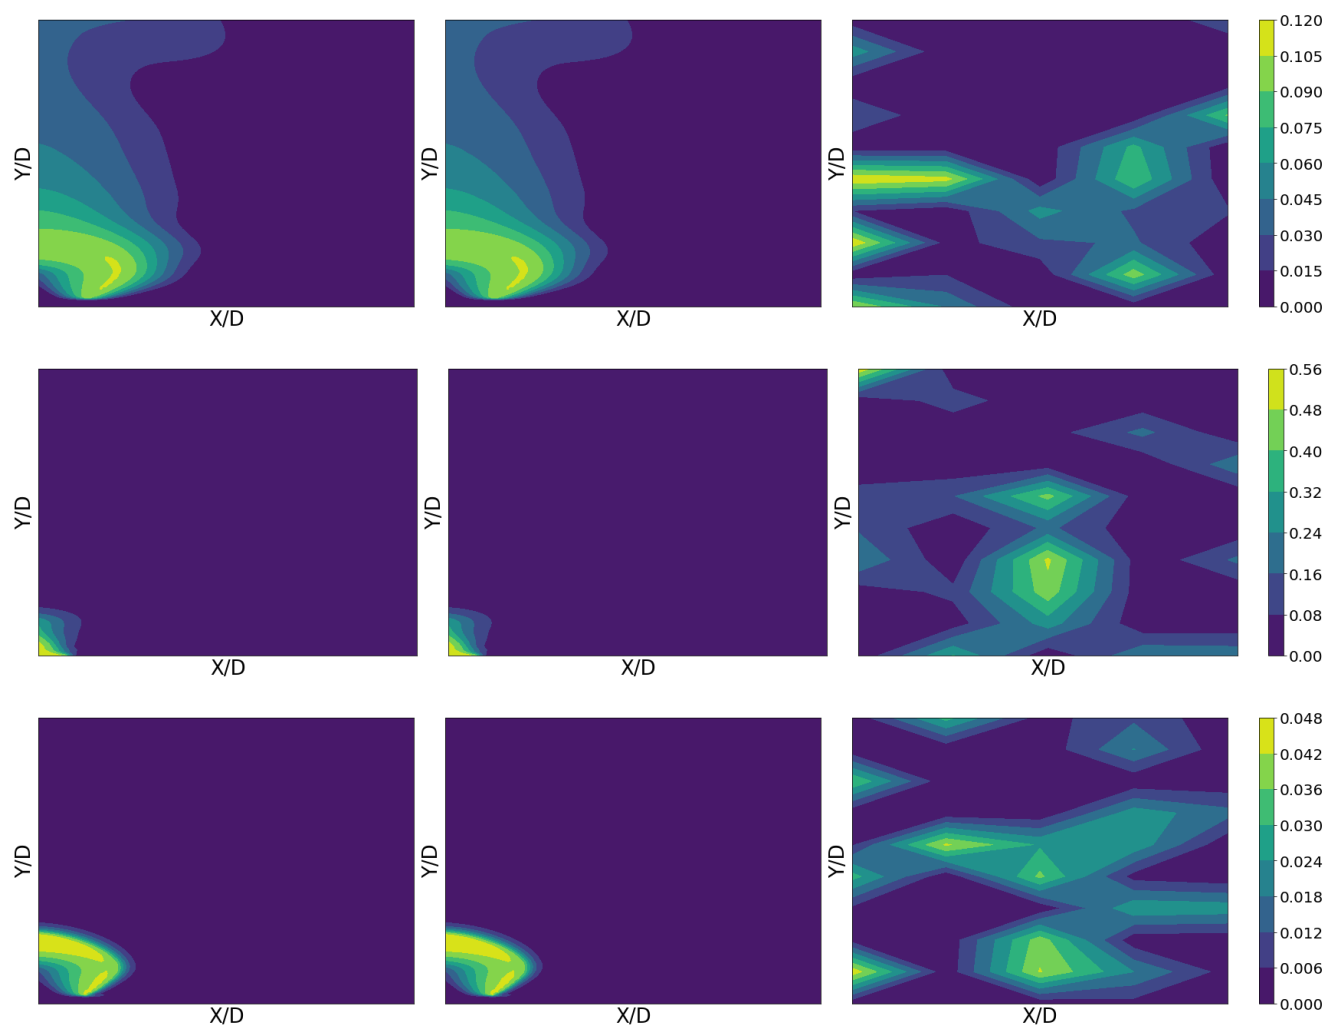

Reconstruction lcSVD optimum sensors (left), ground truth (middle) and downsampled matrix (right) for variables  $OH$ ,  $H_2O$ ,  $CH_4$ ,  $CO$  (top to bottom) in a laminar co-flow flame with methane and nitrogen as fuel.

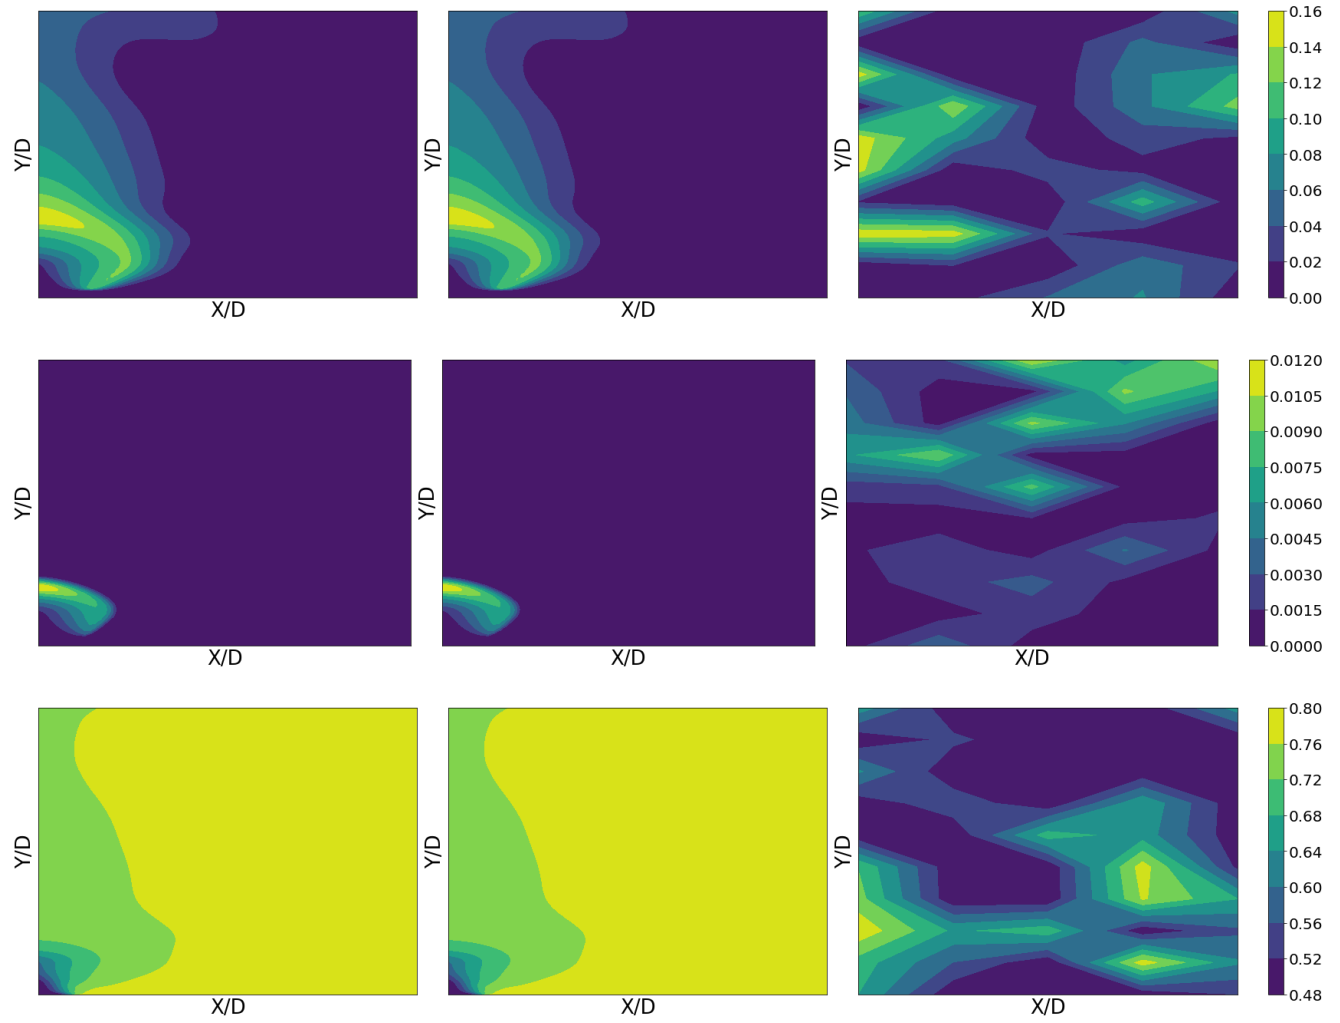

Reconstruction lcSVD optimum sensors (left), ground truth (middle) and downsampled matrix (right) for variables  $CO_2, C_2H_2, N_2$  (top to bottom) in a laminar co-flow flame with methane and nitrogen as fuel.

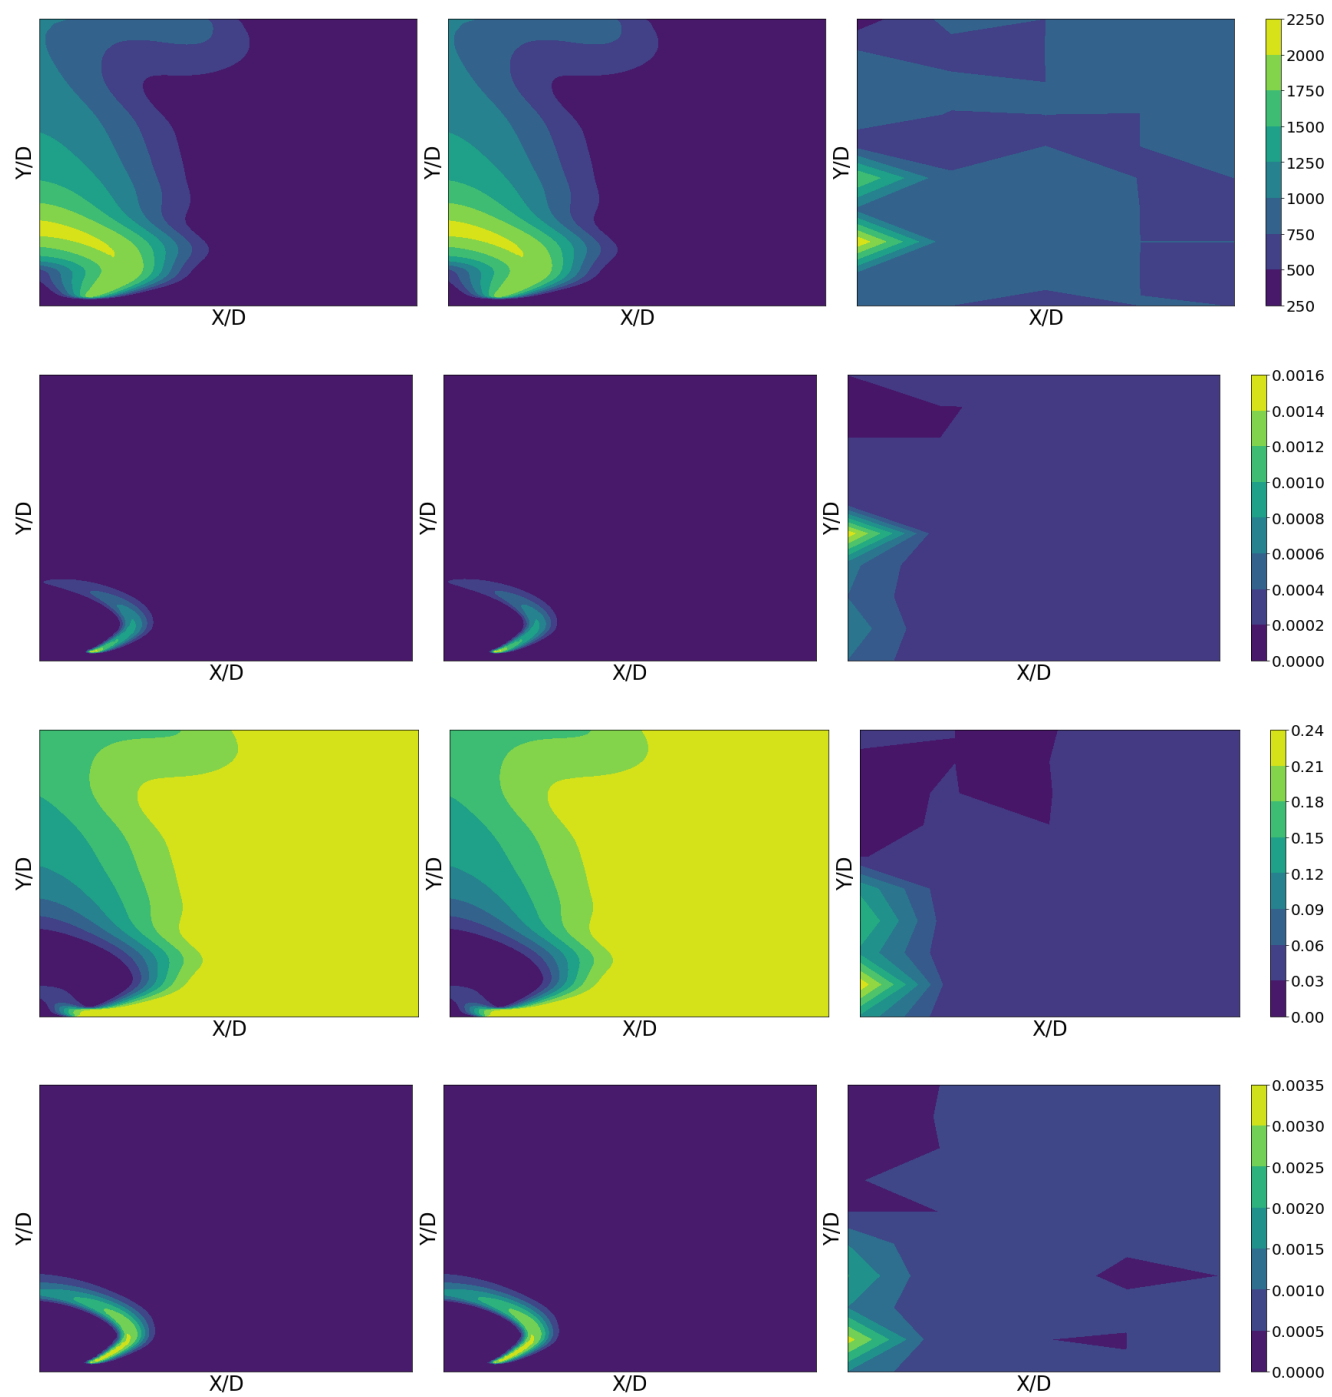

Reconstruction lcSVD using equally spaced samples (left), ground truth (middle) and downsampled matrix (right) for variables  $T, O, O_2, OH$  (top to bottom) in a laminar co-flow flame with methane and nitrogen as fuel.

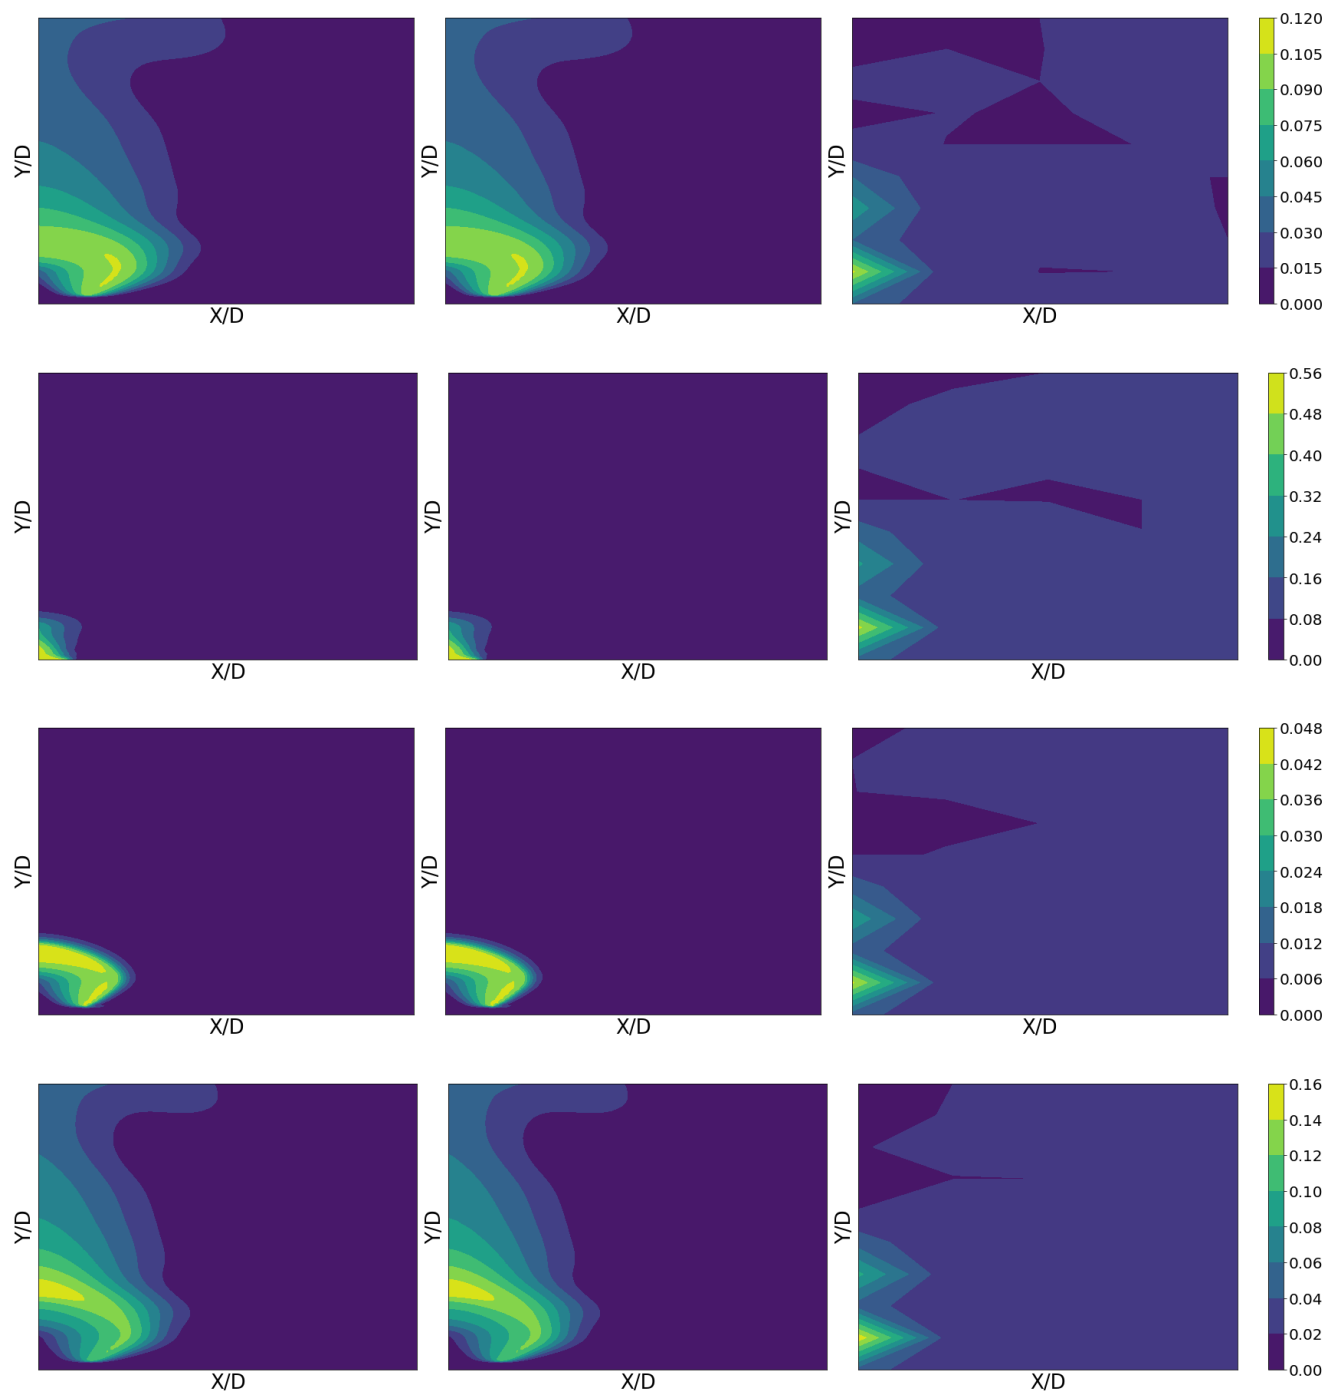

Reconstruction lcSVD equally spaced samples (left), ground truth (middle) and downsampled matrix (right) for variables  $H_2O$ ,  $CH_4$ ,  $CO$ ,  $CO_2$  (top to bottom) in a laminar co-flow flame with methane and nitrogen as fuel.

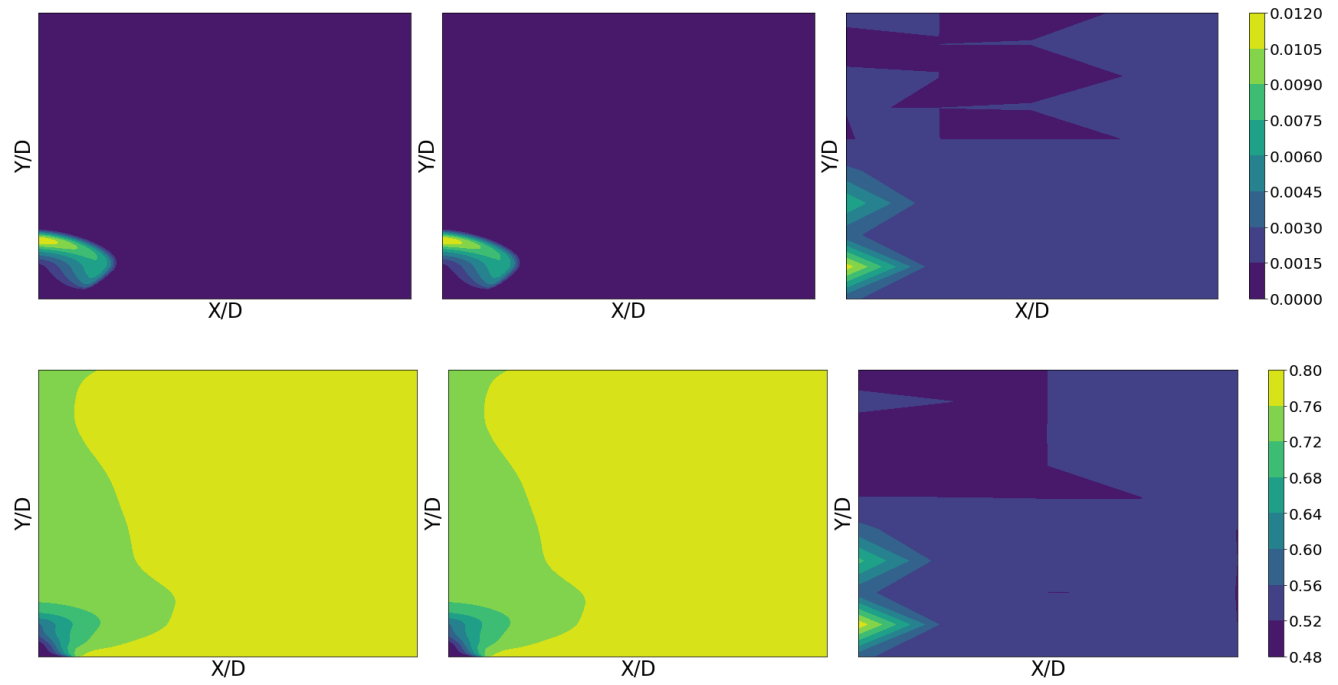

Reconstruction lcSVD equally spaced samples (left), ground truth (middle) and downsampled matrix (right) for variables  $C_2H_2, N_2$  (top to bottom) in a laminar co-flow flame with methane and nitrogen as fuel.

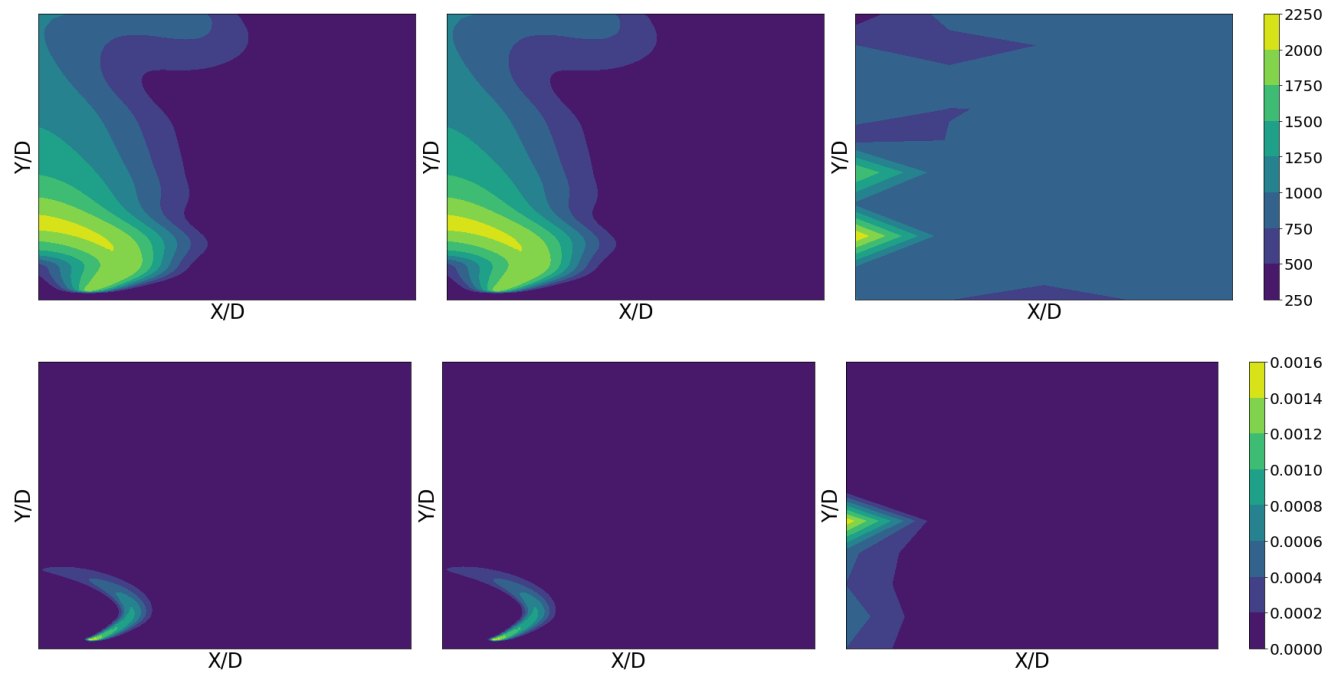

Reconstruction using lcSVD -DA (left), ground truth (middle) and downsampled matrix (right) for variables  $T, O$  (top to bottom) in a laminar co-flow flame with methane and nitrogen as fuel.

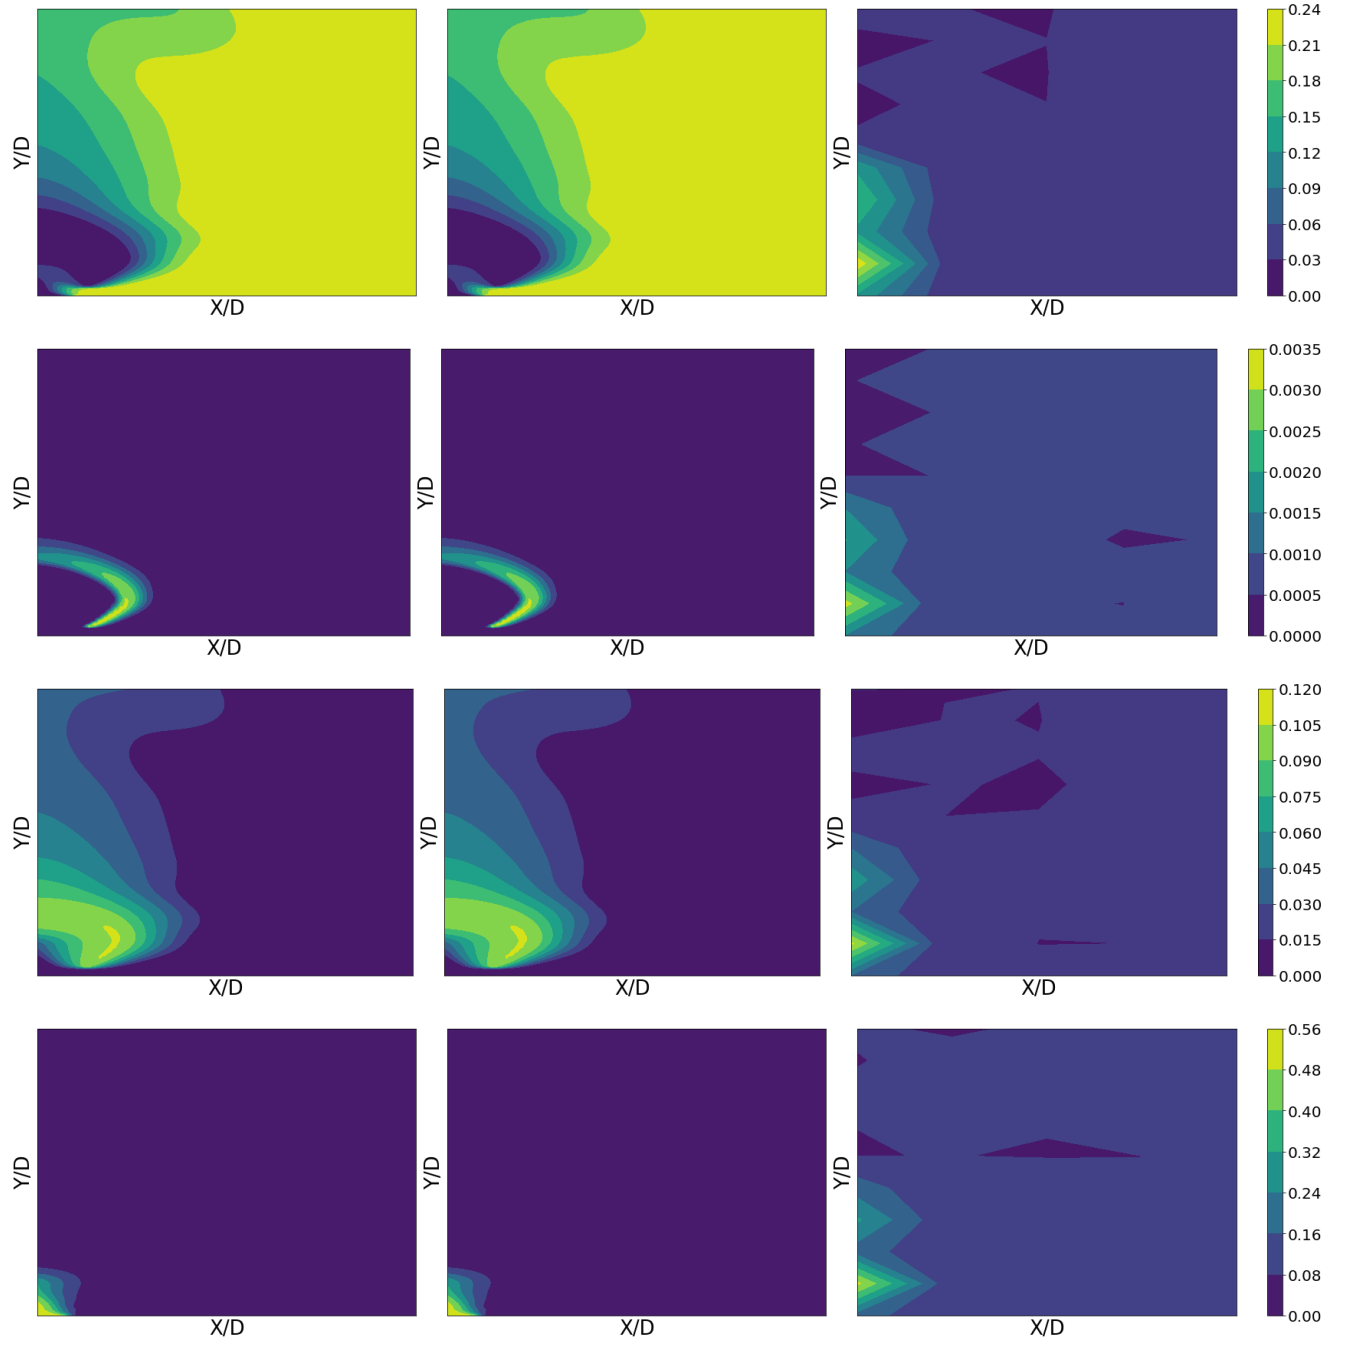

Reconstruction lcSVD -DA (left), ground truth (middle) and downsampled matrix (right) for variables  $O_2, OH, H_2O, CH_4$  (top to bottom) in a laminar co-flow flame with methane and nitrogen as fuel.

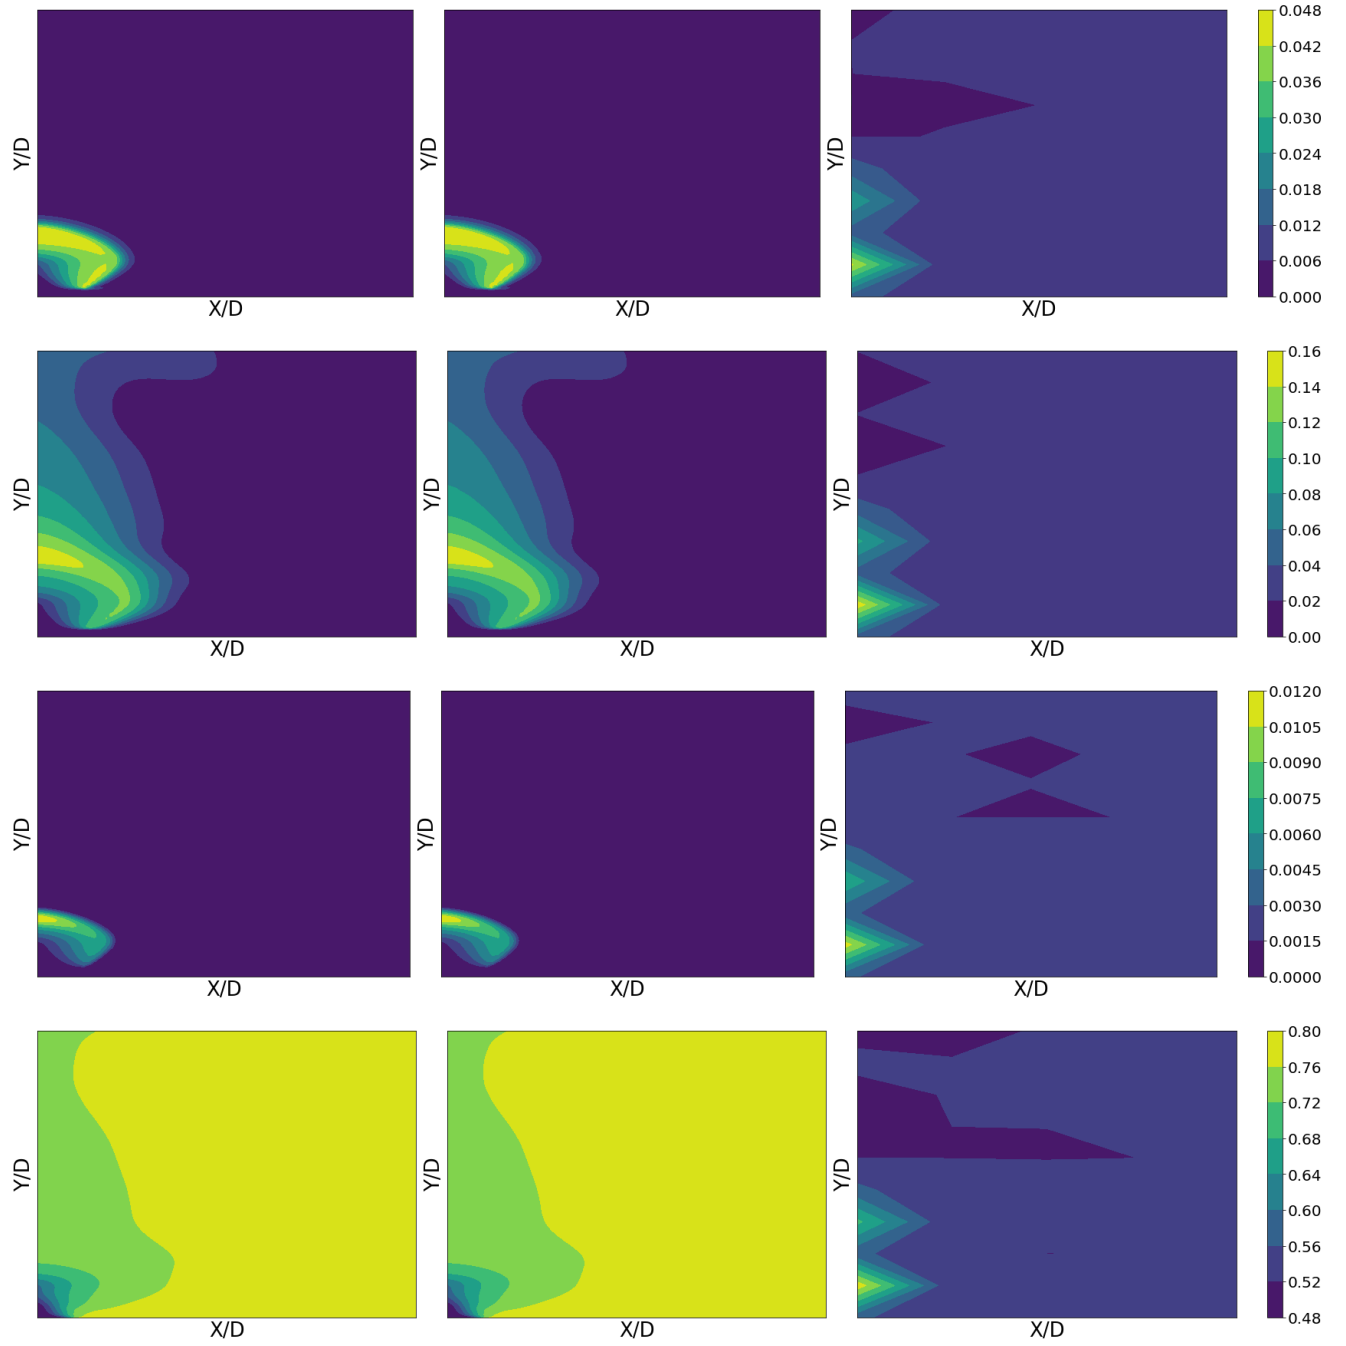

Reconstruction lcSVD -DA (left), ground truth (middle) and downsampled matrix (right) for variables  $CO, CO_2, C_2H_2, N_2$  (top to bottom) in a laminar co-flow flame with methane and nitrogen as fuel.

Laminar co-flow flame with methane and nitrogen as fuel. (Modes comparison)

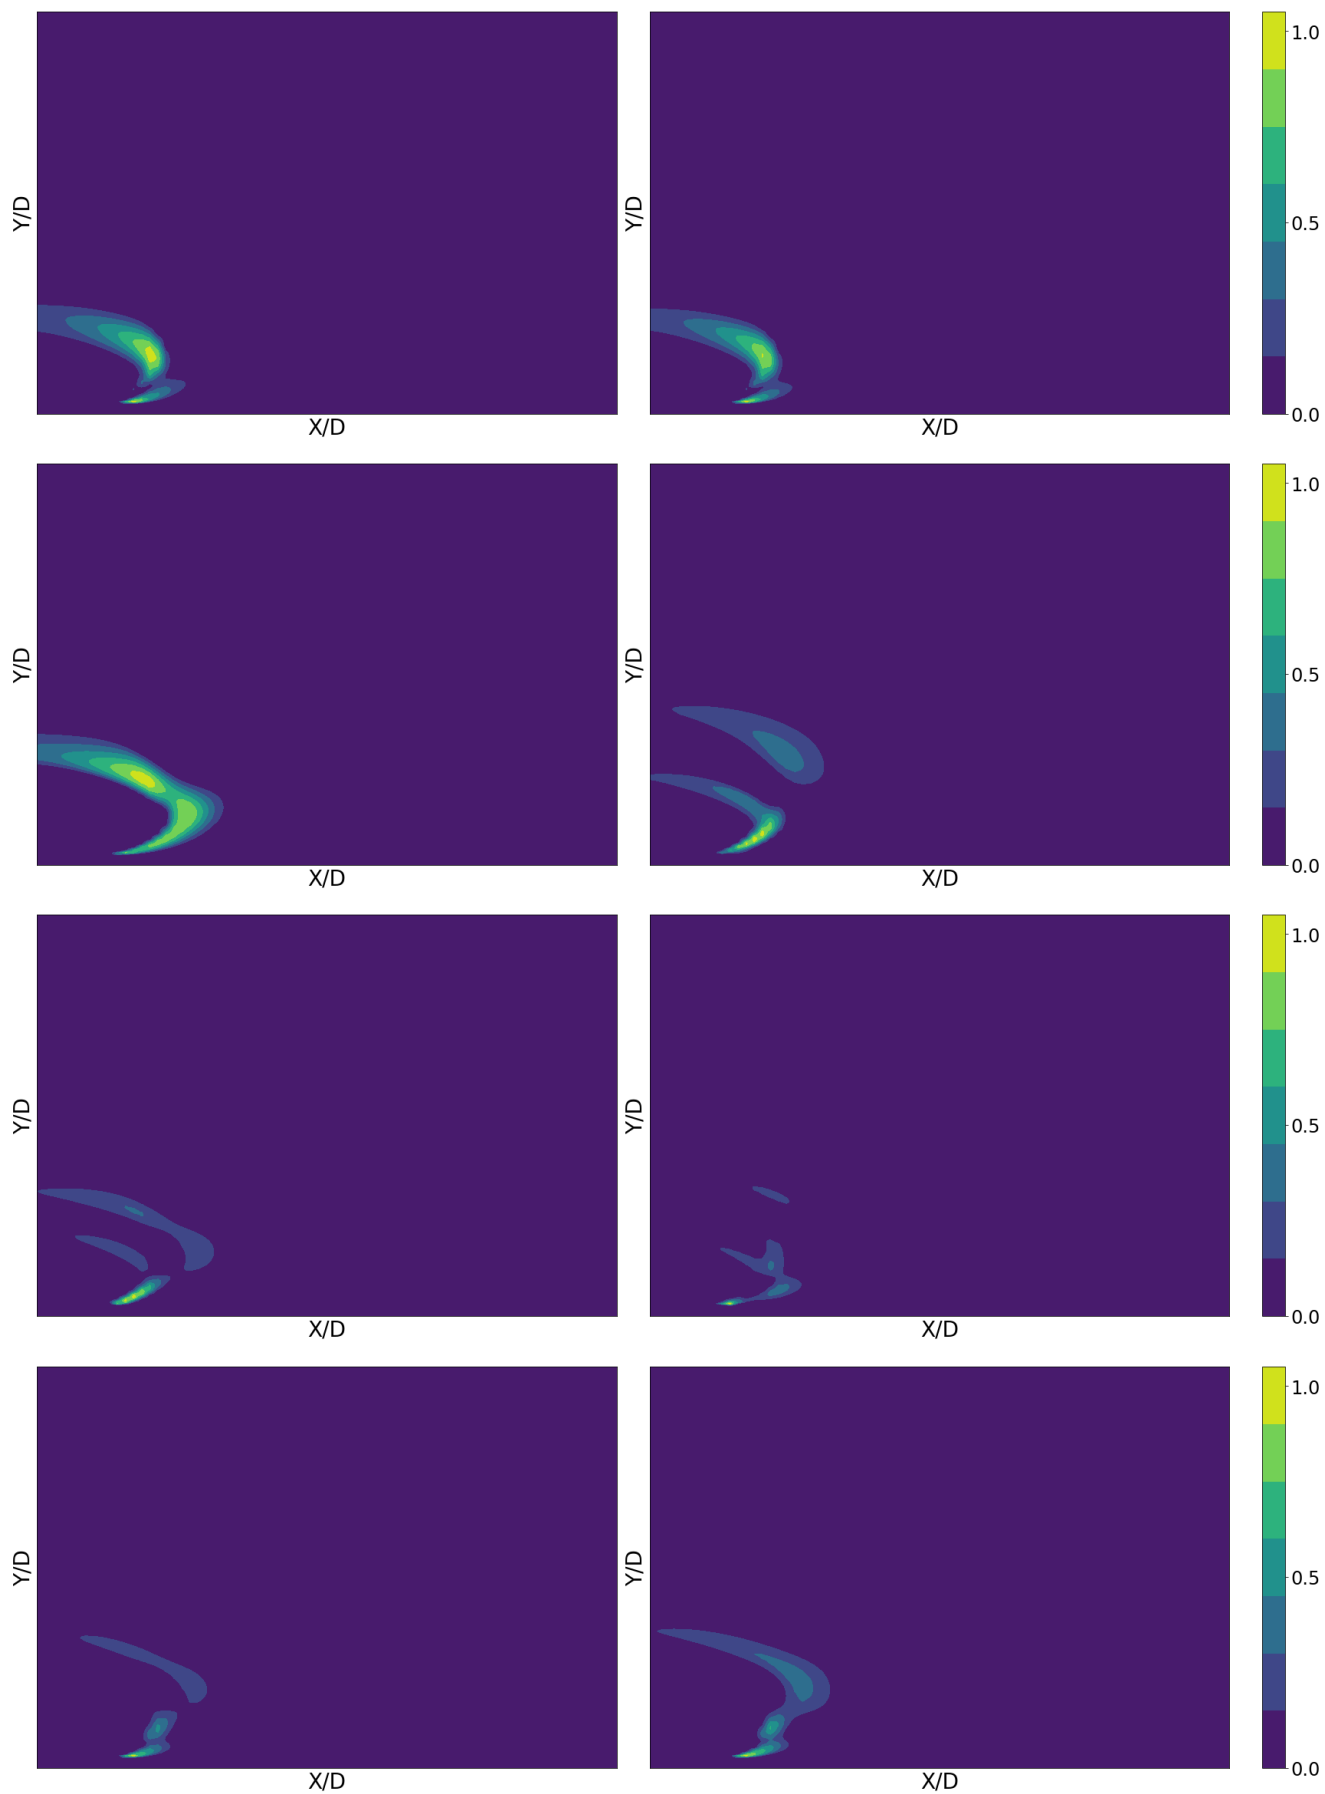

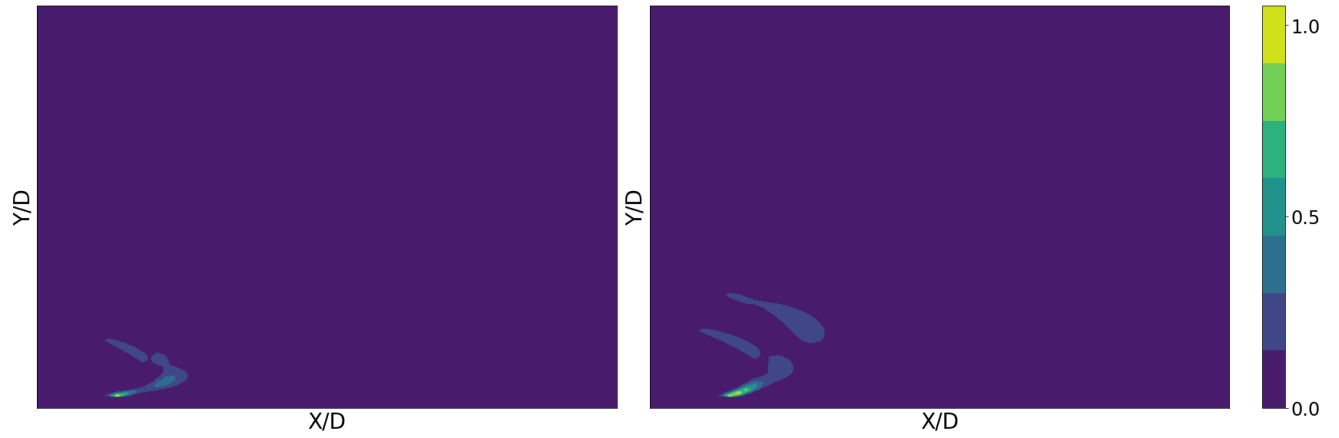

The first five weighted 2D Proper Orthogonal Decomposition (POD) spatial modes, comparing lcSVD optimum sensors(left) with the ground truth (right) for the variable  $O$  in the laminar co flow flame dataset. With 20\% of modes retained, the modes are arranged from top to bottom in order of decreasing energy.

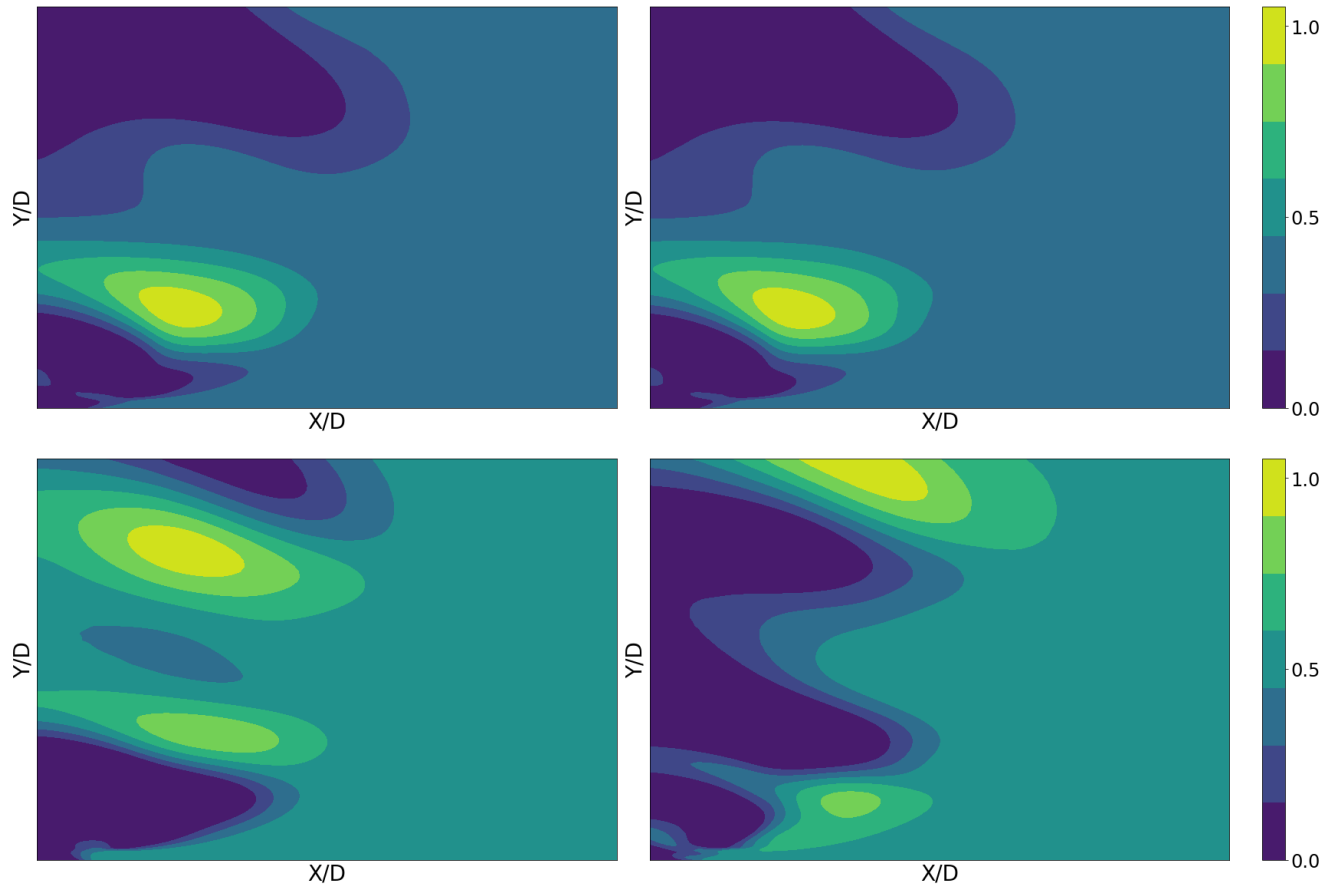

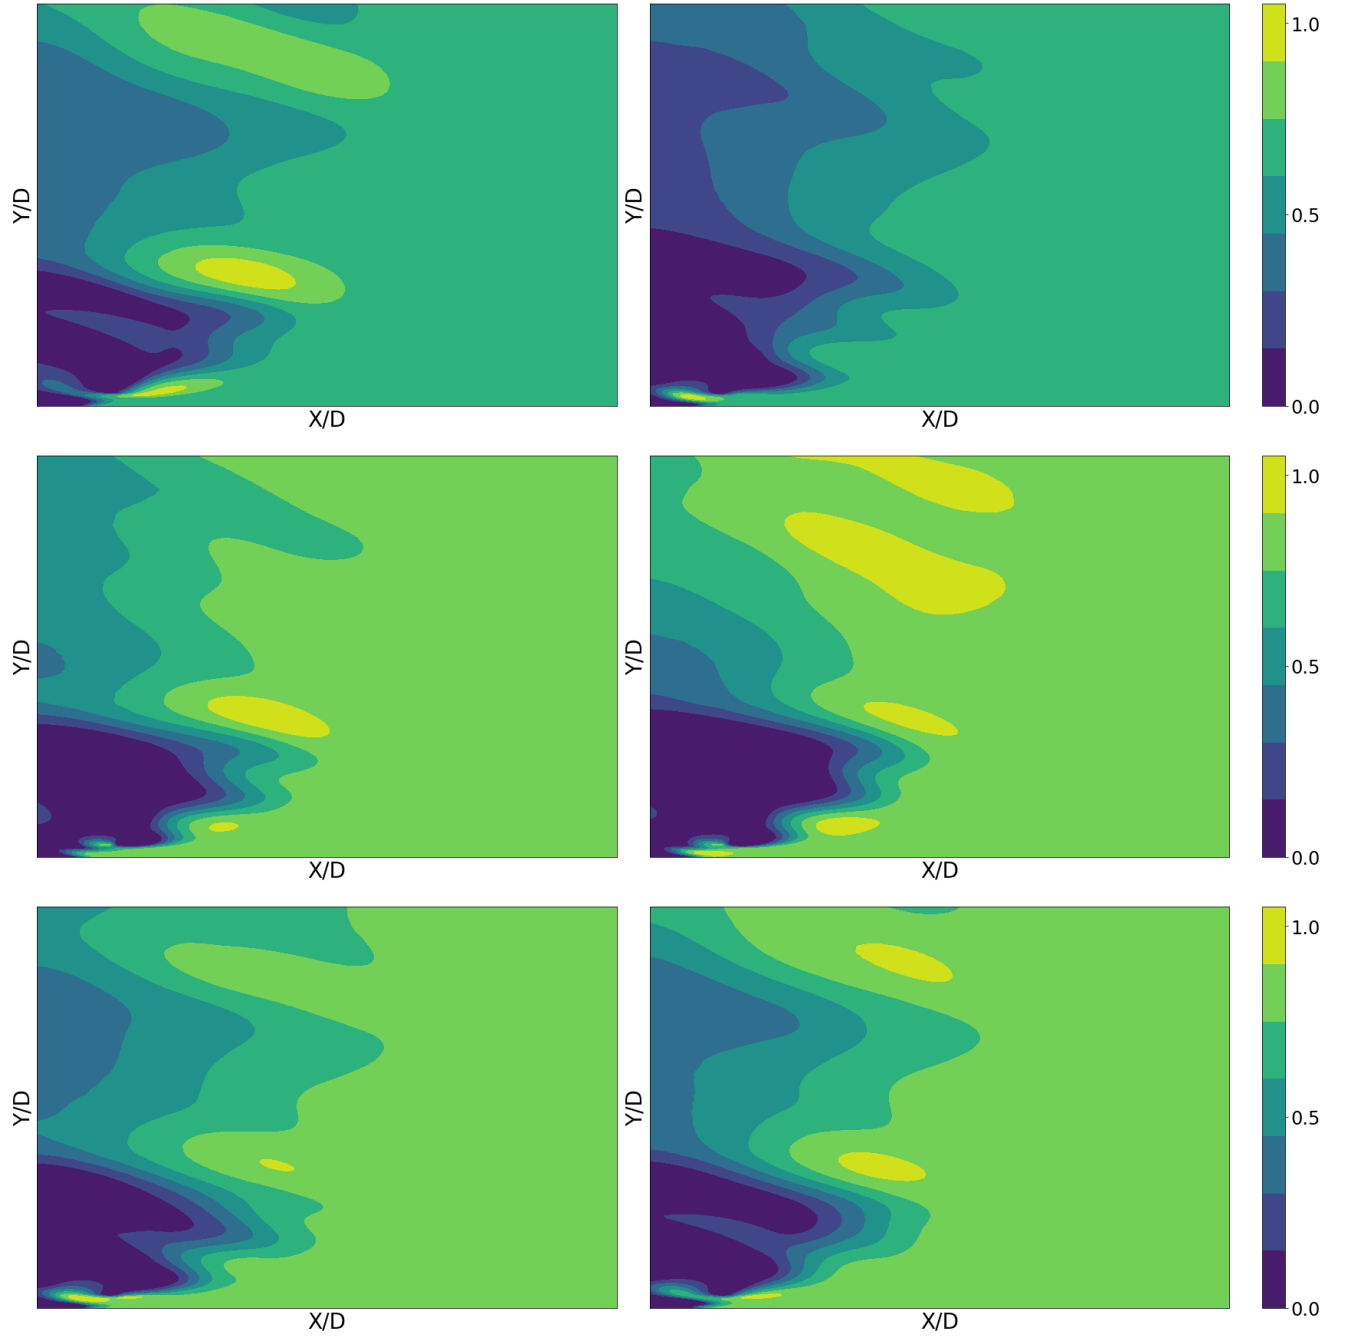

The normalized first five weighted 2D Proper Orthogonal Decomposition (POD) spatial modes, comparing lcSVD optimum sensors(left) with the ground truth (right) for the variable  $O_2$  in the laminar co flow flame dataset. With 20\% of modes retained, the modes are arranged from top to bottom in order of decreasing energy.

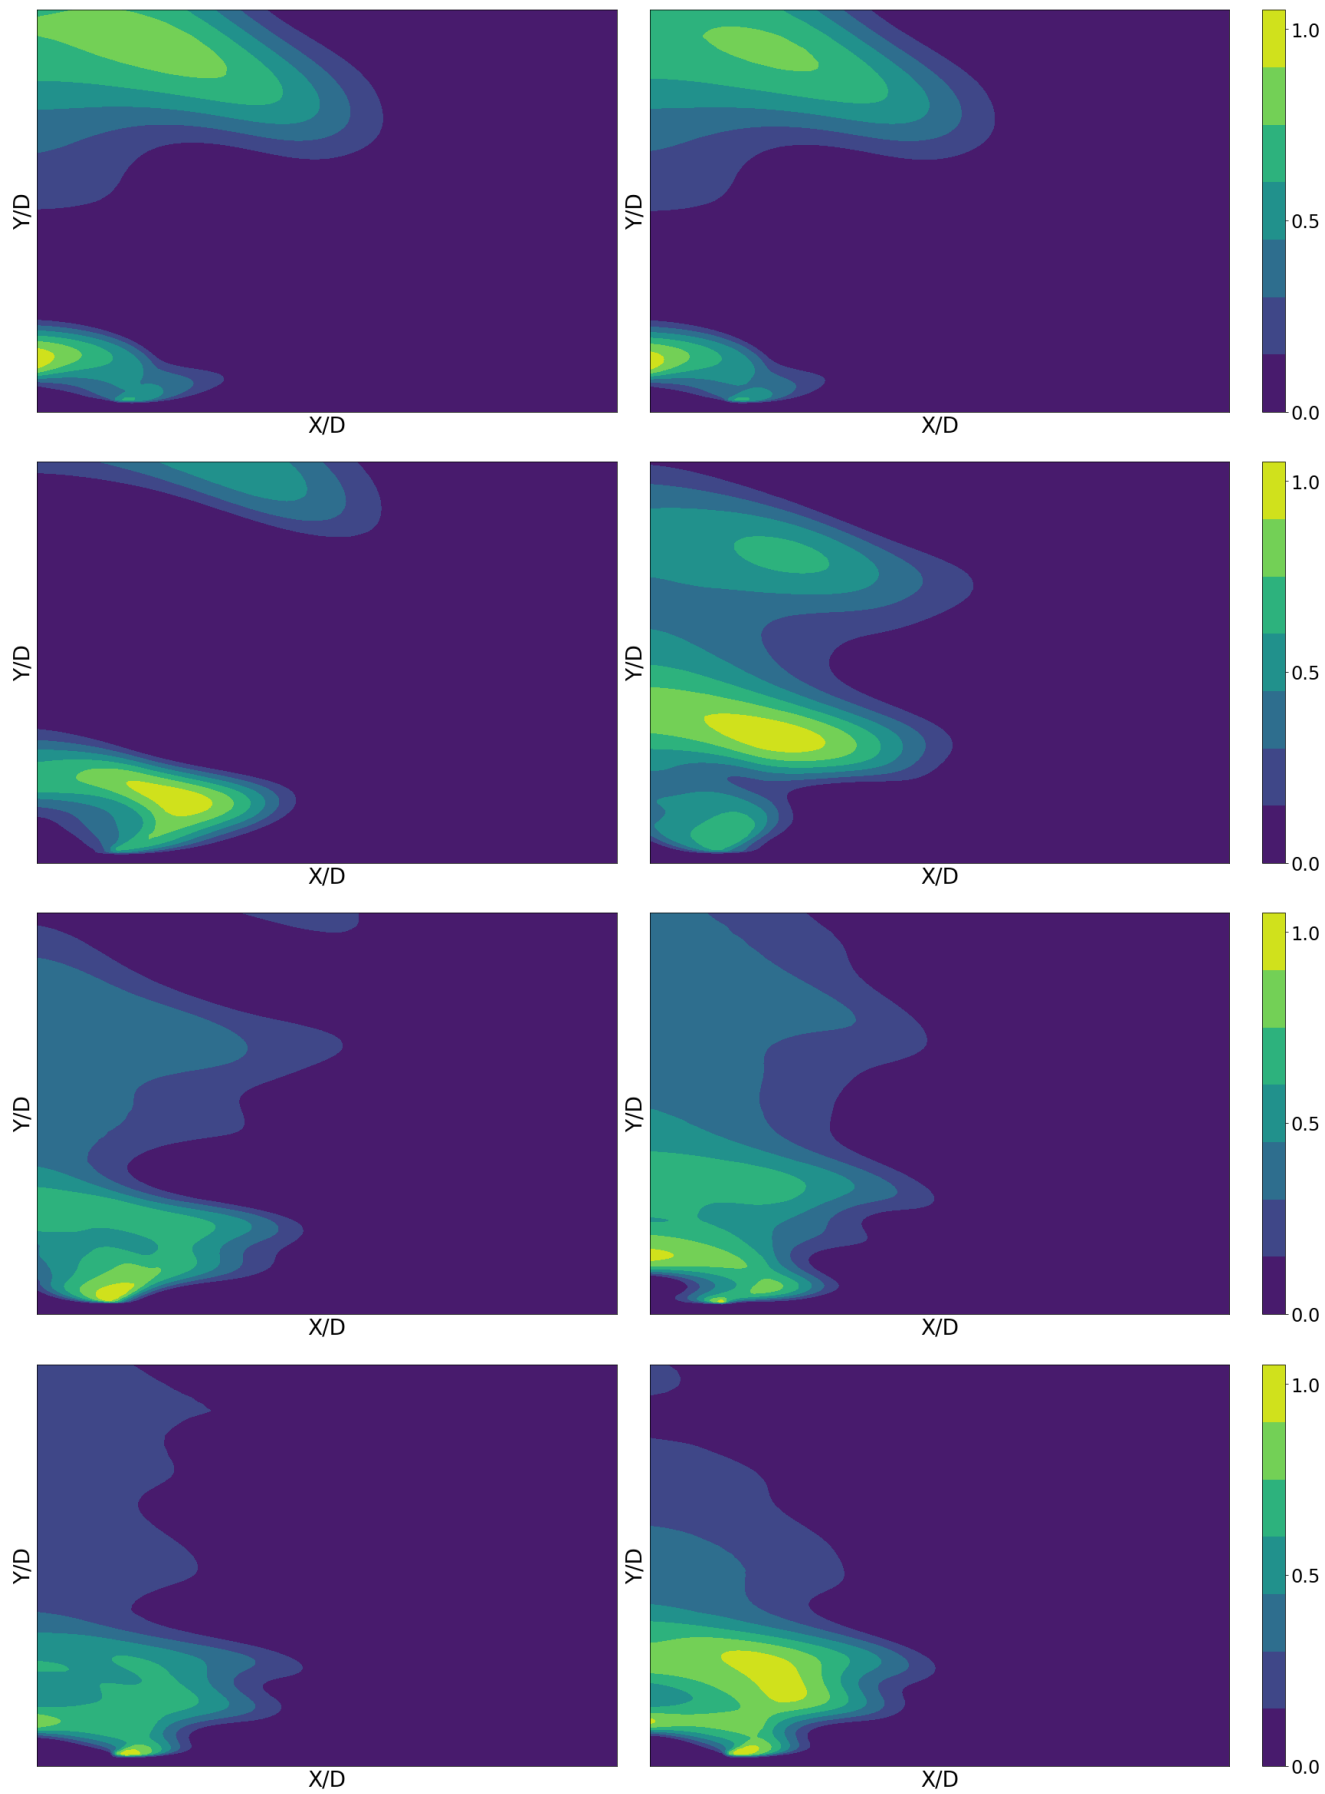

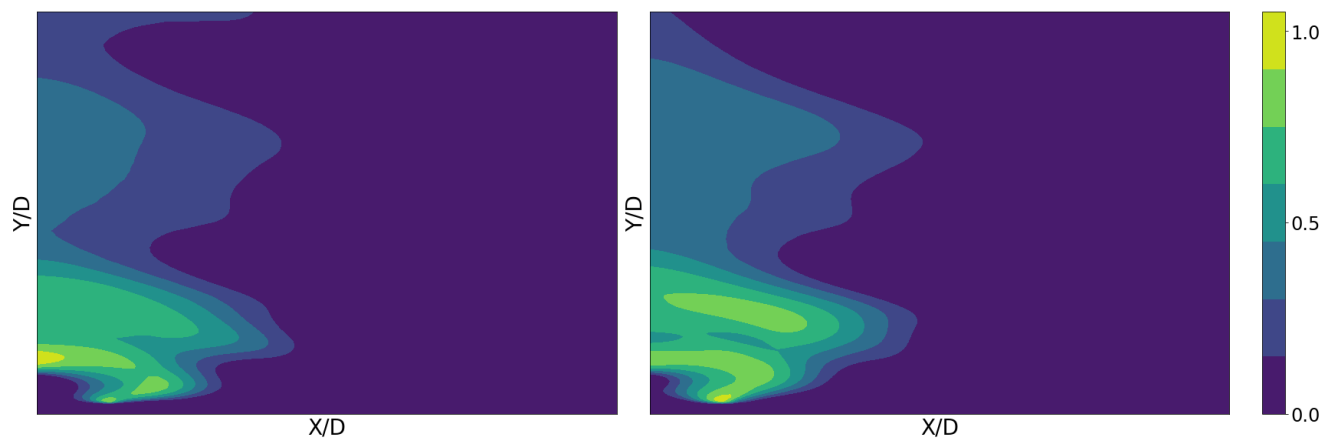

The normalized first five weighted 2D Proper Orthogonal Decomposition (POD) spatial modes, comparing lcSVD optimum sensors(left) with the ground truth (right) for the variable  $H_2O$  in the laminar co flow flame dataset. With 20\% of modes retained, the modes are arranged from top to bottom in order of decreasing energy.

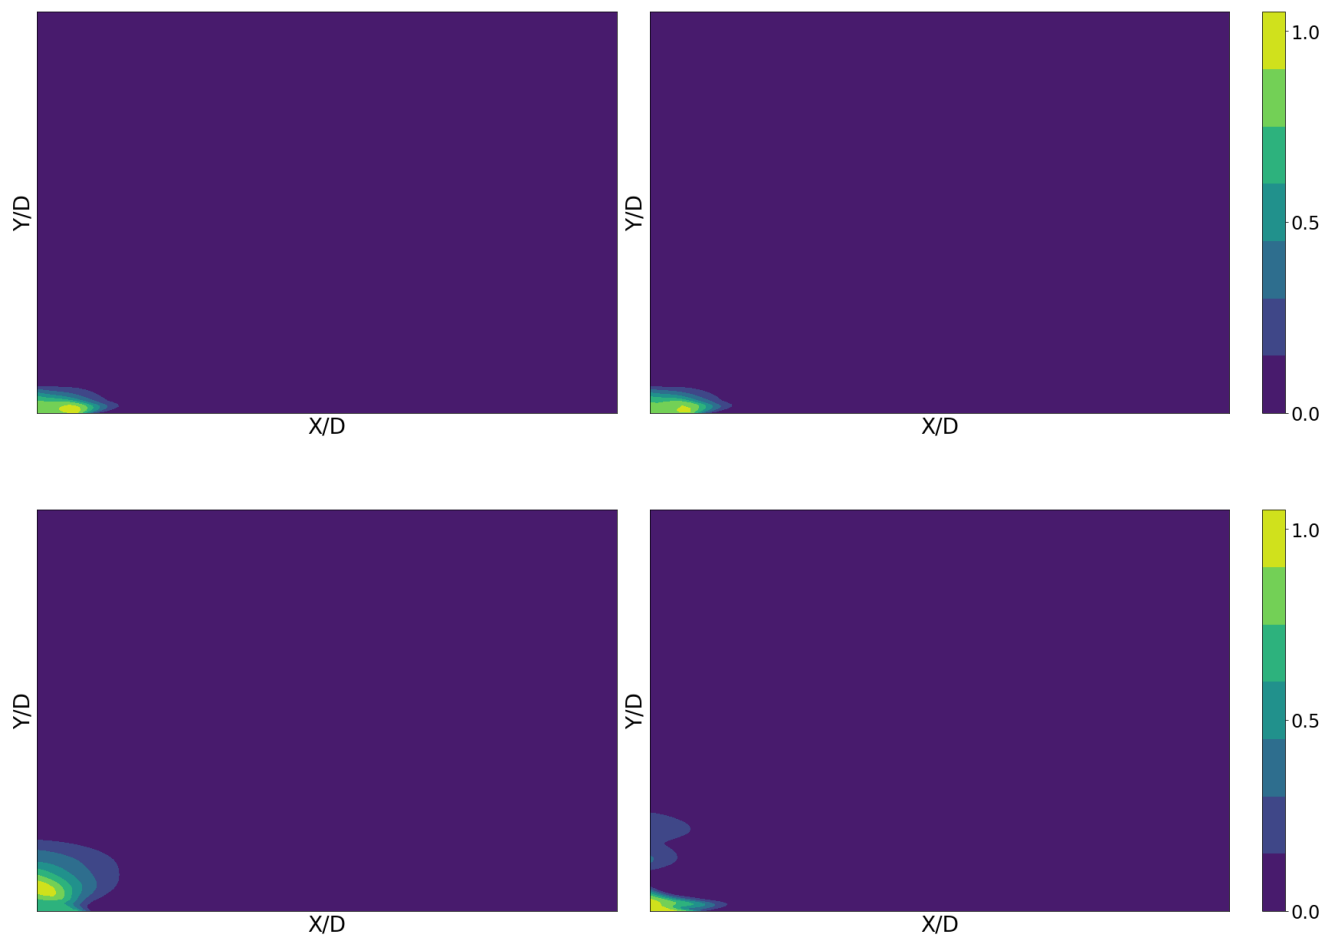

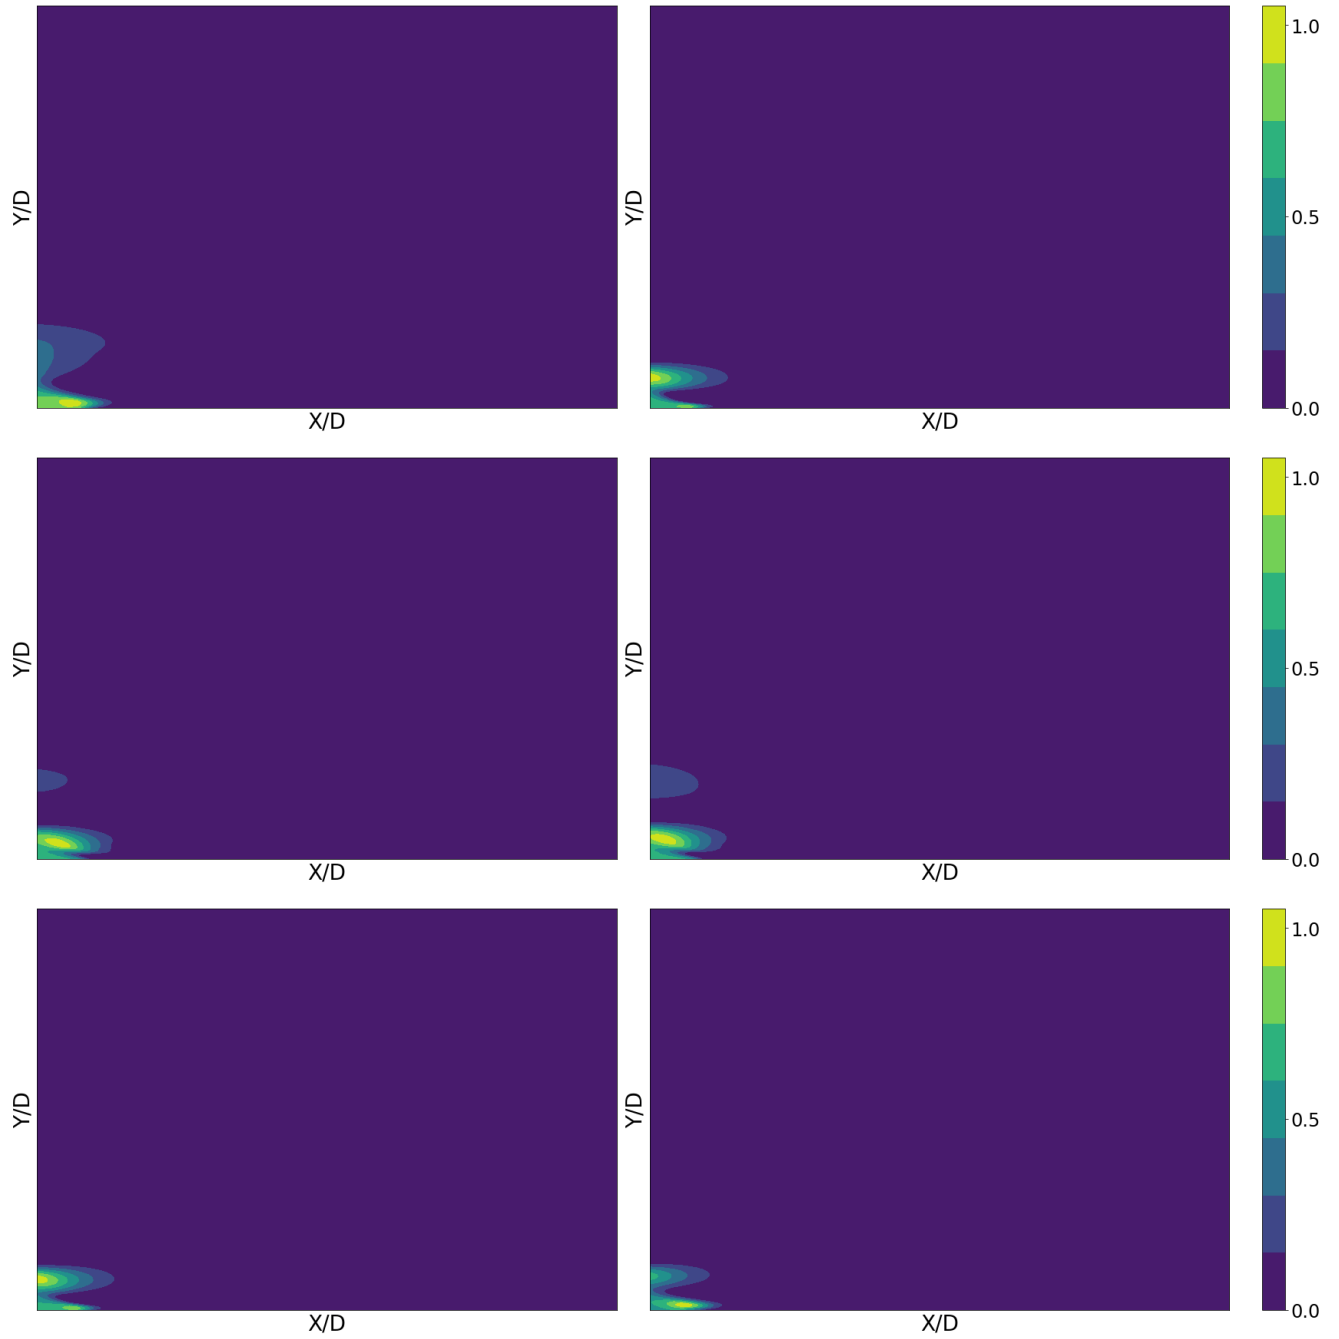

The normalized first five weighted 2D Proper Orthogonal Decomposition (POD) spatial modes, comparing lcSVD optimum sensors(left) with the ground truth (right) for the variable  $CH_4$  in the laminar co flow flame dataset. With 20\% of modes retained, the modes are arranged from top to bottom in order of decreasing energy.

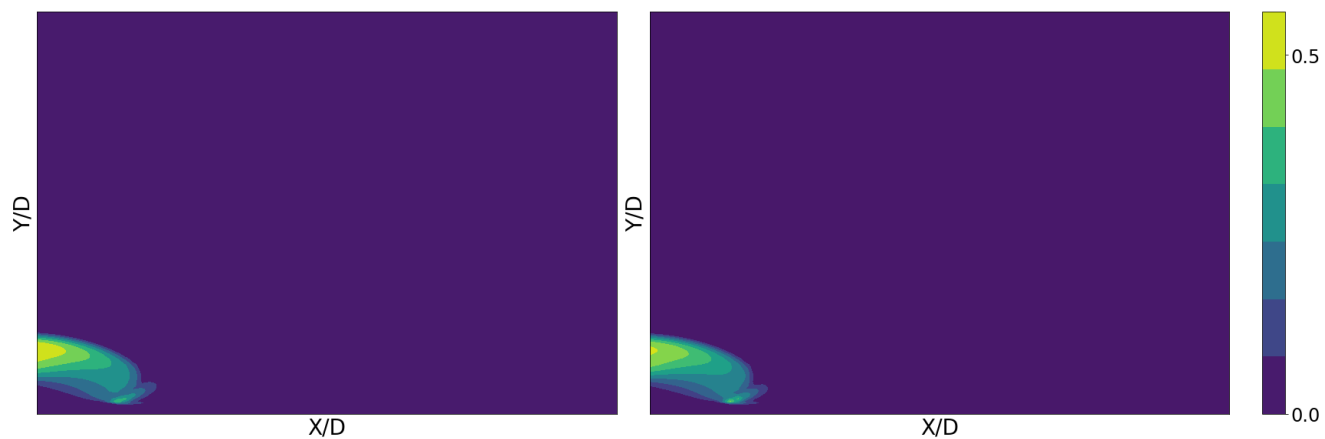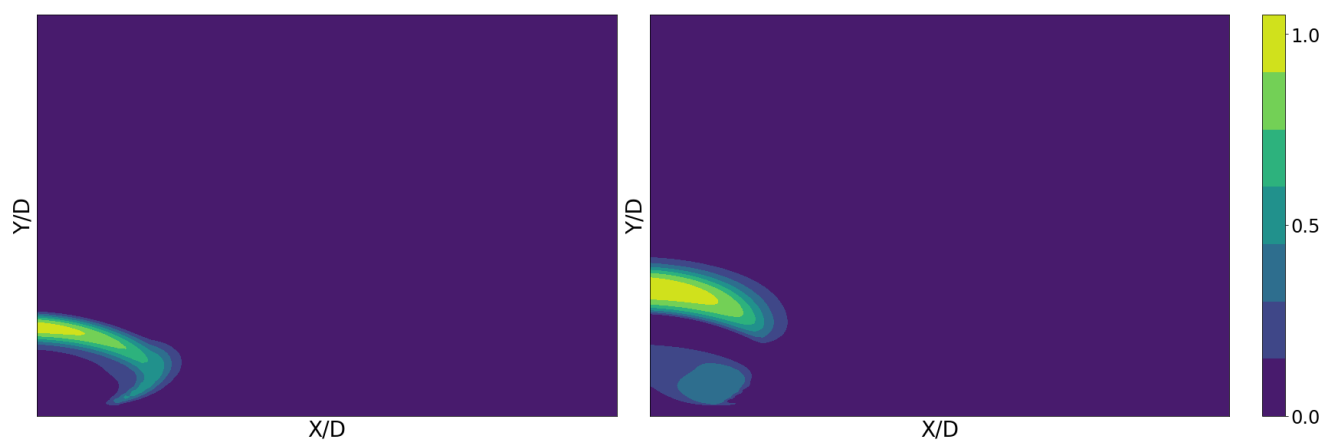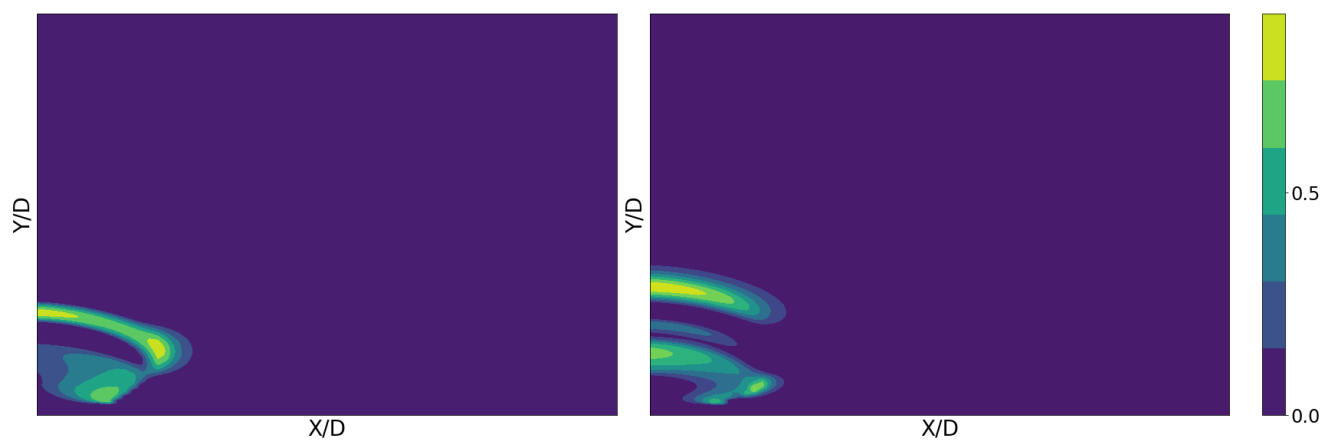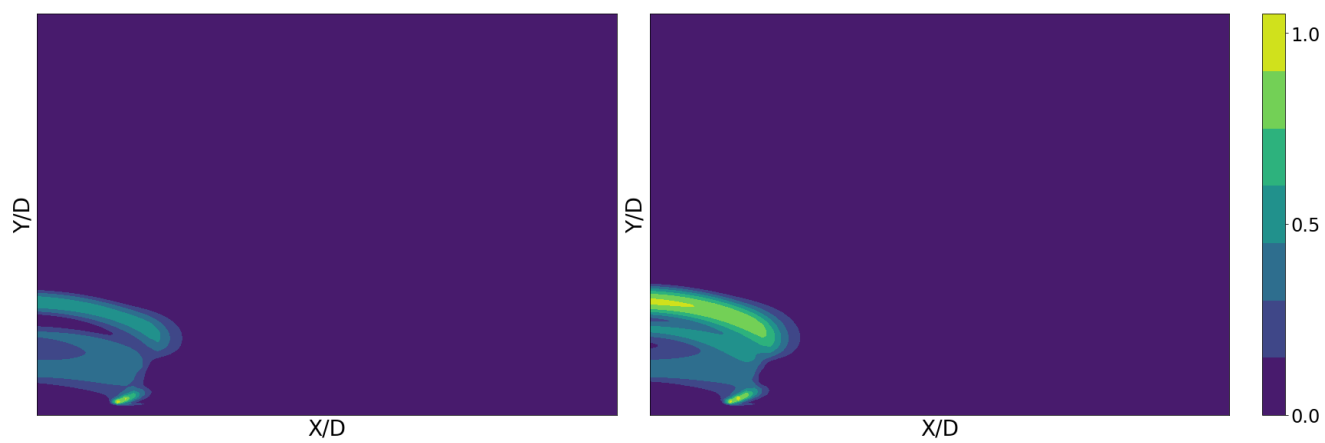

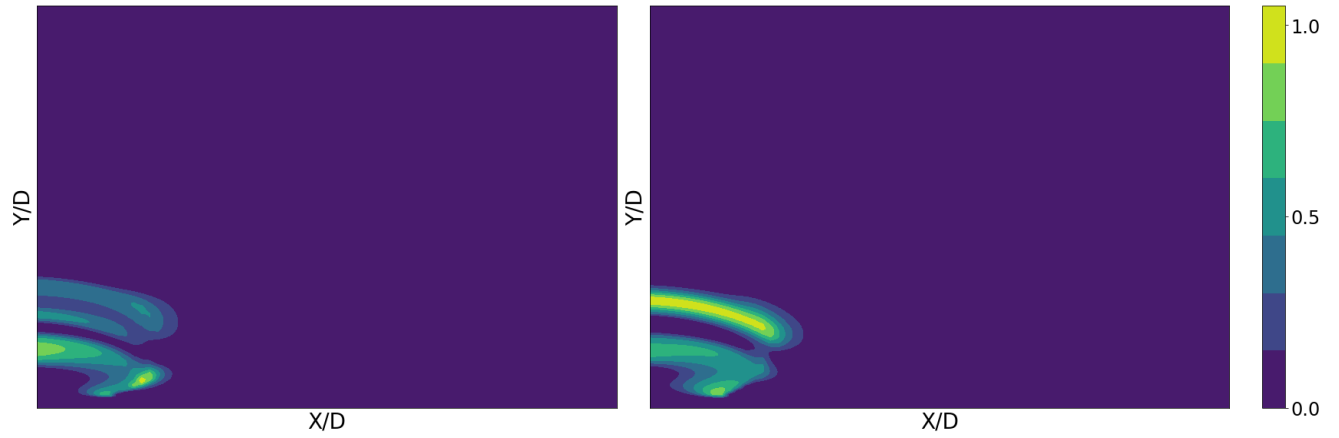

The normalized first five weighted 2D Proper Orthogonal Decomposition (POD) spatial modes, comparing lcSVD optimum sensors(left) with the ground truth (right) for the variable  $CO$  in the laminar co flow flame dataset. With 20% of modes retained, the modes are arranged from top to bottom in order of decreasing energy.

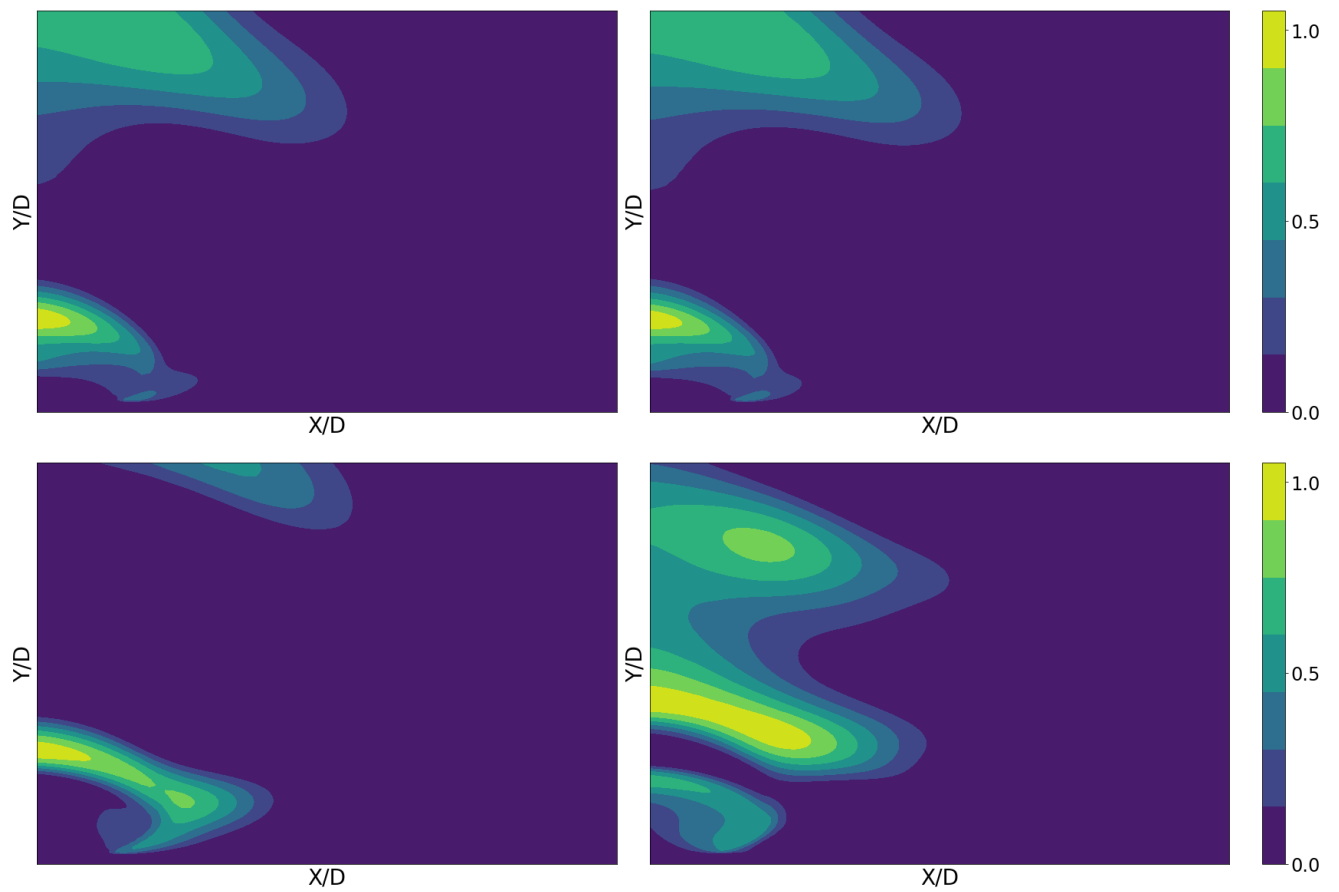

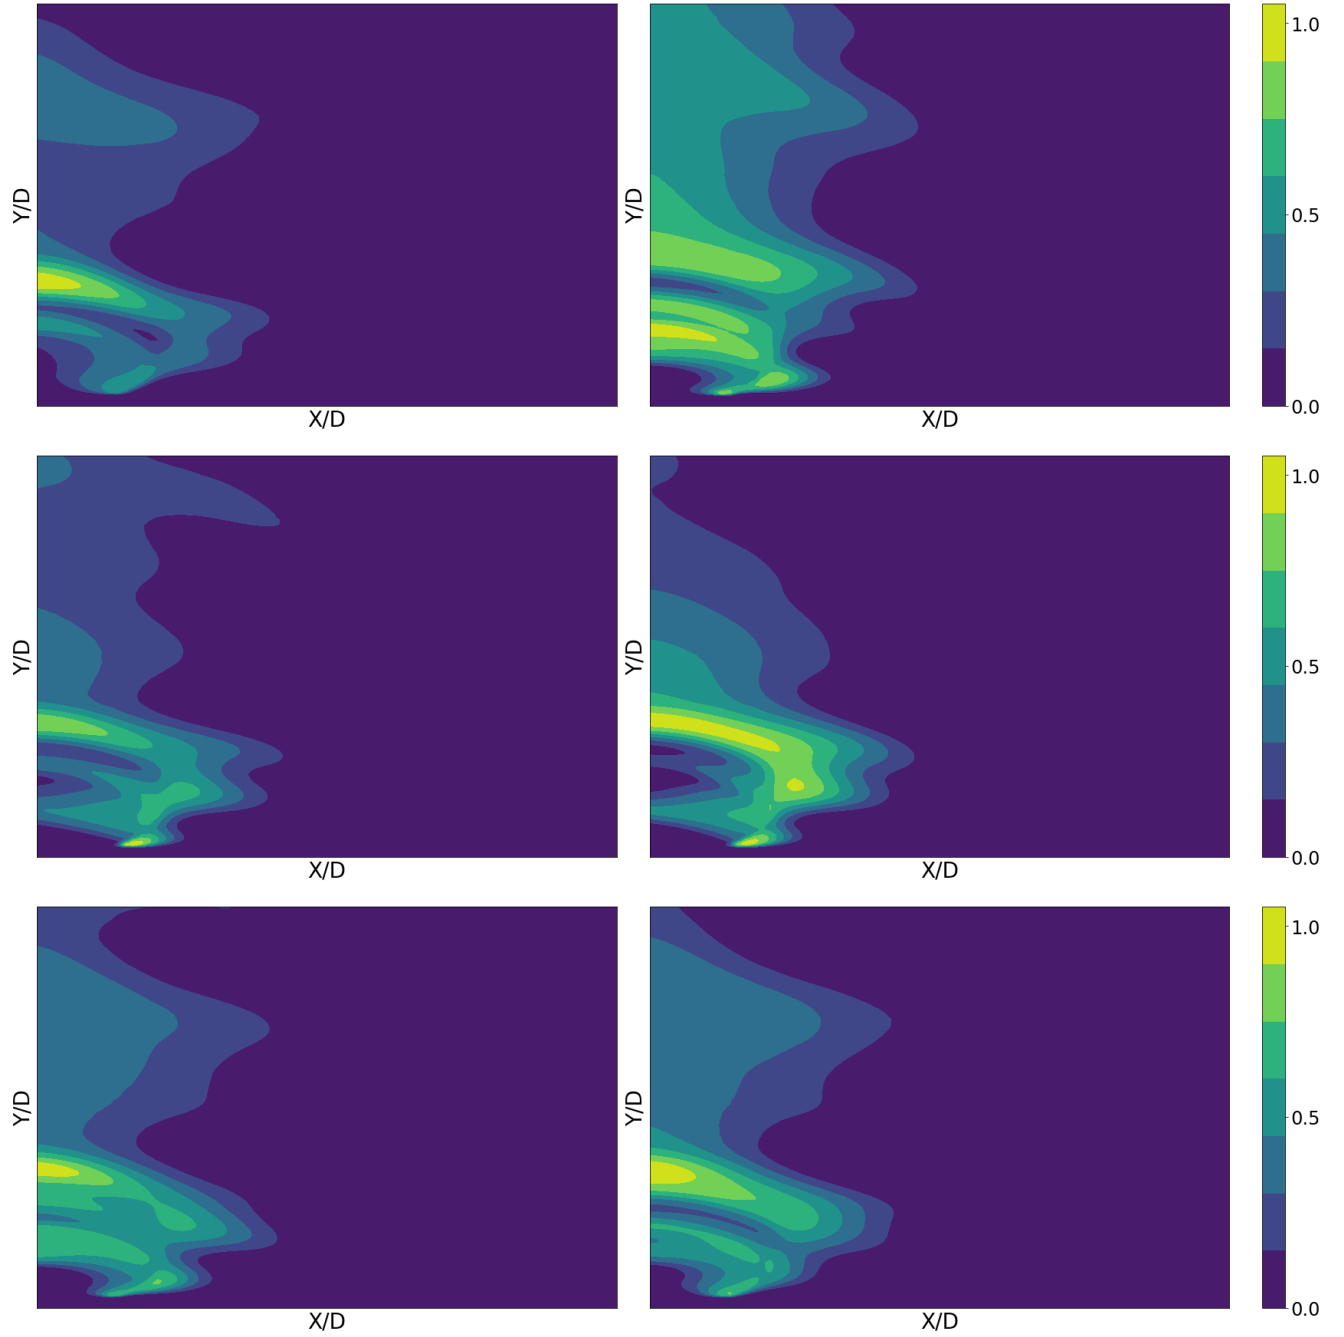

The normalized first five weighted 2D Proper Orthogonal Decomposition (POD) spatial modes, comparing lcSVD optimum sensors(left) with the ground truth (right) for the variable  $CO_2$  in the laminar co flow flame dataset. With 20\% of modes retained, the modes are arranged from top to bottom in order of decreasing energy.

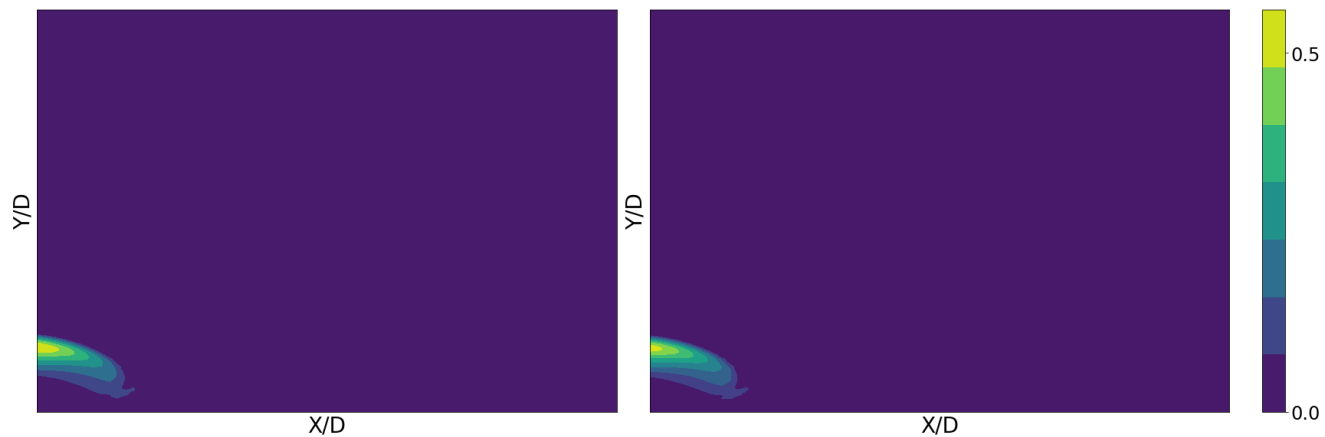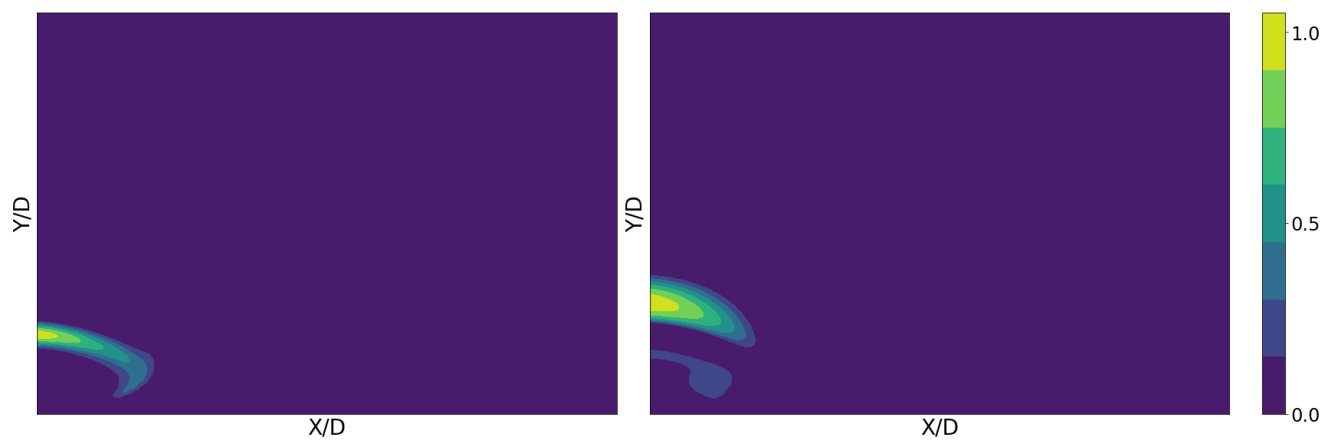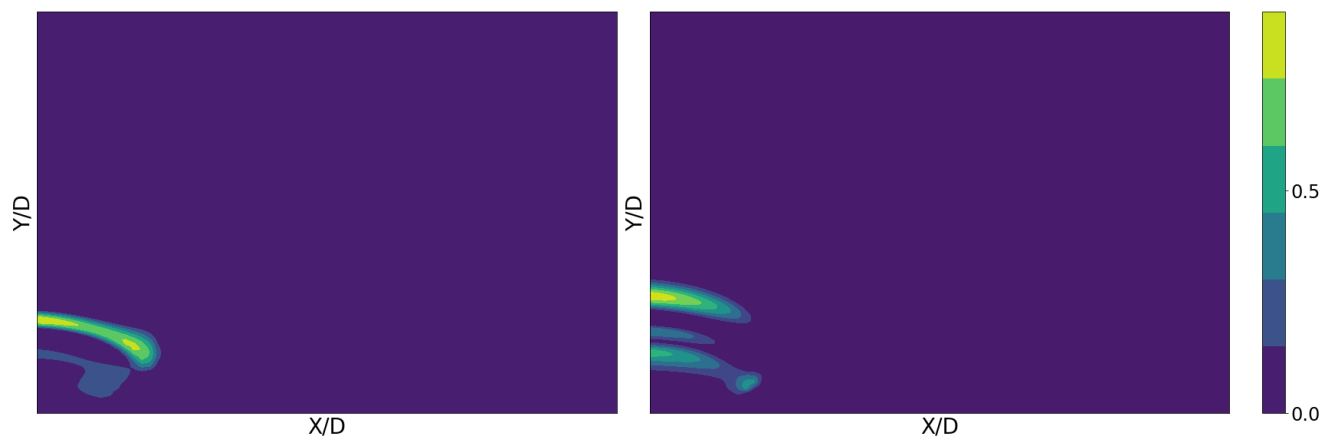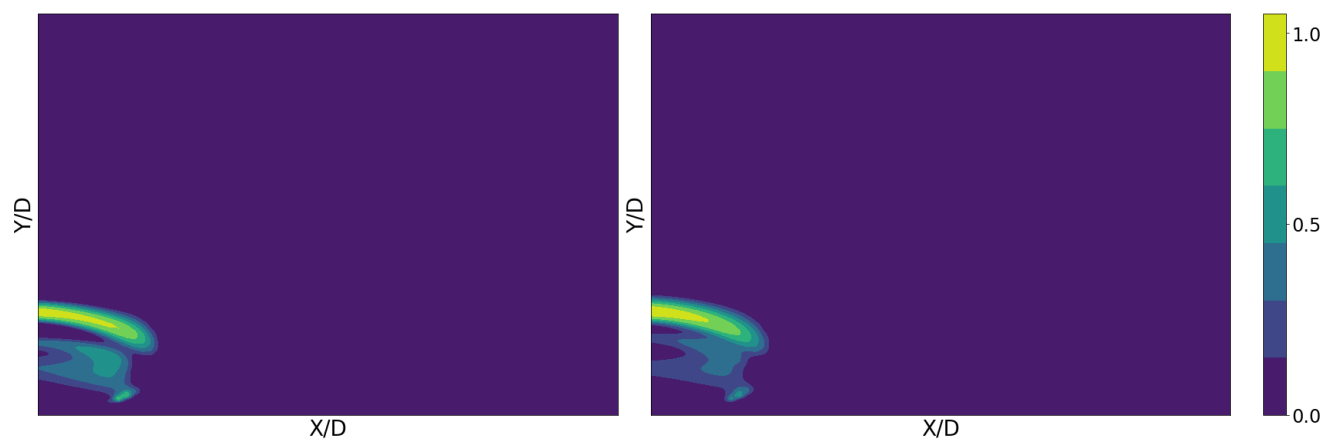

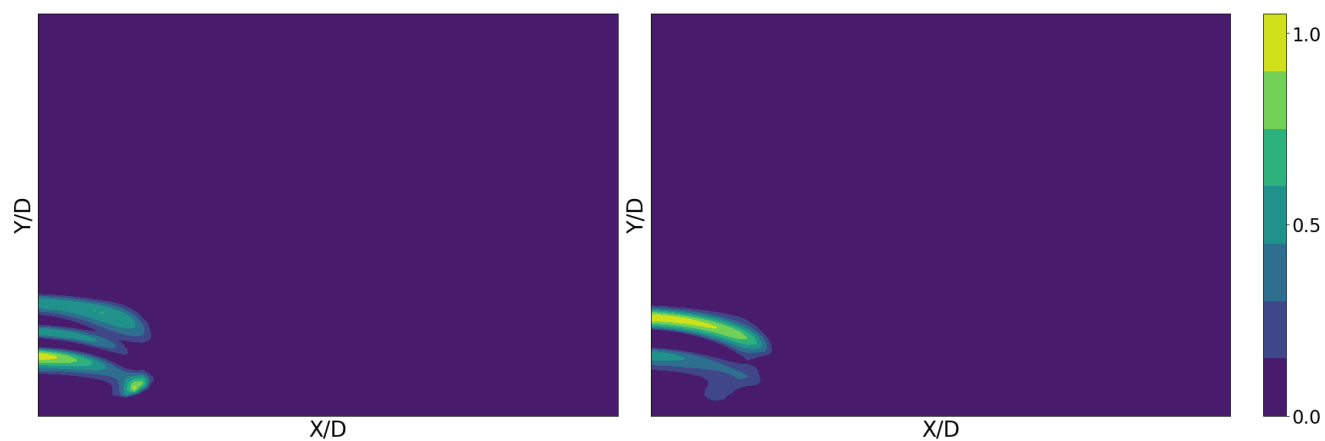

The normalized first five weighted 2D Proper Orthogonal Decomposition (POD) spatial modes, comparing lcSVD optimum sensors(left) with the ground truth (right) for the variable  $C_2H_2$  in the laminar co flow flame dataset. With 20\% of modes retained, the modes are arranged from top to bottom in order of decreasing energy.

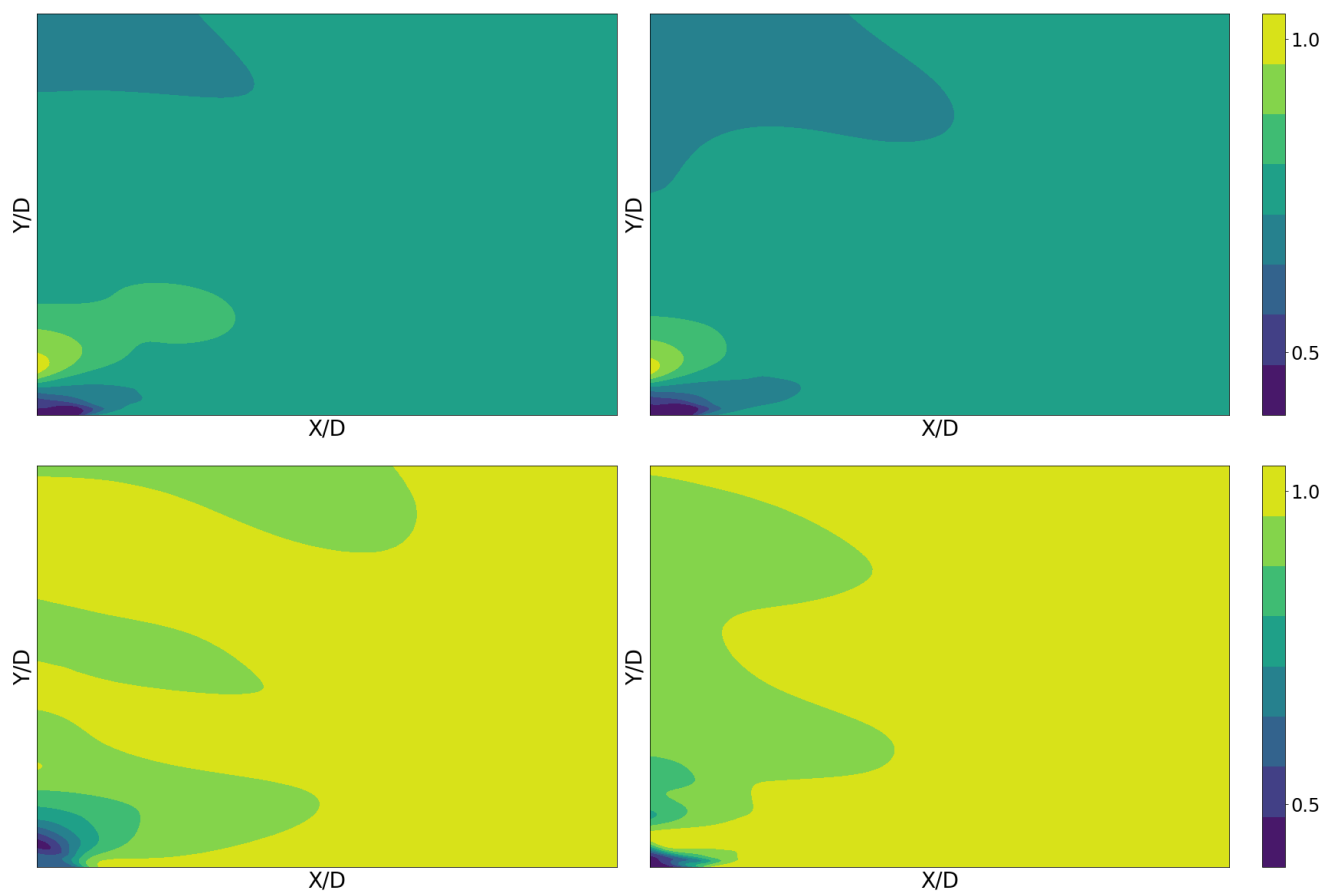

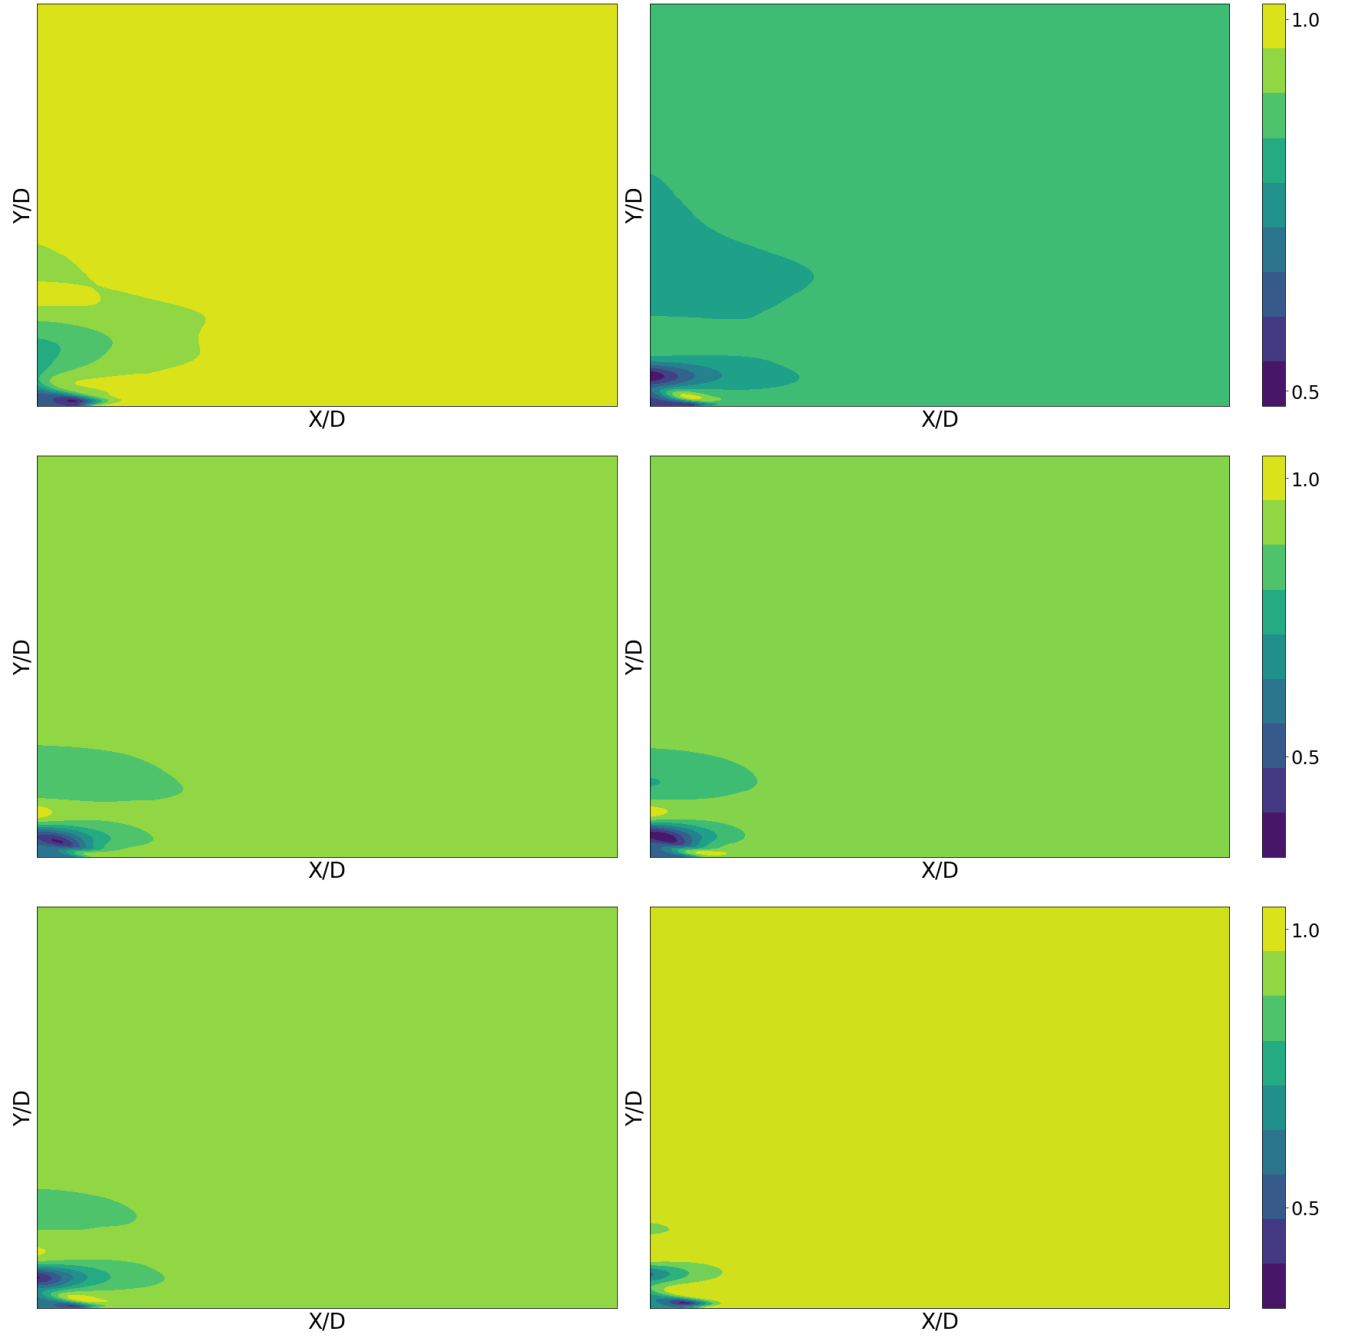

The normalized first five weighted 2D Proper Orthogonal Decomposition (POD) spatial modes, comparing lcSVD optimum sensors(left) with the ground truth (right) for the variable  $N_2$  in the laminar co flow flame dataset. With 20% of modes retained, the modes are arranged from top to bottom in order of decreasing energy.

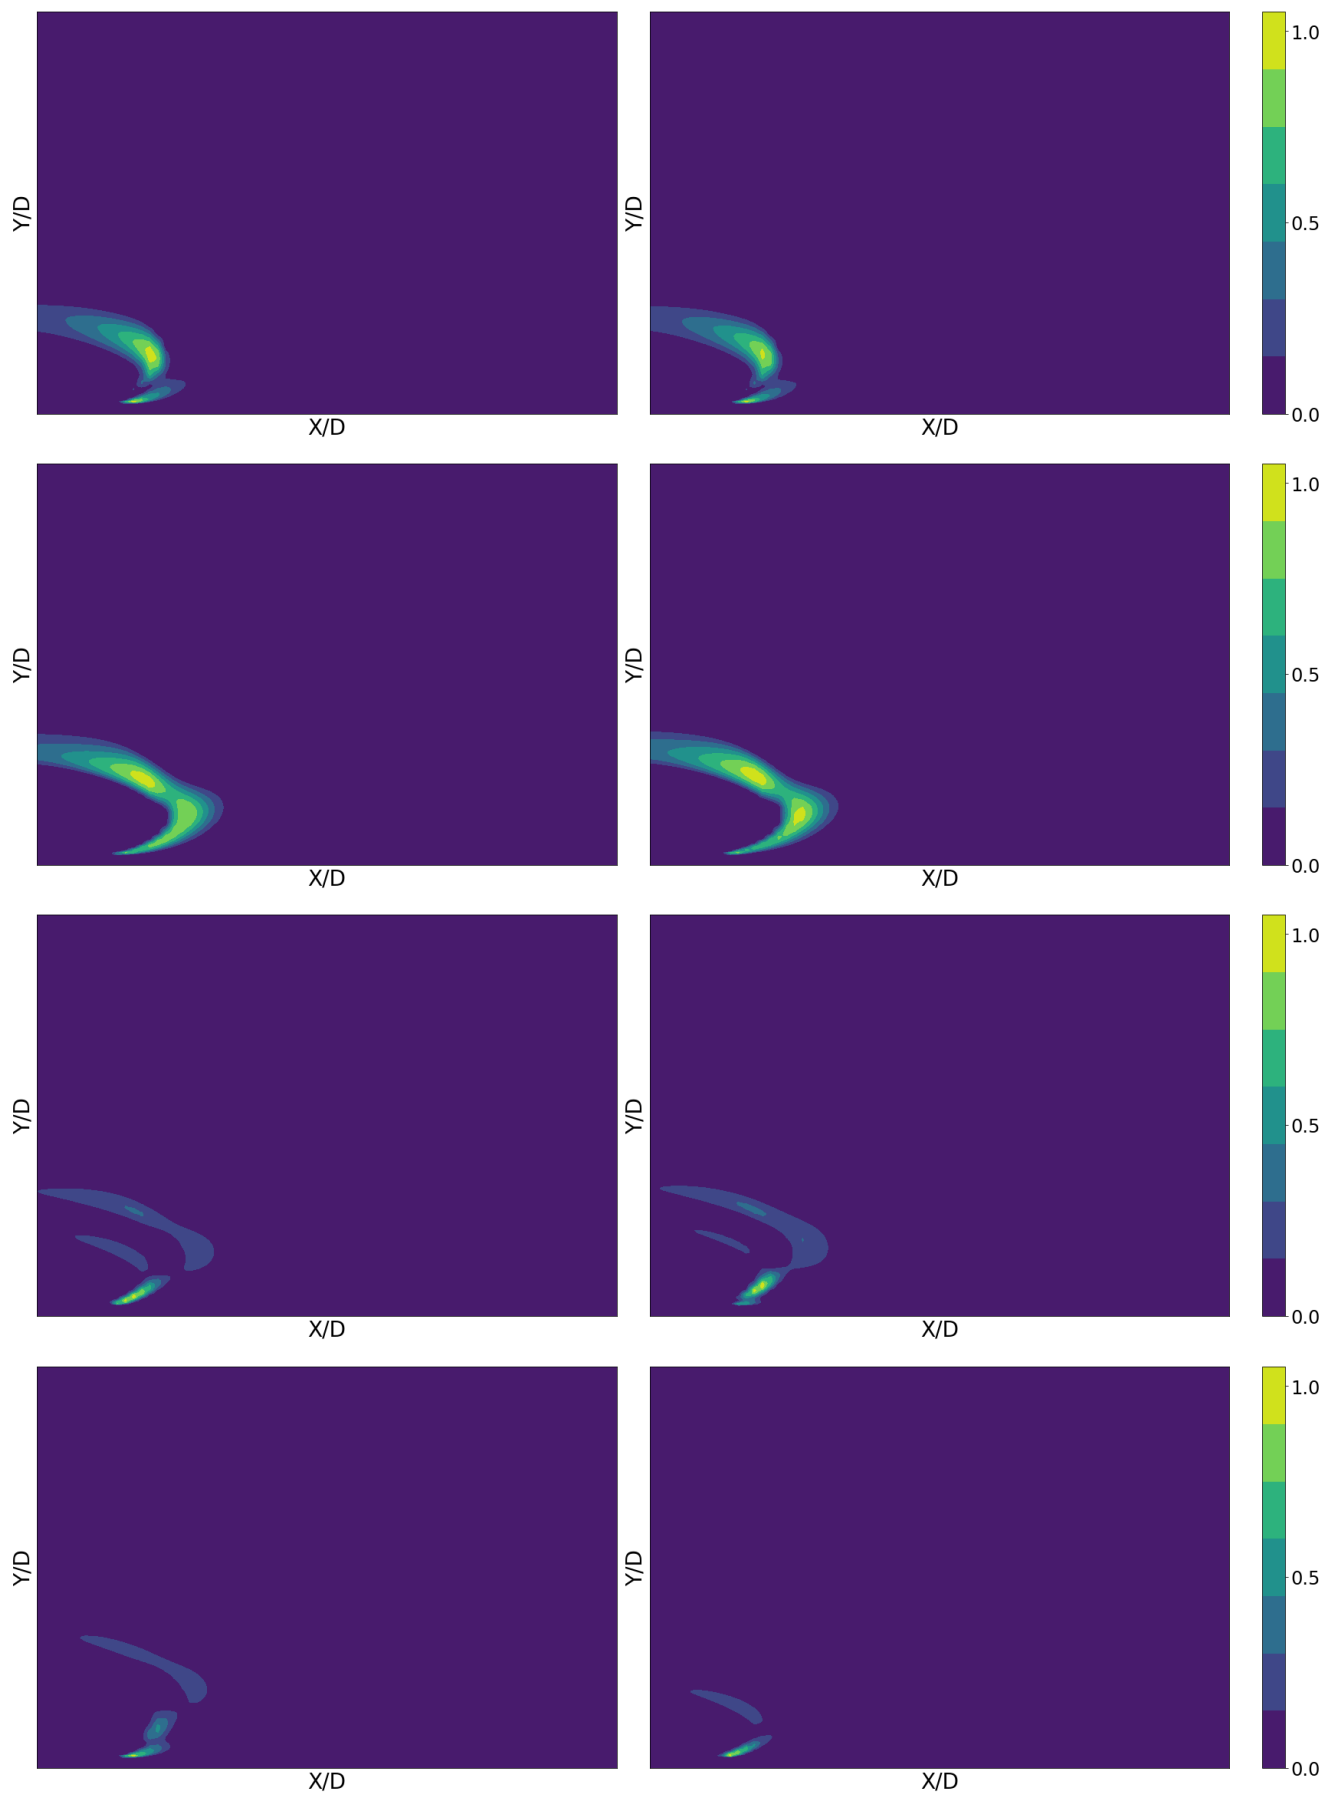

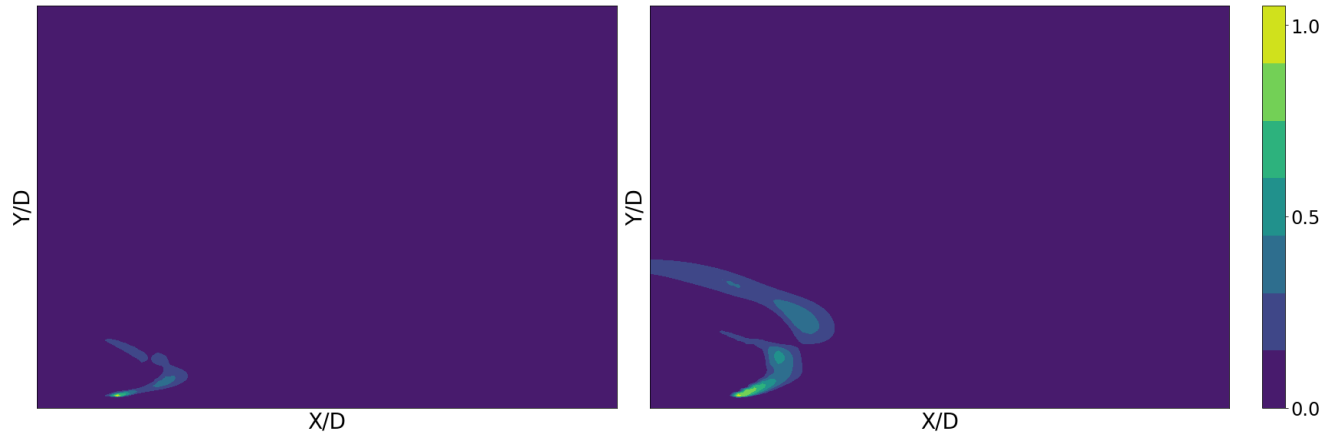

The normalized first five weighted 2D Proper Orthogonal Decomposition (POD) spatial modes, comparing lcSVD equally spaced samples(left) with the ground truth (right) for the variable  $O$  in the laminar co flow flame dataset. With 20\% of modes retained, the modes are arranged from top to bottom in order of decreasing energy.

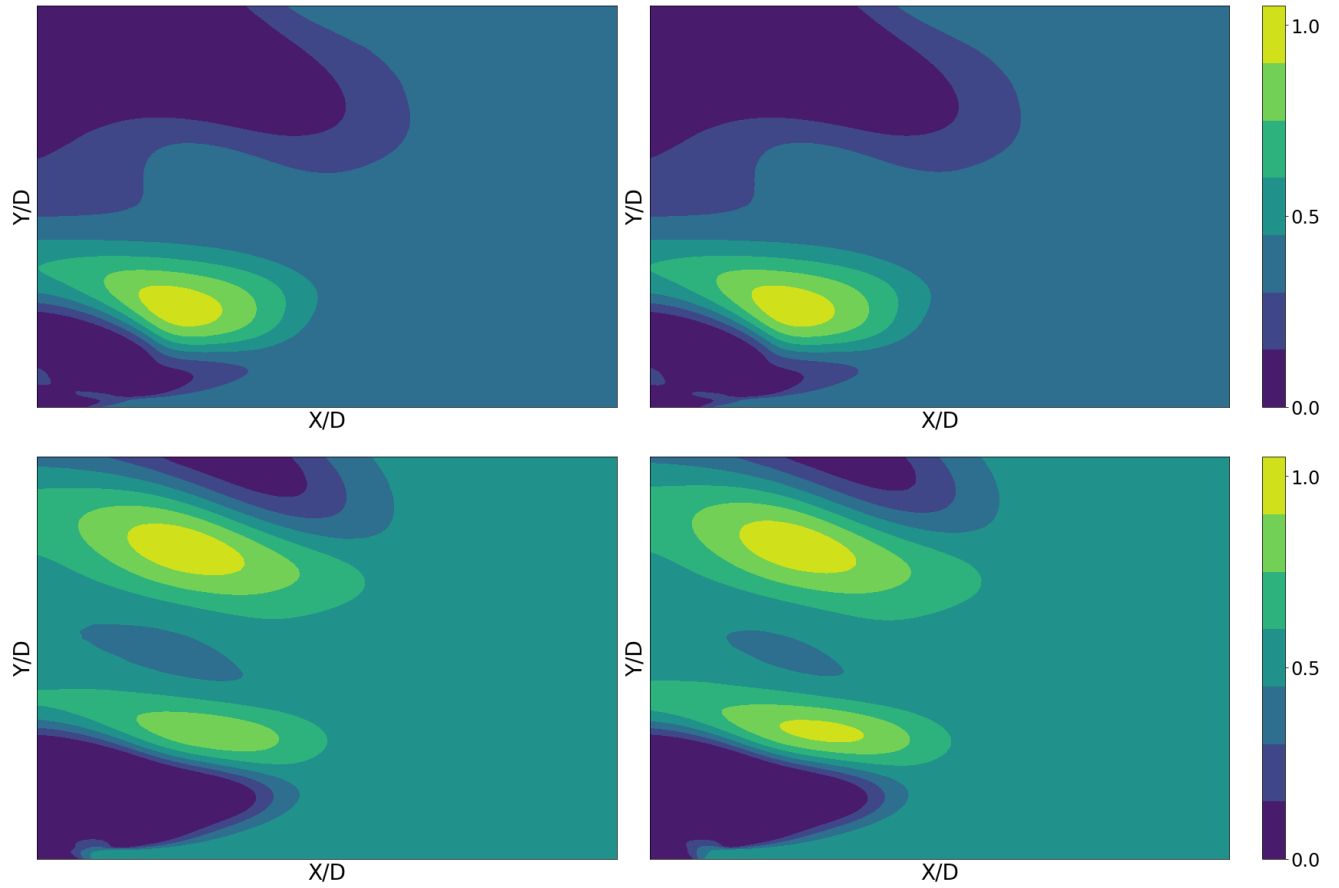

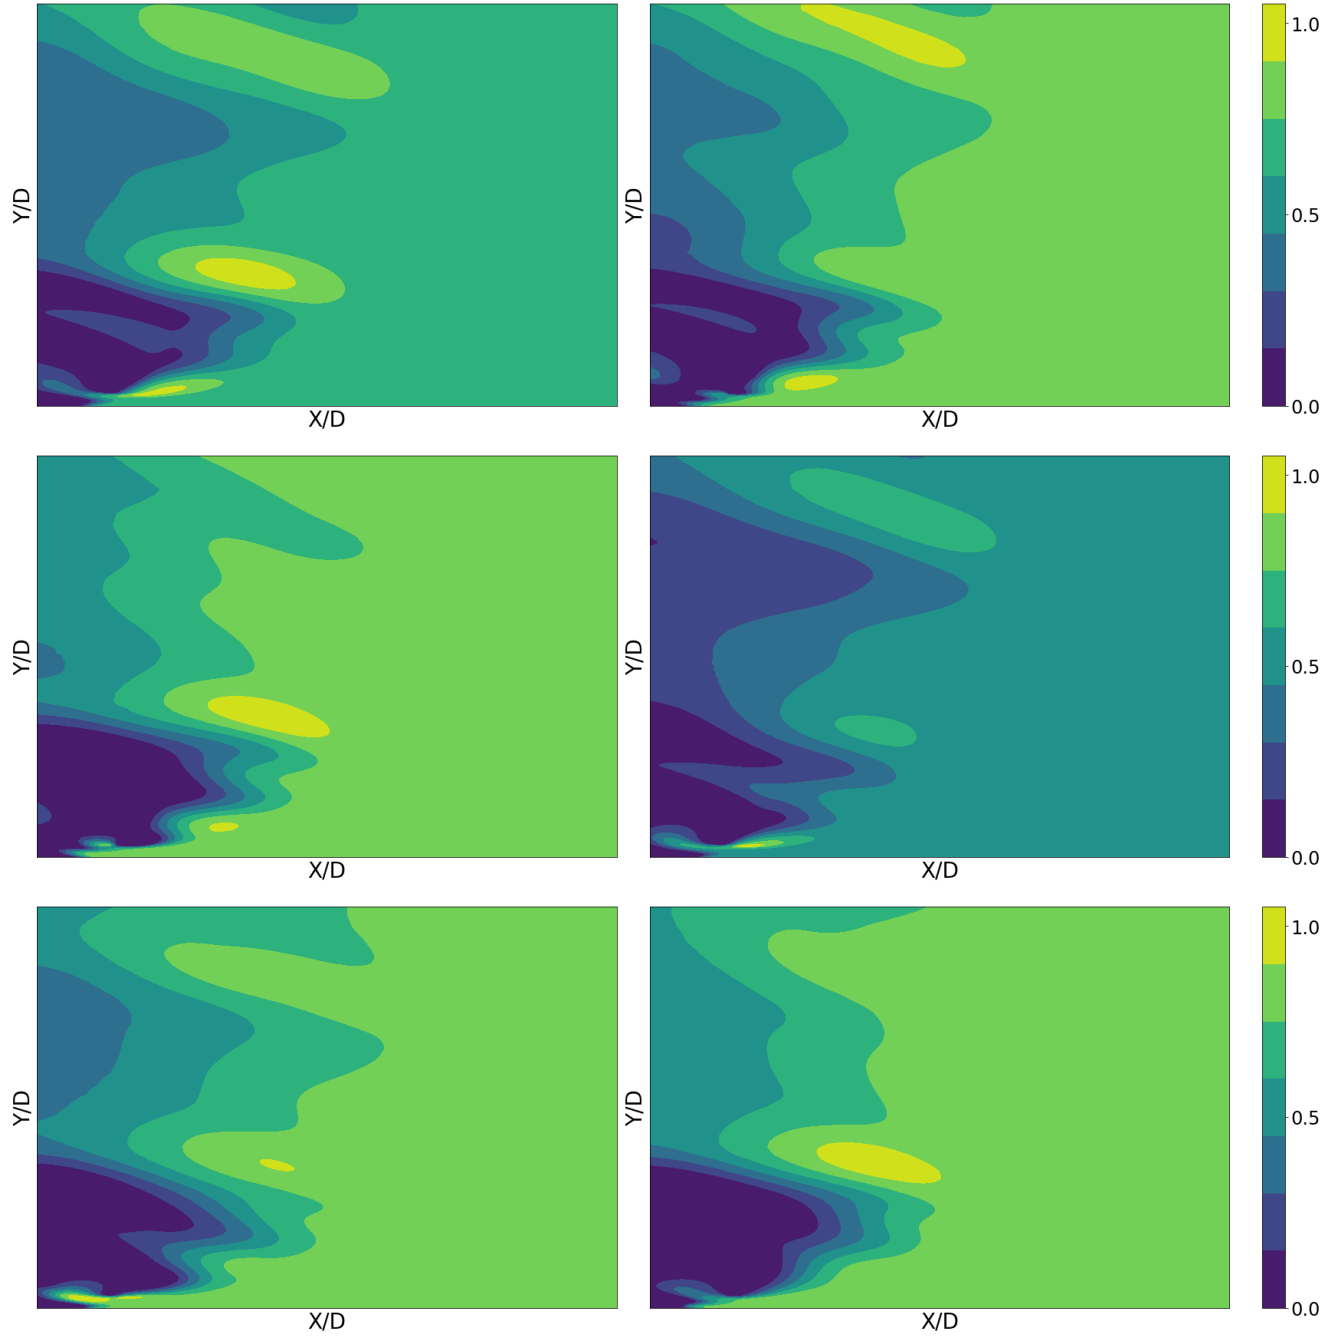

The normalized first five weighted 2D Proper Orthogonal Decomposition (POD) spatial modes, comparing lcSVD equally spaced samples(left) with the ground truth (right) for the variable  $O_2$  in the laminar co flow flame dataset. With 20\% of modes retained, the modes are arranged from top to bottom in order of decreasing energy.

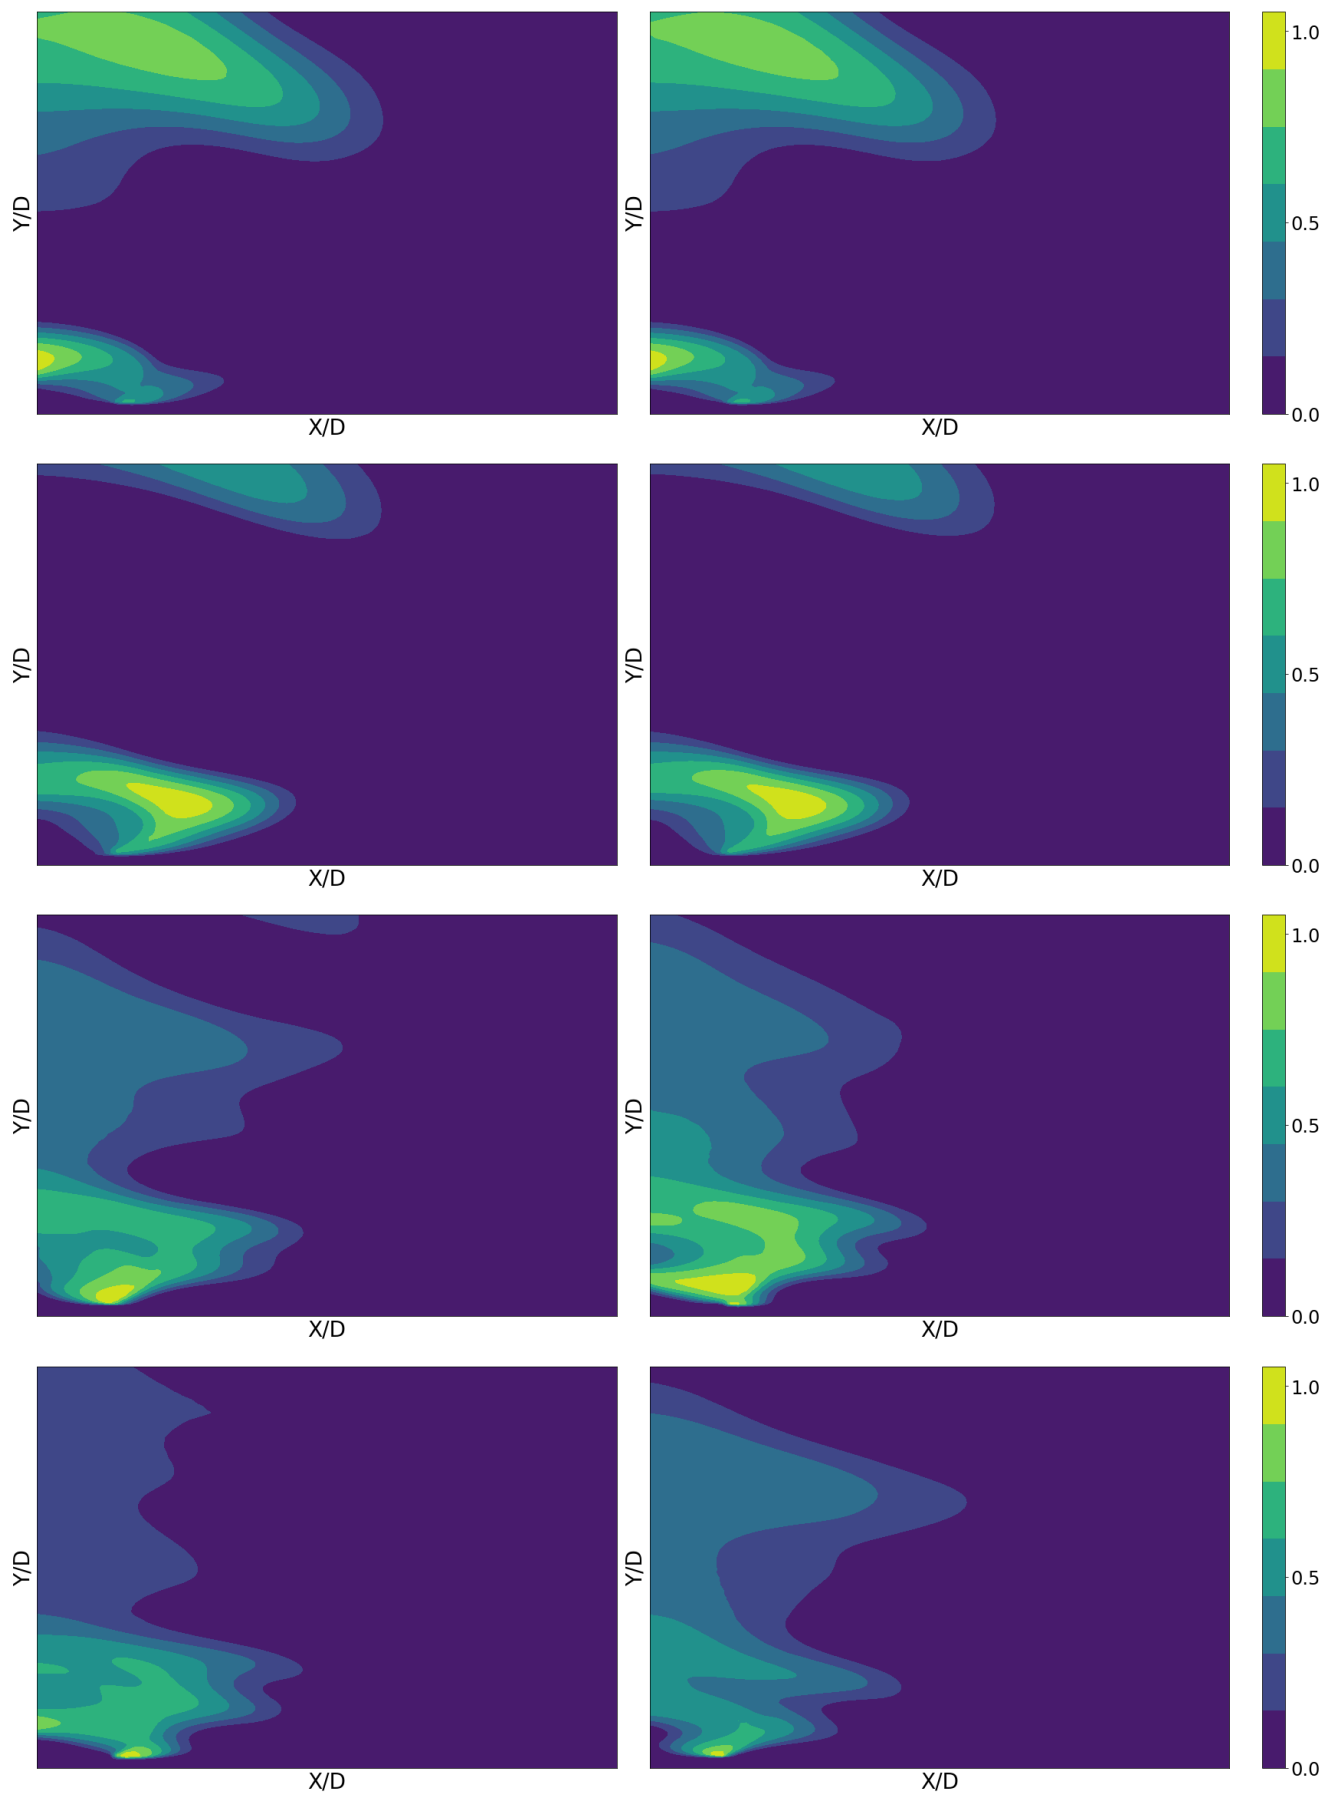

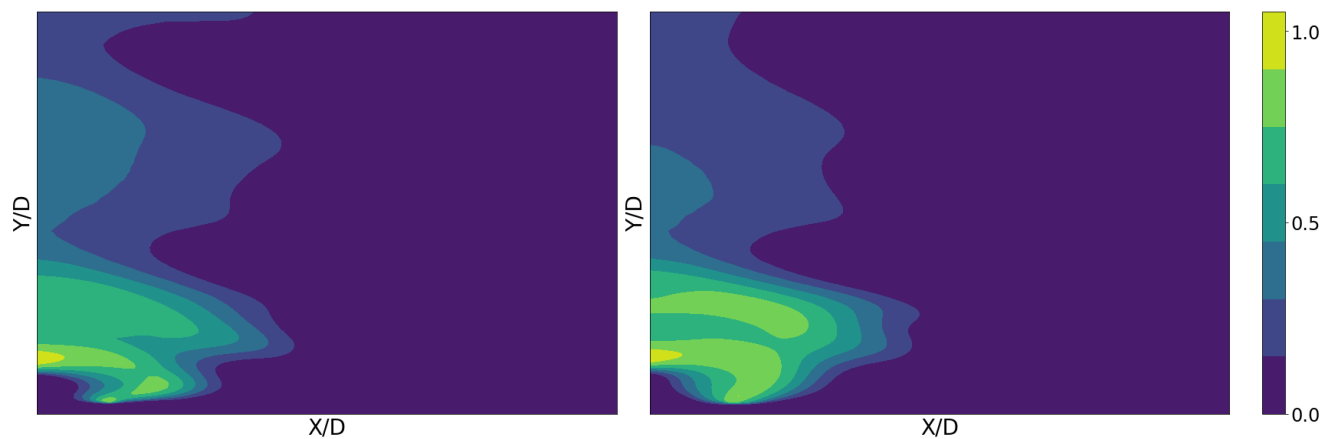

The normalized first five weighted 2D Proper Orthogonal Decomposition (POD) spatial modes, comparing lcSVD equally spaced samples(left) with the ground truth (right) for the variable  $H_2O$  in the laminar co flow flame dataset. With 20\% of modes retained, the modes are arranged from top to bottom in order of decreasing energy.

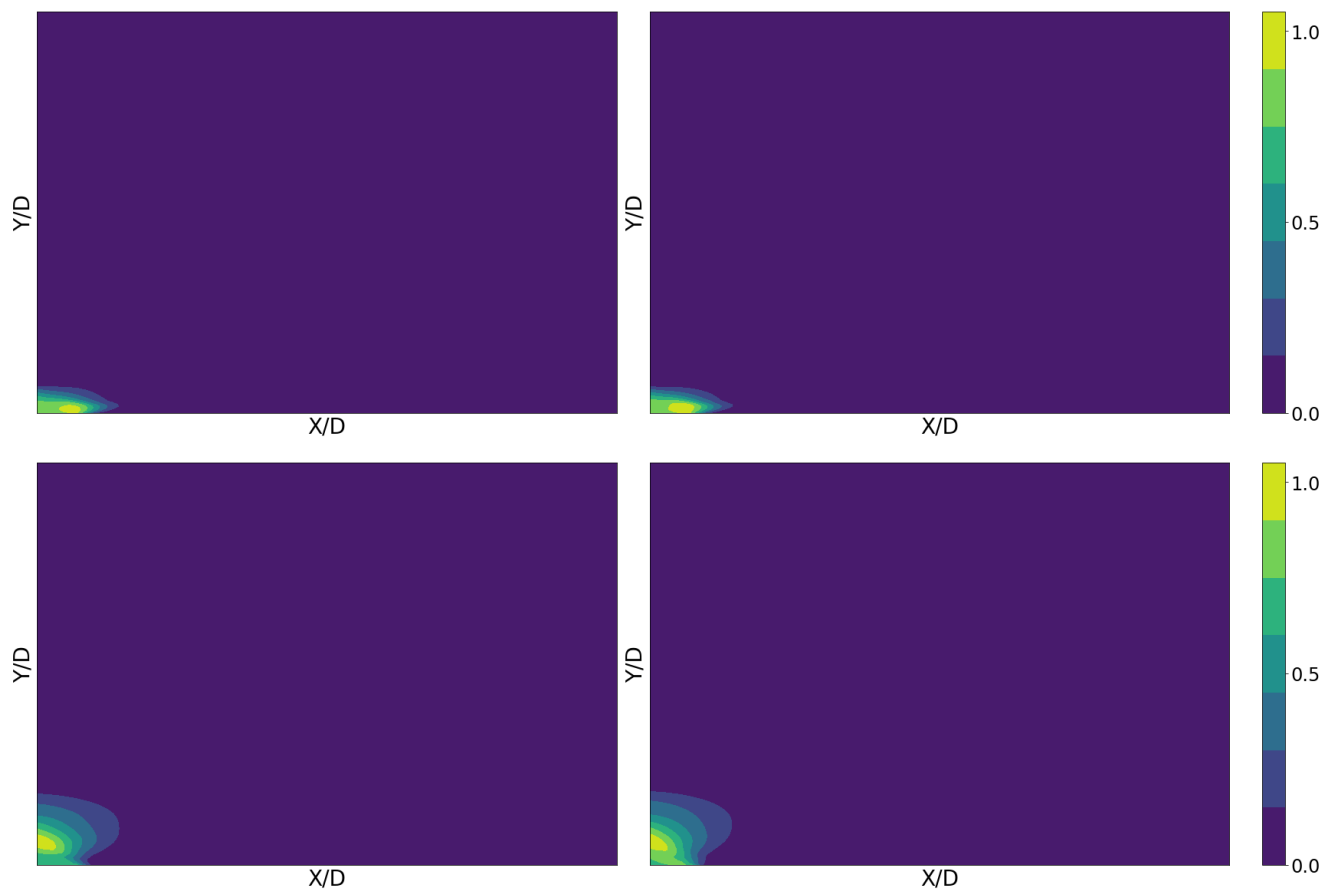

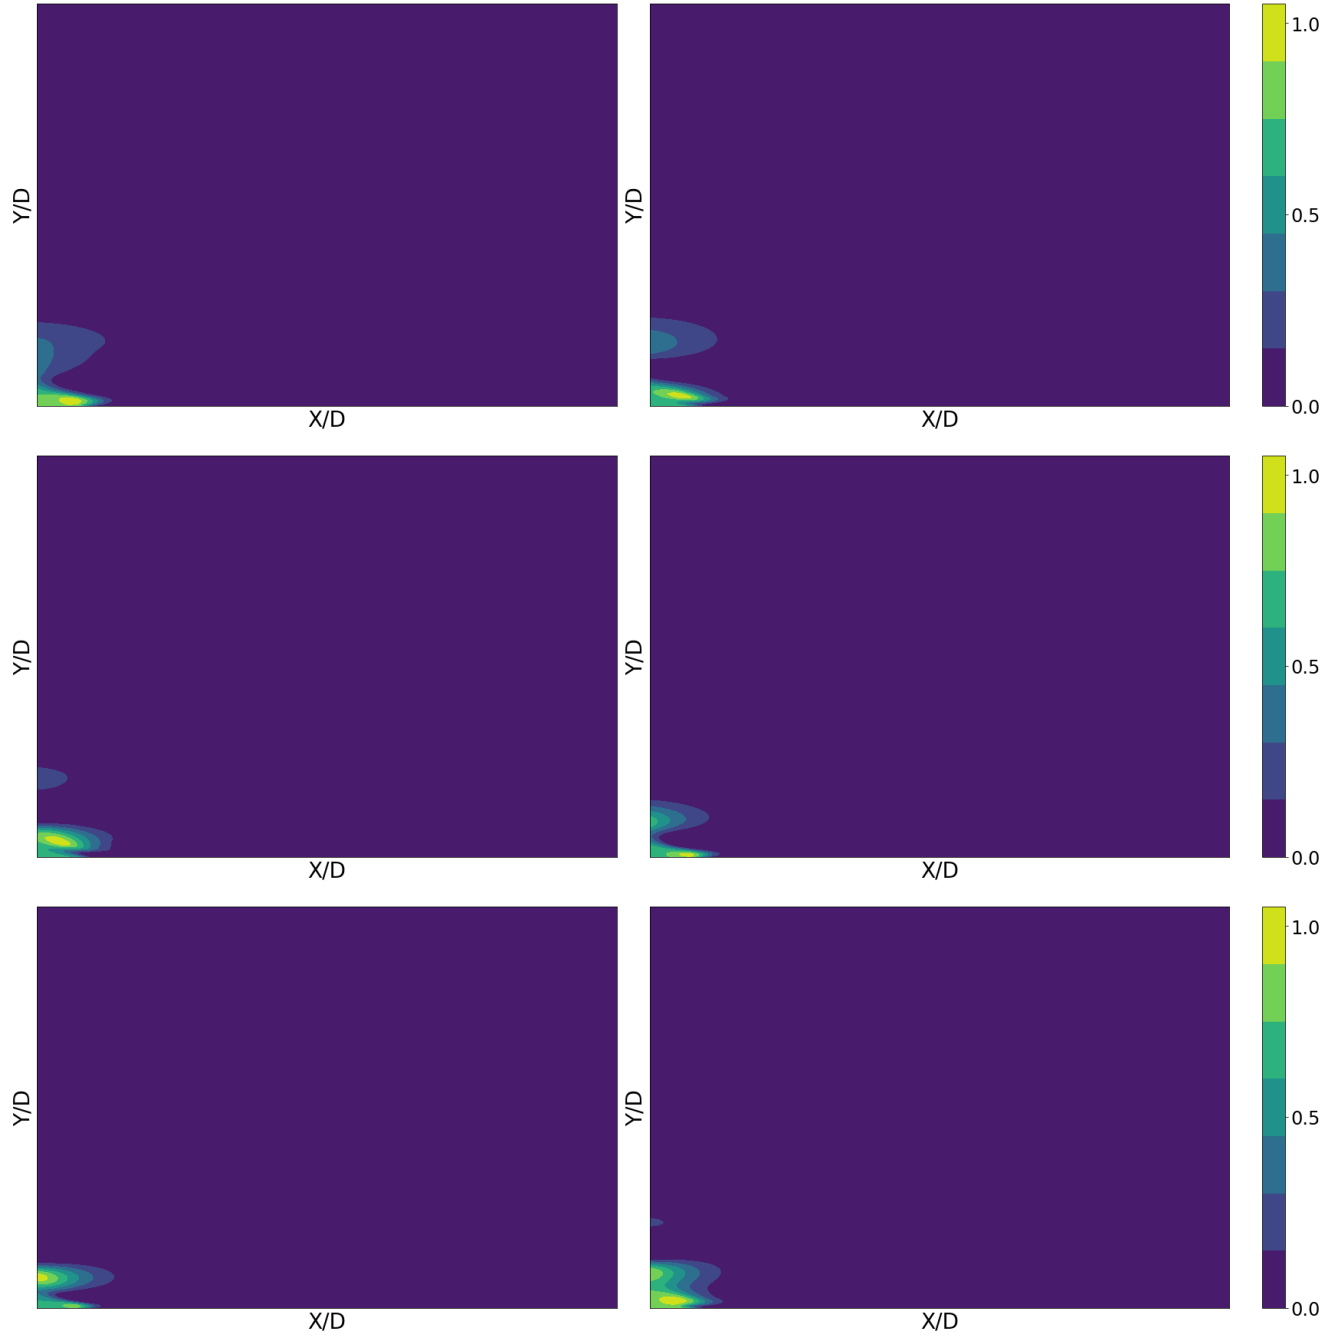

The normalized first five weighted 2D Proper Orthogonal Decomposition (POD) spatial modes, comparing lcSVD equally spaced samples(left) with the ground truth (right) for the variable  $CH_4$  in the laminar co flow flame dataset. With 20\% of modes retained, the modes are arranged from top to bottom in order of decreasing energy.

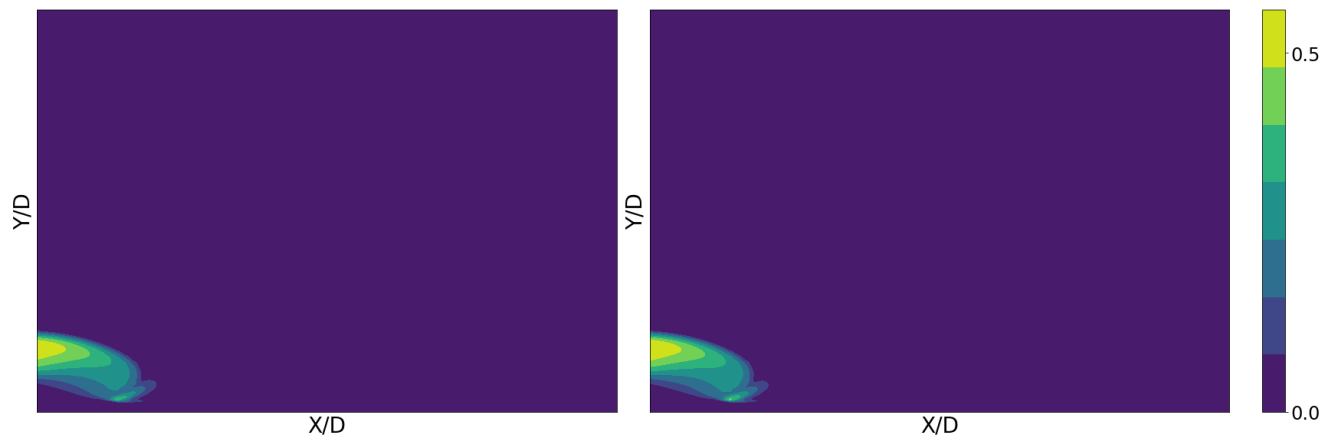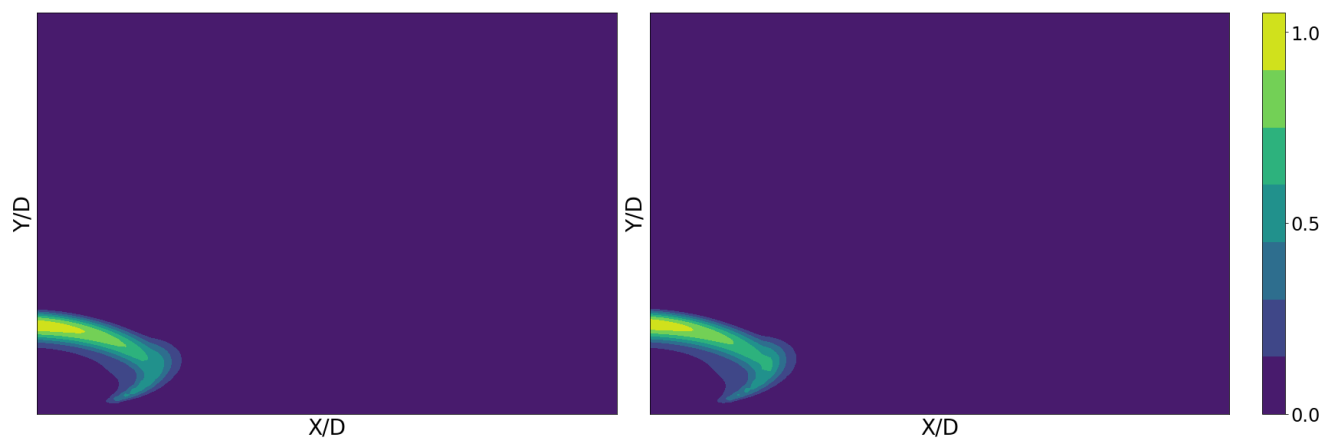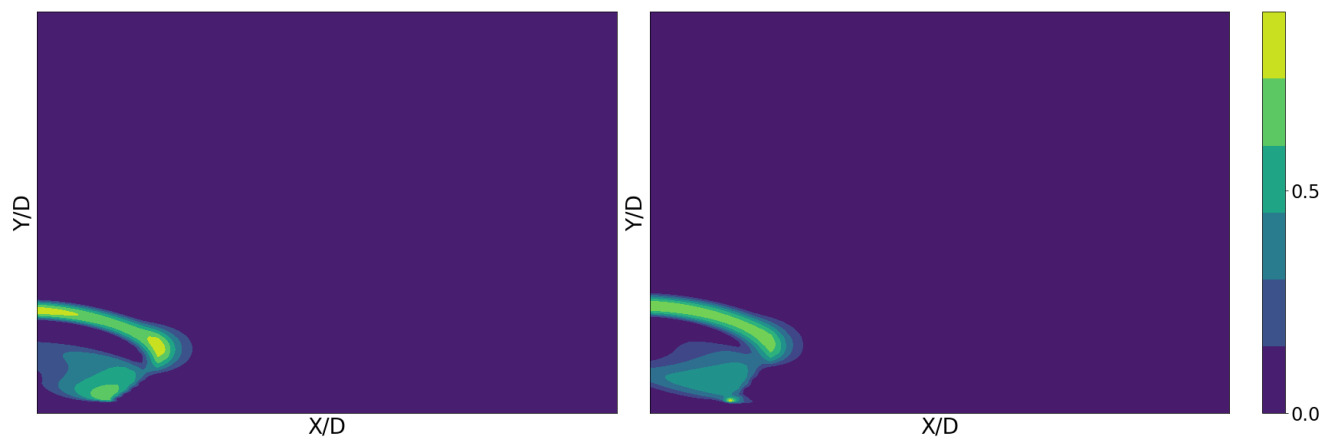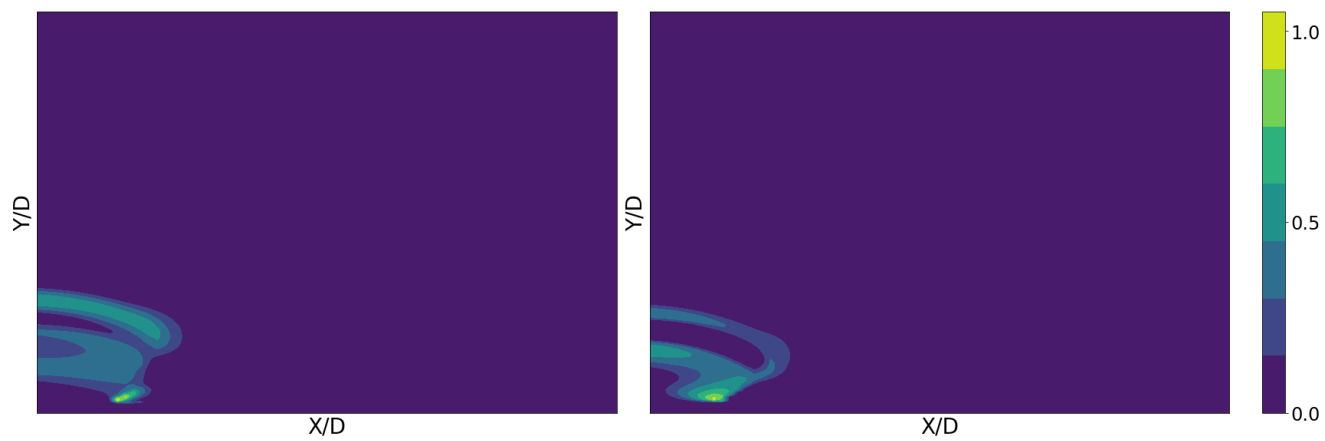

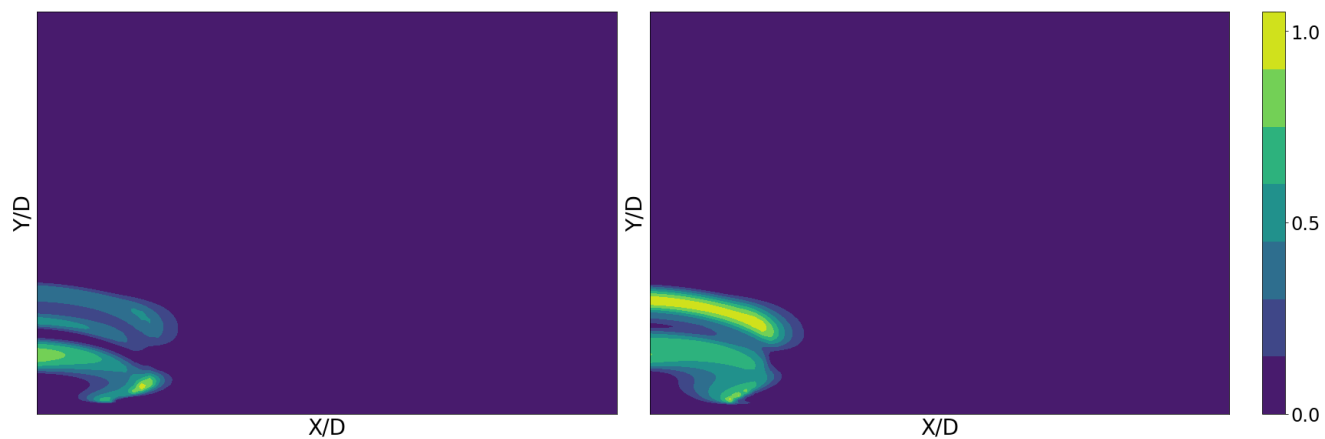

The normalized first five weighted 2D Proper Orthogonal Decomposition (POD) spatial modes, comparing lcSVD equally spaced samples(left) with the ground truth (right) for the variable  $CO$  in the laminar co flow flame dataset. With 20\% of modes retained, the modes are arranged from top to bottom in order of decreasing energy.

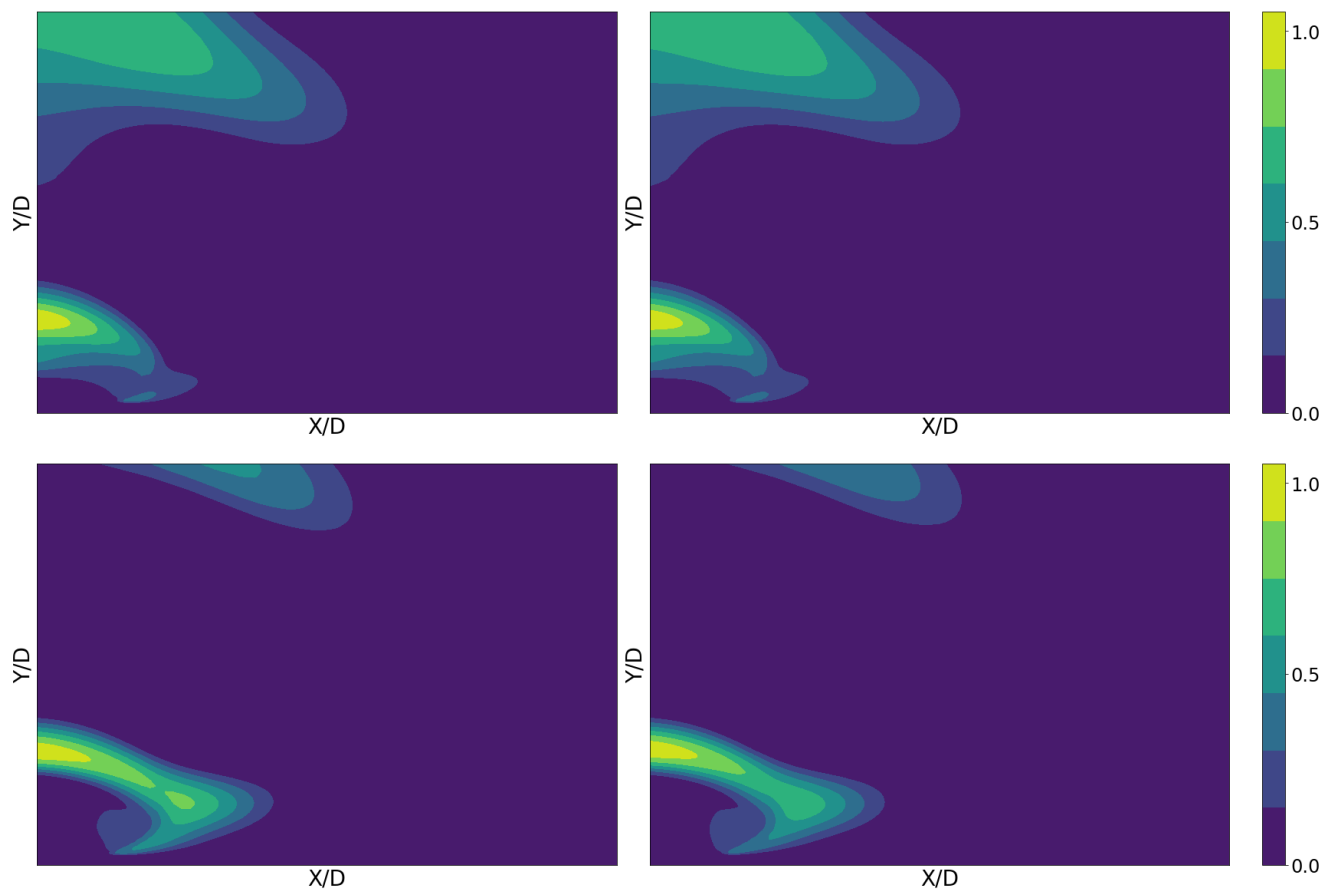

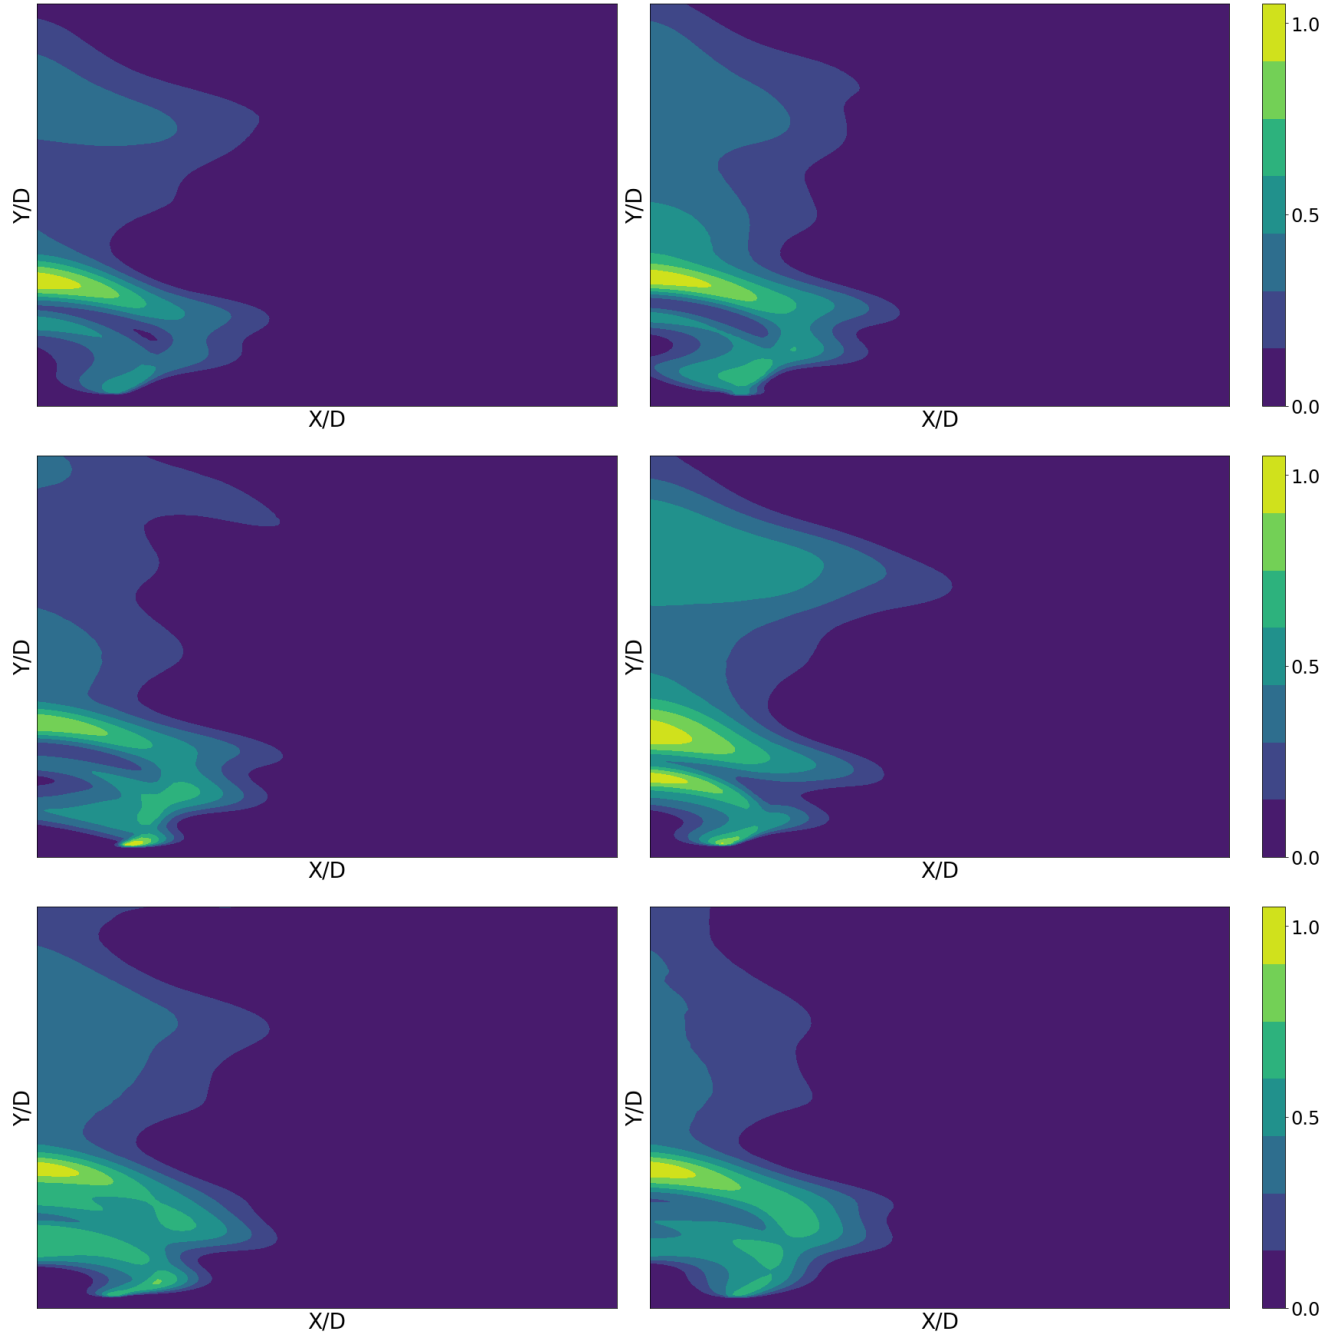

The normalized first five weighted 2D Proper Orthogonal Decomposition (POD) spatial modes, comparing lcSVD equally spaced samples(left) with the ground truth (right) for the variable  $CO_2$  in the laminar co flow flame dataset. With 20\% of modes retained, the modes are arranged from top to bottom in order of decreasing energy.

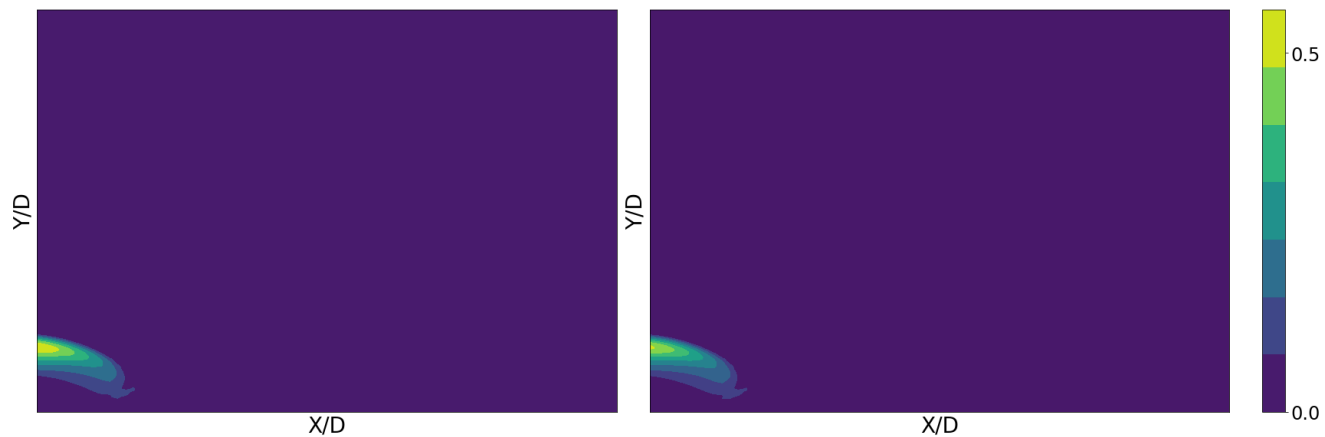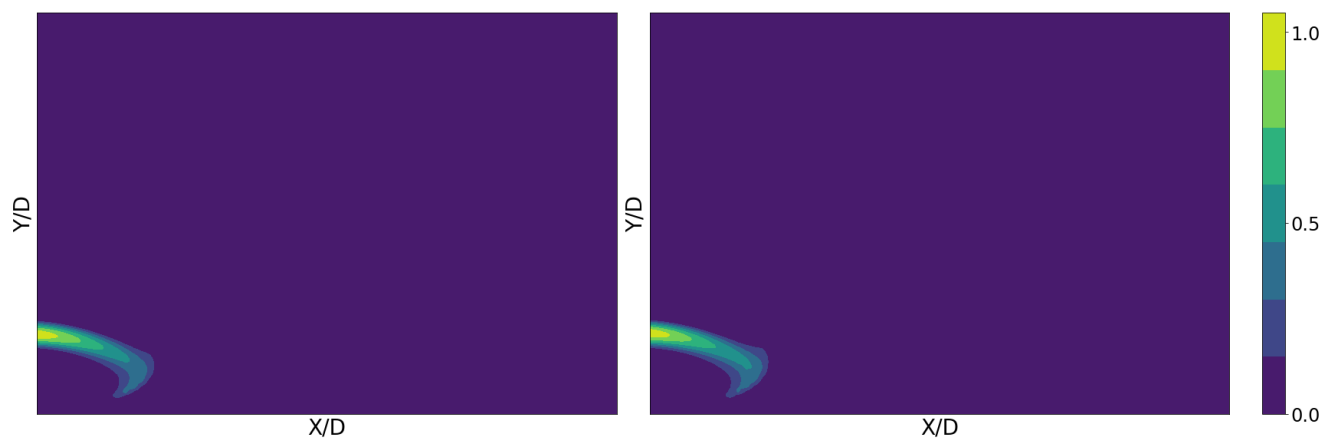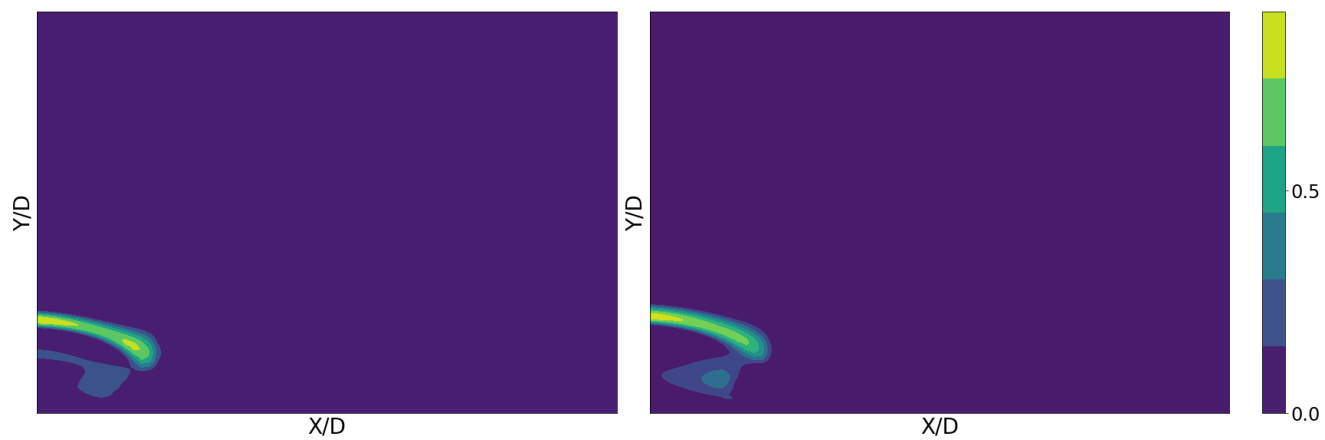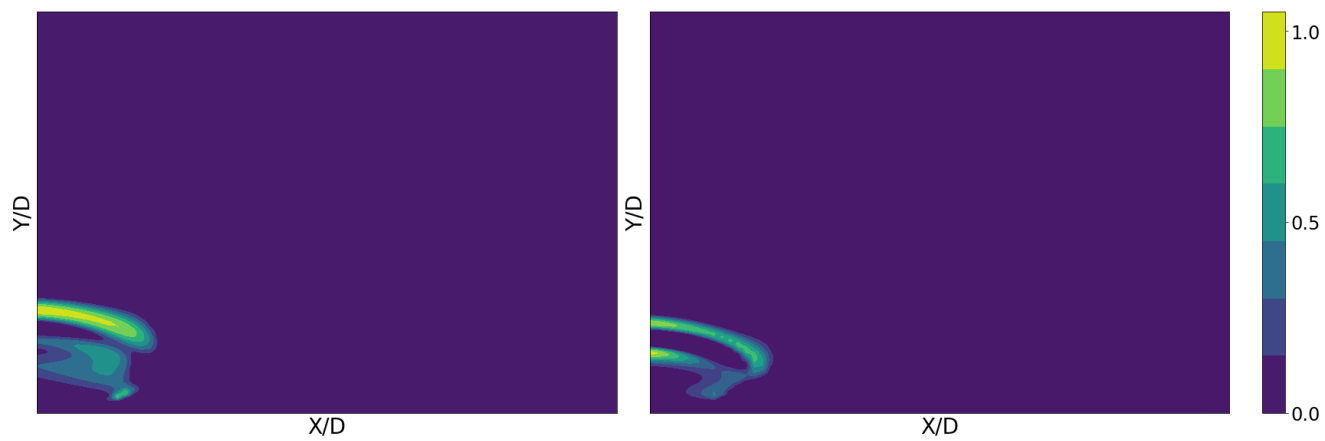

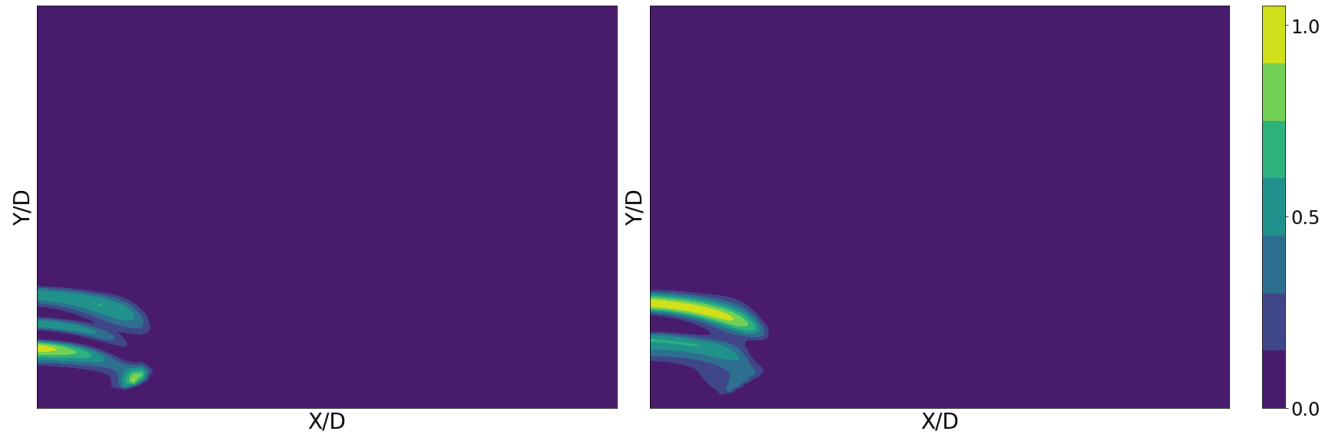

The normalized first five weighted 2D Proper Orthogonal Decomposition (POD) spatial modes, comparing lcSVD equally spaced samples(left) with the ground truth (right) for the variable  $C_2H_2$  in the laminar co flow flame dataset. With 20\% of modes retained, the modes are arranged from top to bottom in order of decreasing energy.

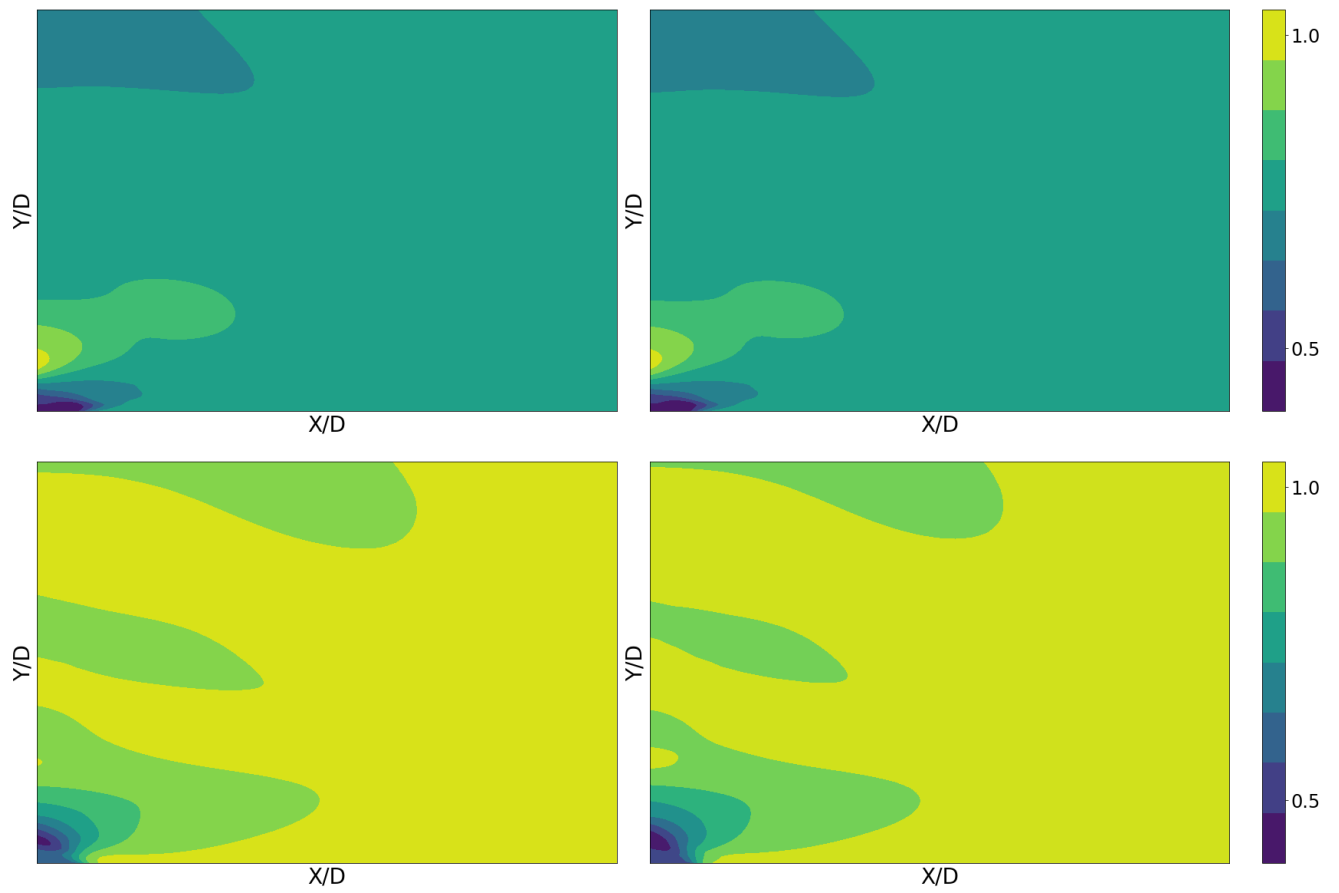

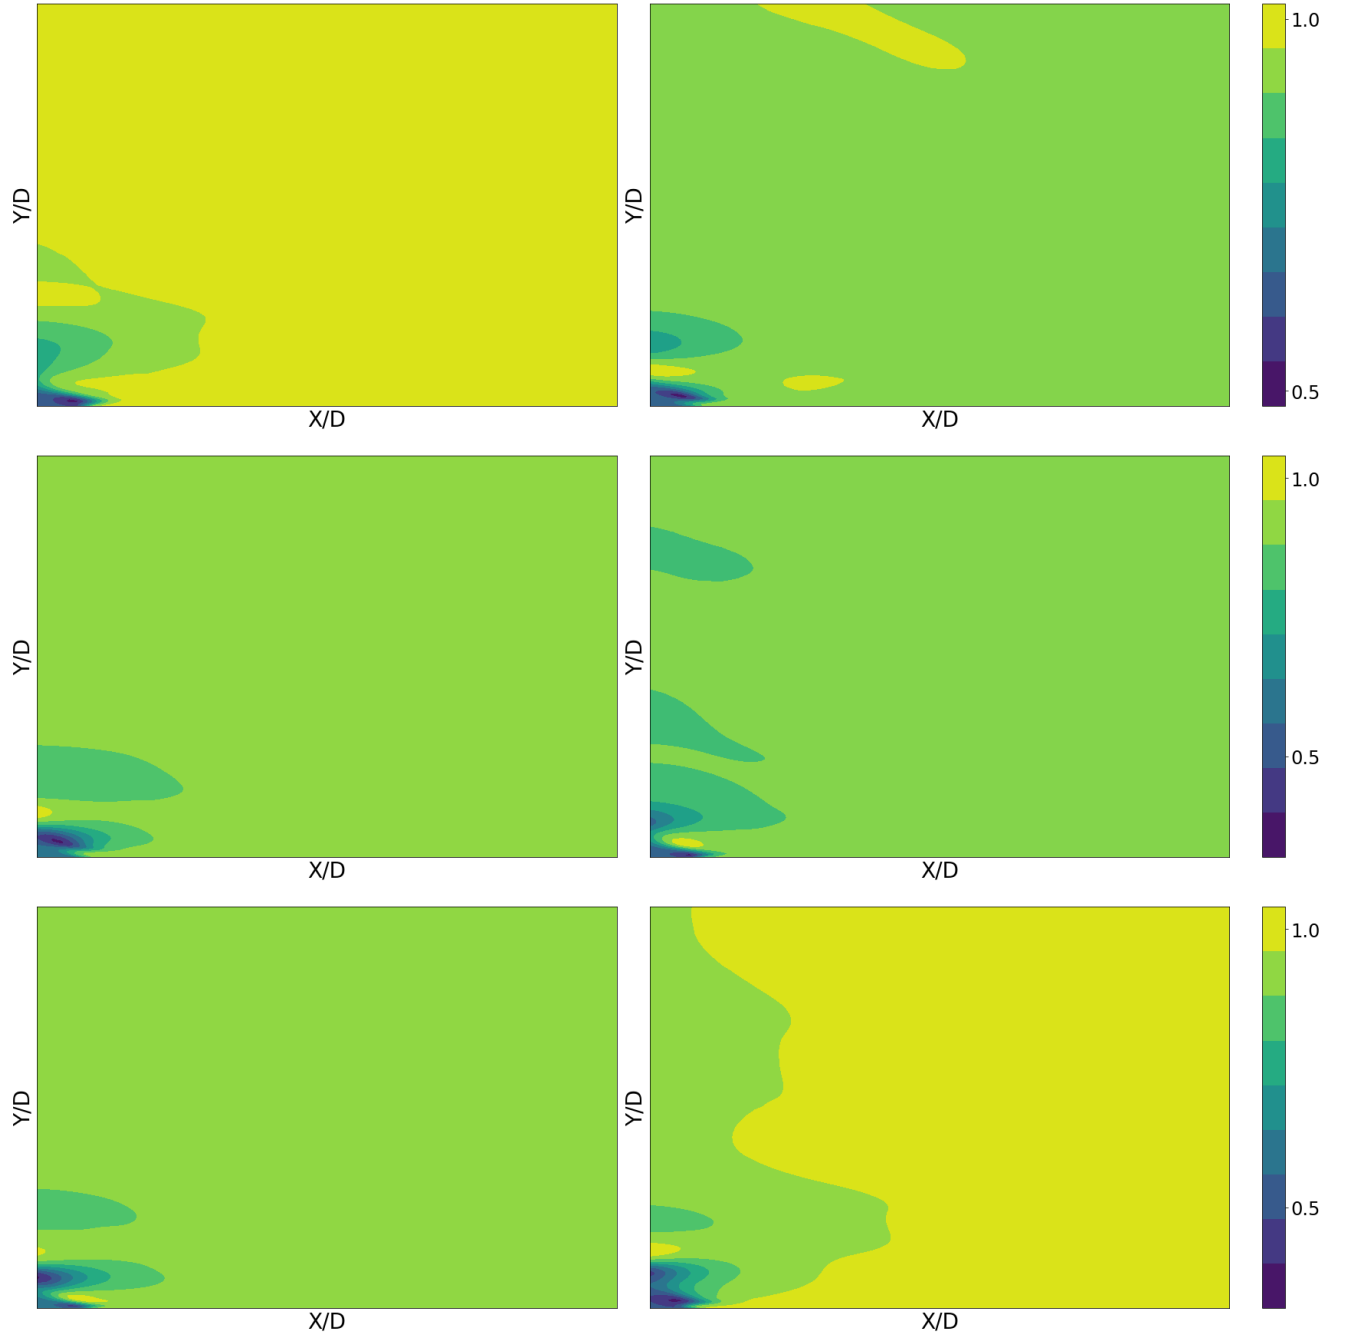

The normalized first five weighted 2D Proper Orthogonal Decomposition (POD) spatial modes, comparing lcSVD equally spaced samples(left) with the ground truth (right) for the variable  $N_2$  in the laminar co flow flame dataset. With 20\% of modes retained, the modes are arranged from top to bottom in order of decreasing energy.

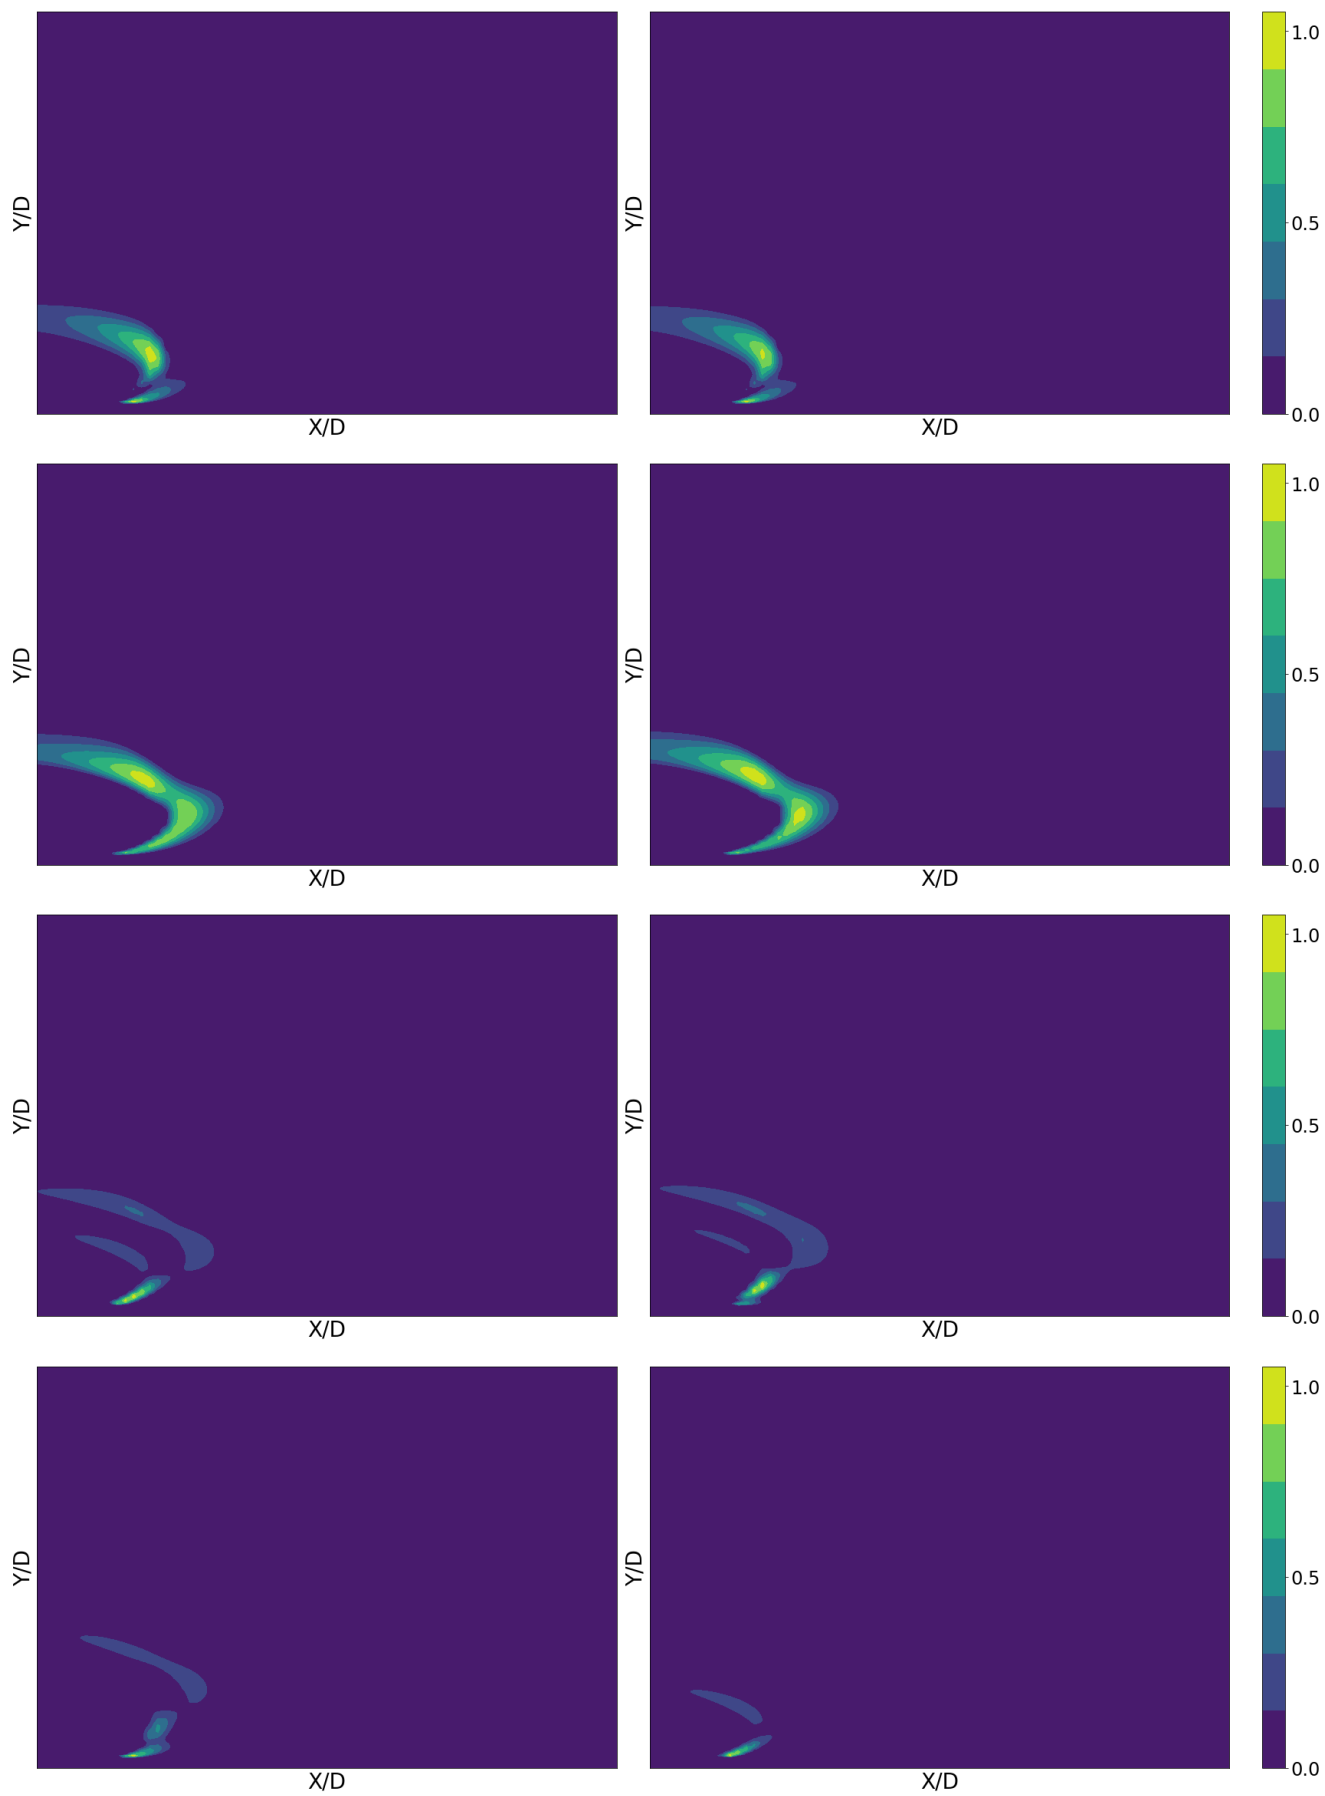

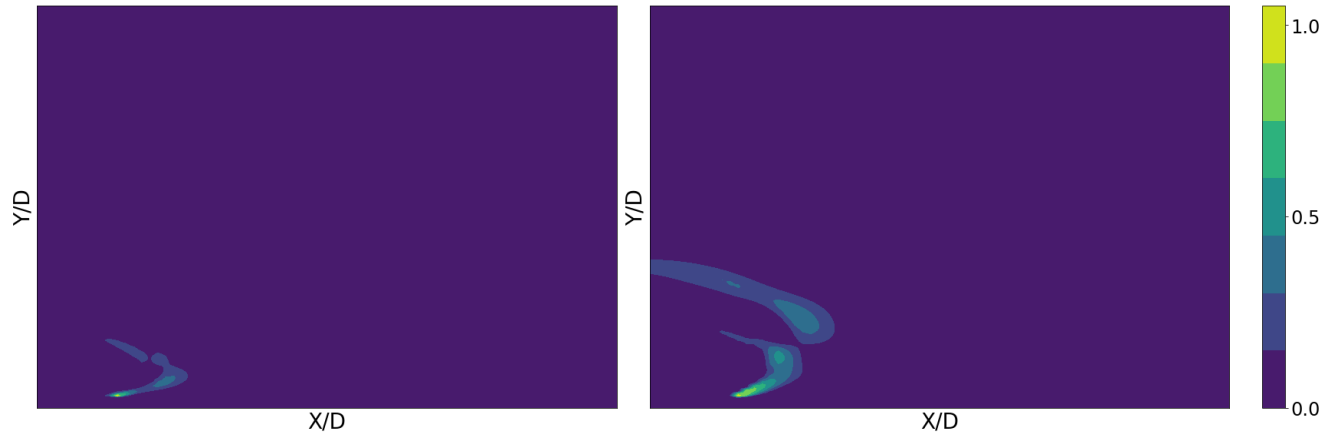

The normalized first five weighted 2D Proper Orthogonal Decomposition (POD) spatial modes, comparing lcSVD DA (left) with the ground truth (right) for the variable  $O$  in the laminar co flow flame dataset. With 20% of modes retained, the modes are arranged from top to bottom in order of decreasing energy.

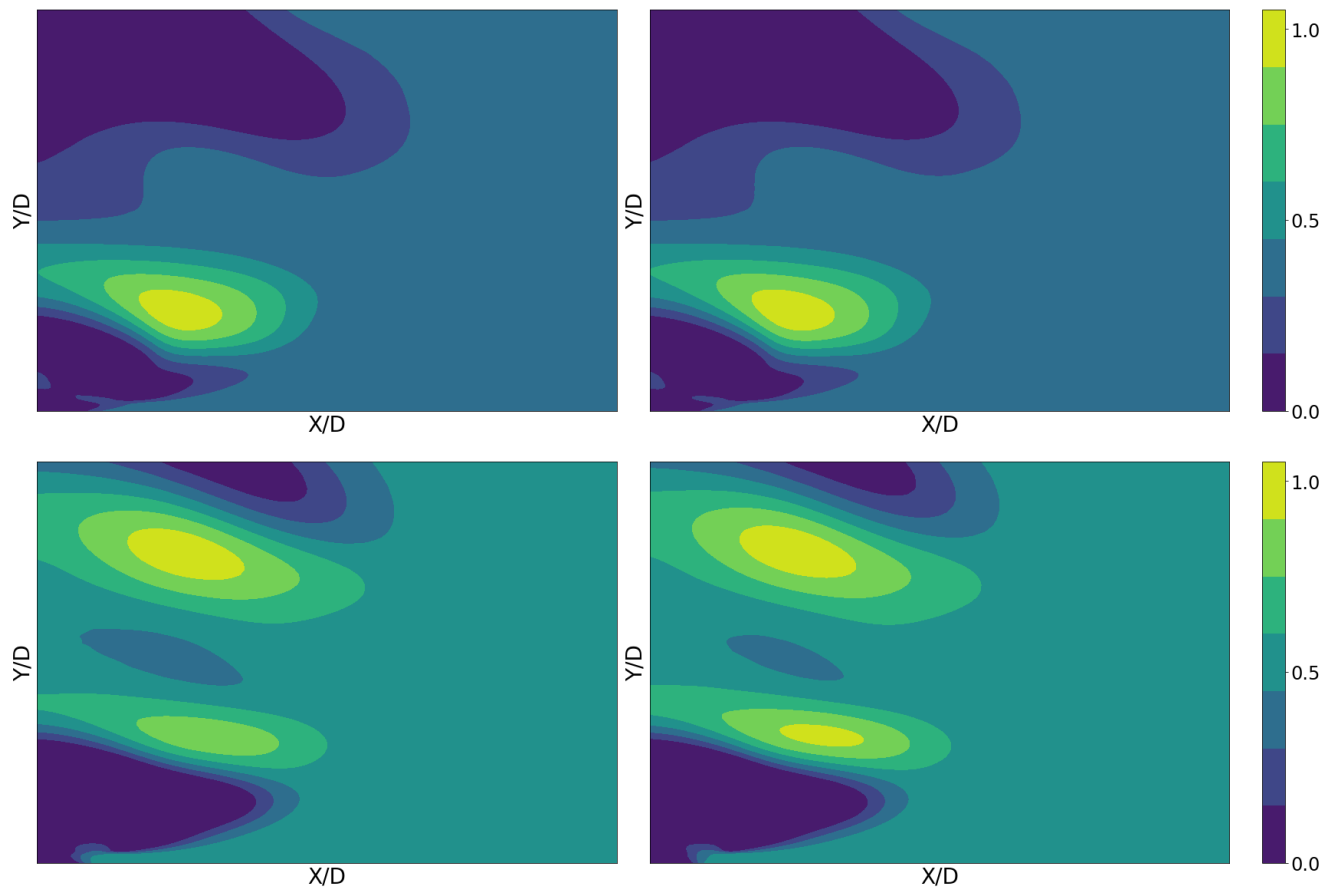

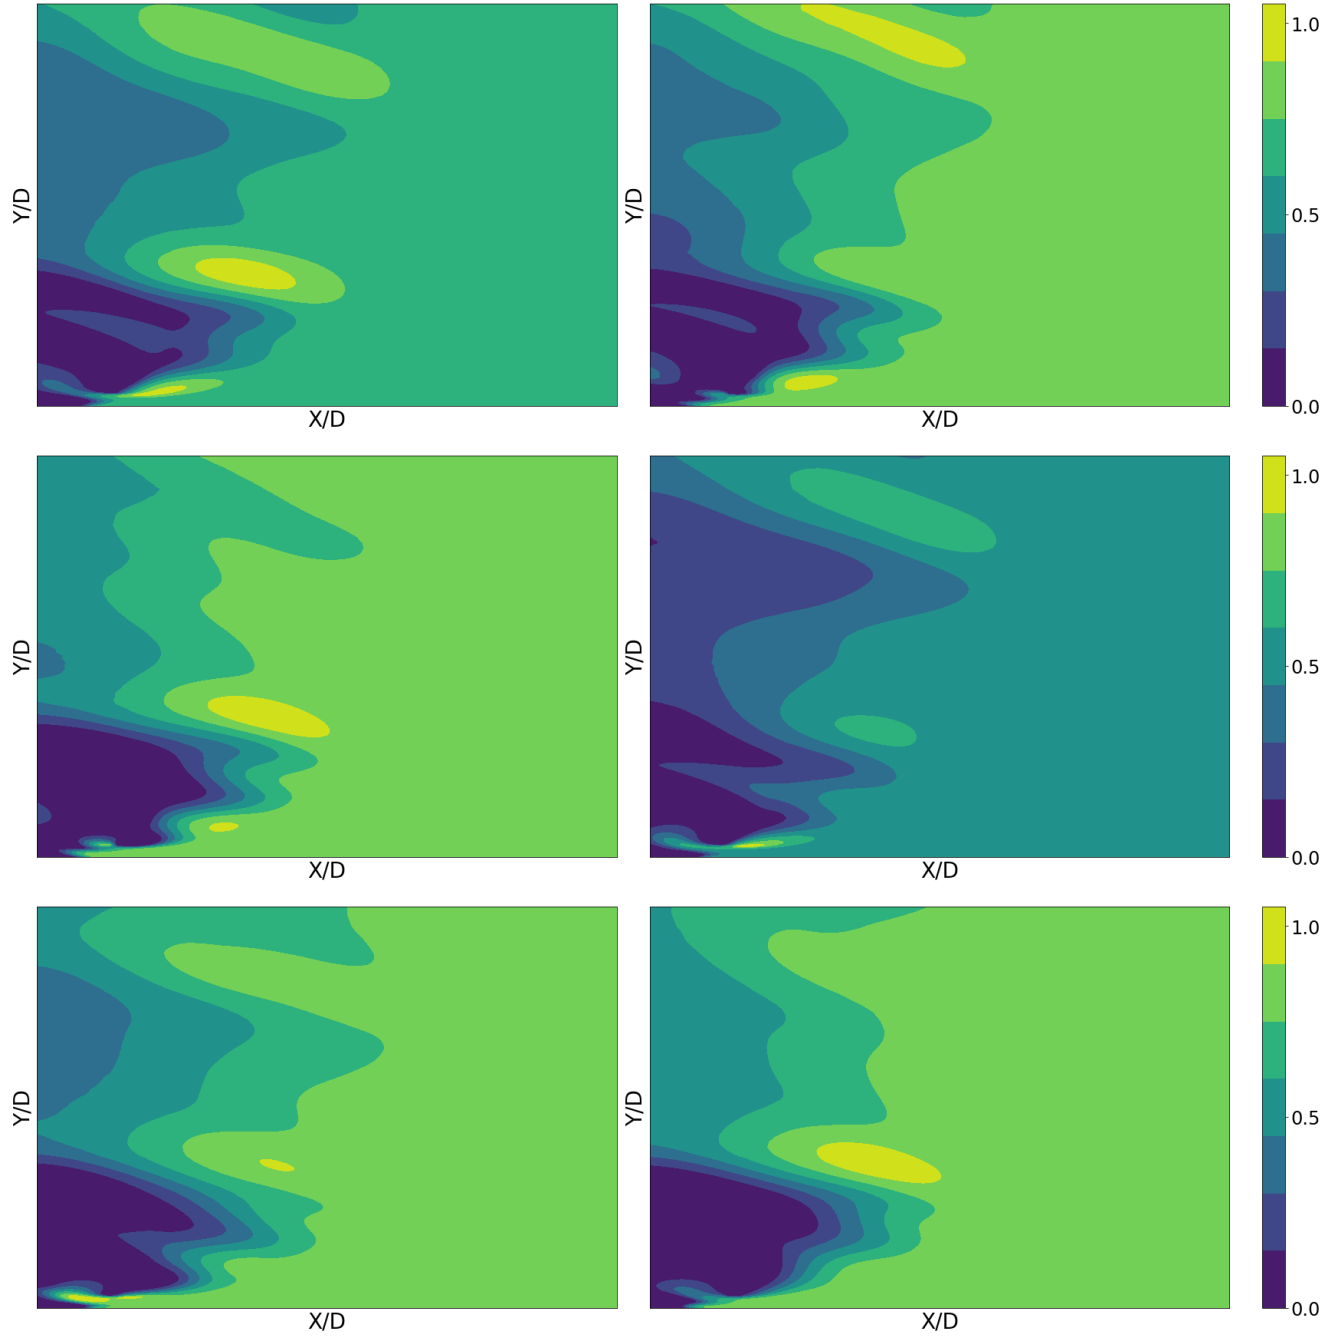

The normalized first five weighted 2D Proper Orthogonal Decomposition (POD) spatial modes, comparing lcSVD DA (left) with the ground truth (right) for the variable  $O_2$  in the laminar co flow flame dataset. With 20\% of modes retained, the modes are arranged from top to bottom in order of decreasing energy.

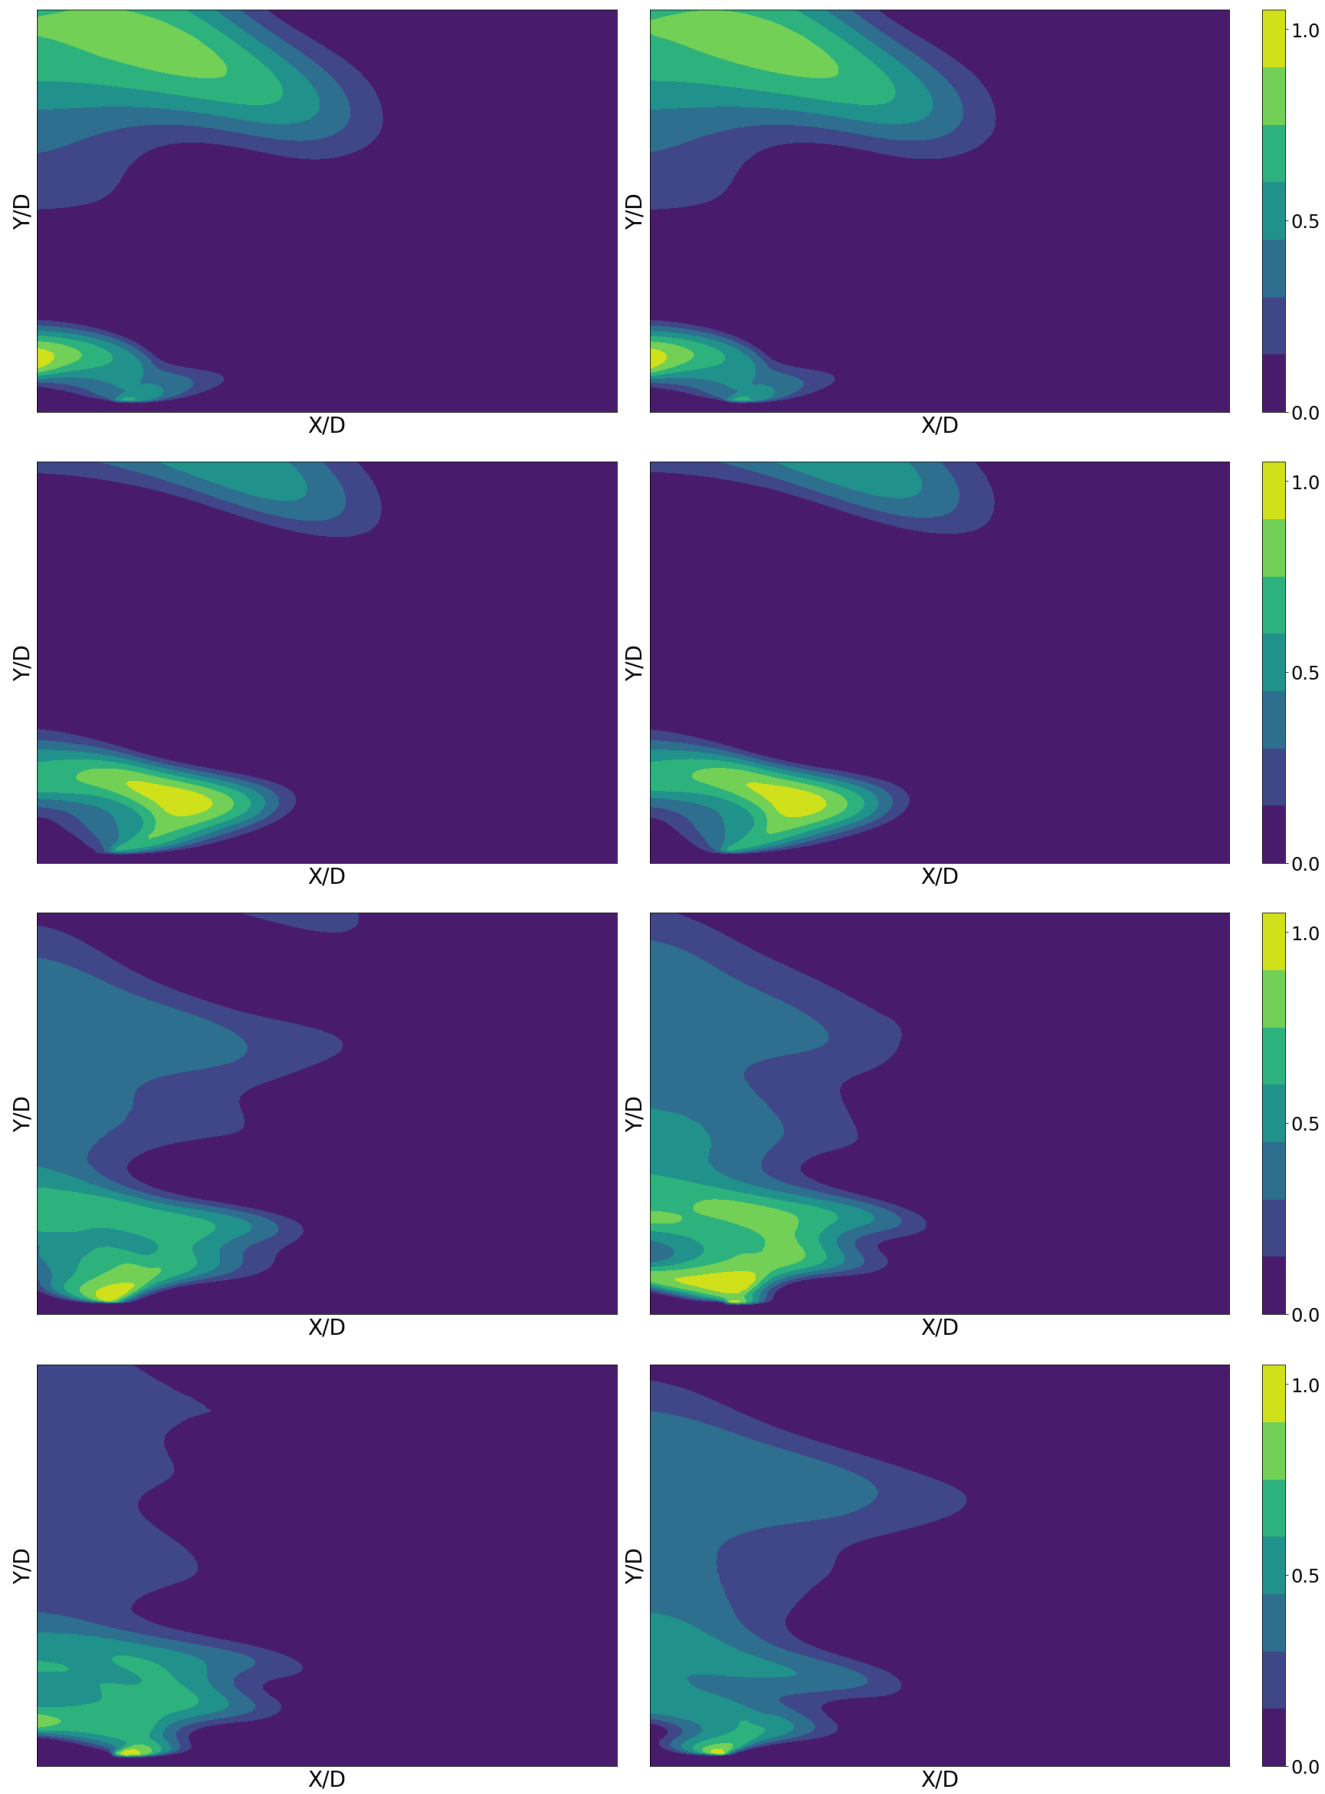

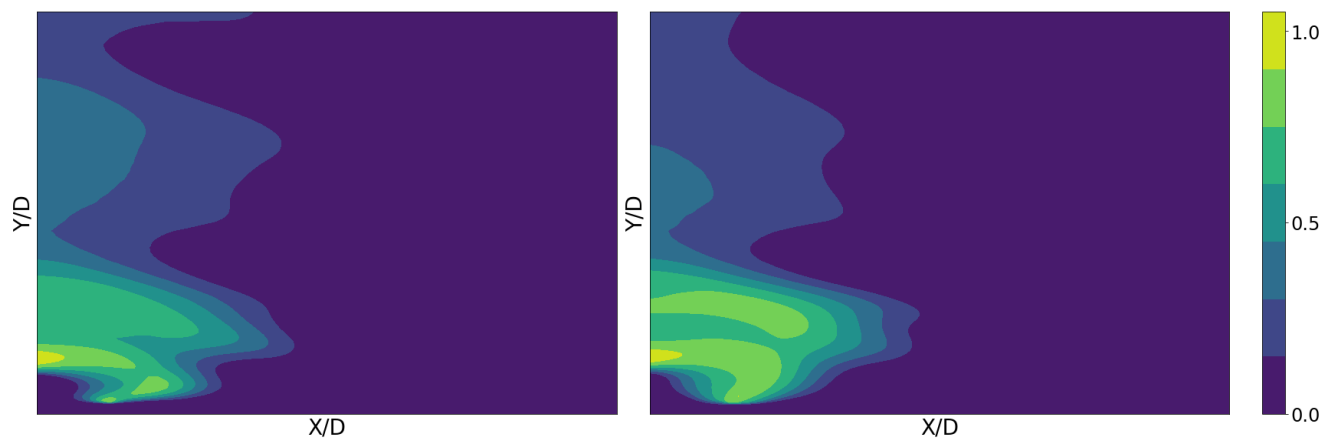

The normalized first five weighted 2D Proper Orthogonal Decomposition (POD) spatial modes, comparing lcSVD DA (left) with the ground truth (right) for the variable  $H_2O$  in the laminar co flow flame dataset. With 20% of modes retained, the modes are arranged from top to bottom in order of decreasing energy.

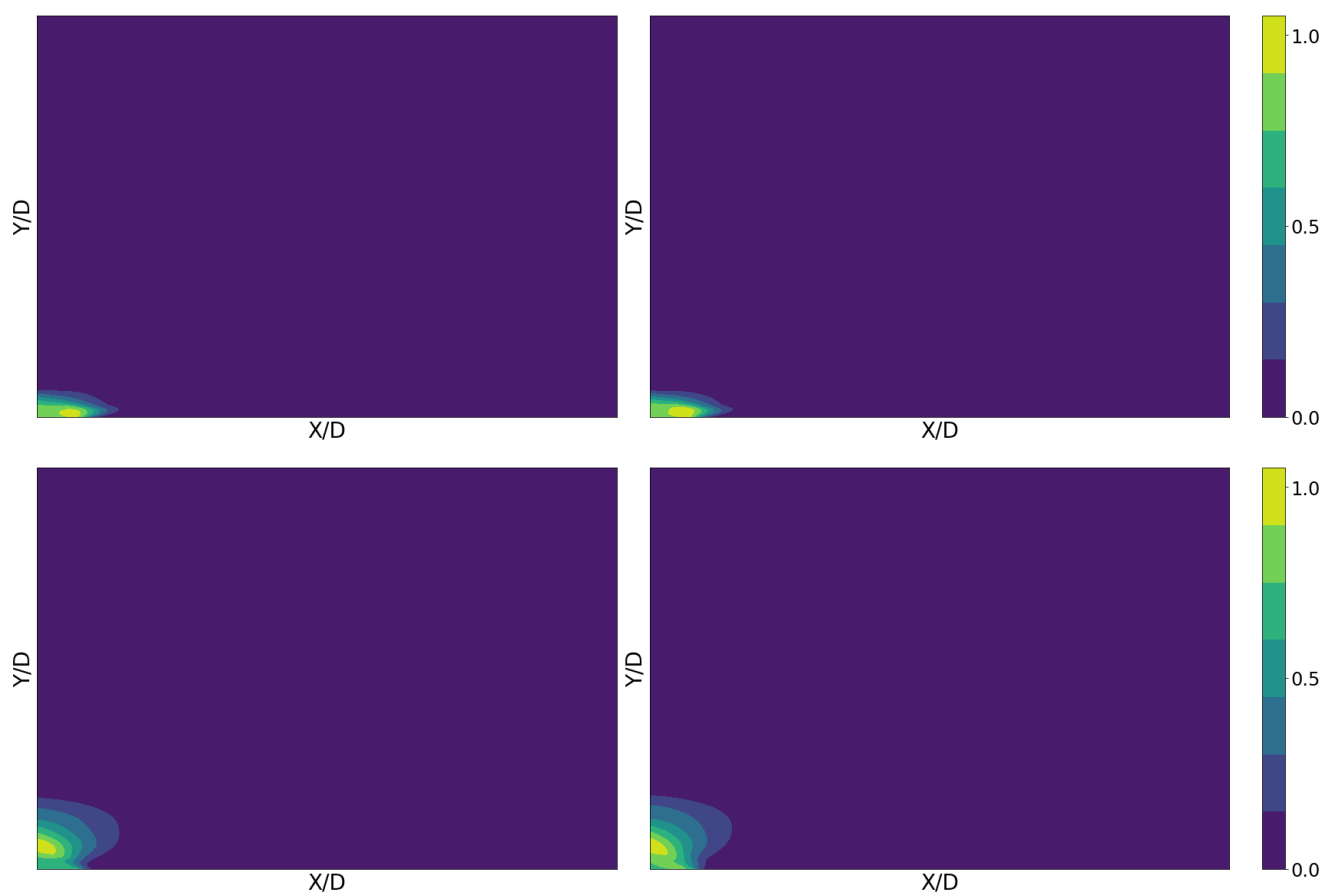

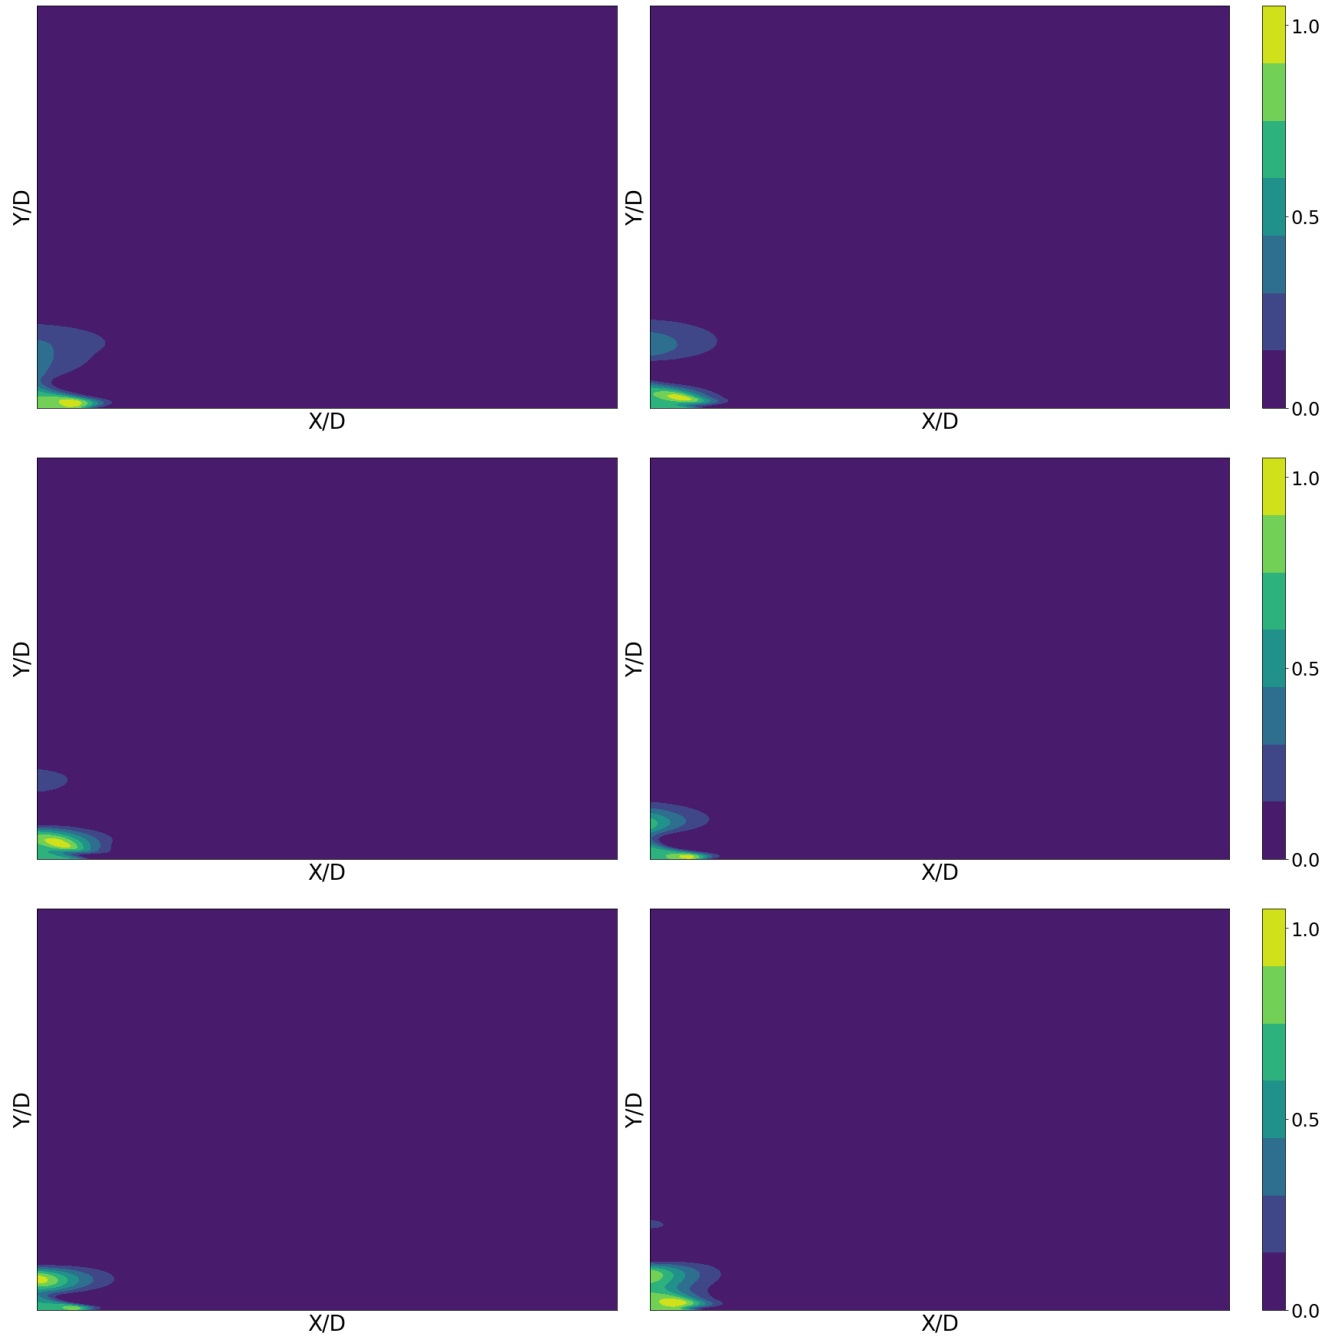

The normalized first five weighted 2D Proper Orthogonal Decomposition (POD) spatial modes, comparing lcSVD DA (left) with the ground truth (right) for the variable  $CH_4$  in the laminar co flow flame dataset. With 20\% of modes retained, the modes are arranged from top to bottom in order of decreasing energy.

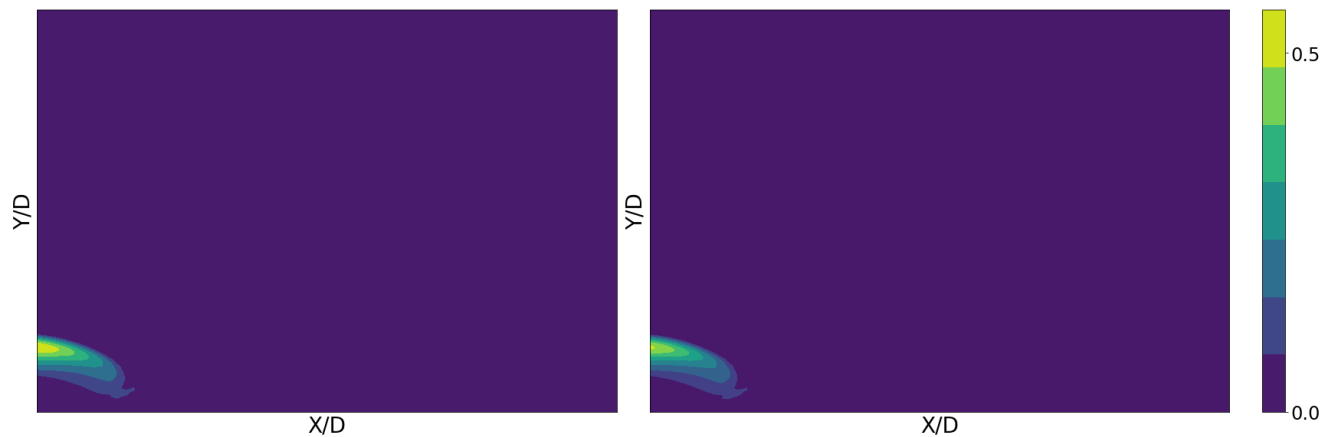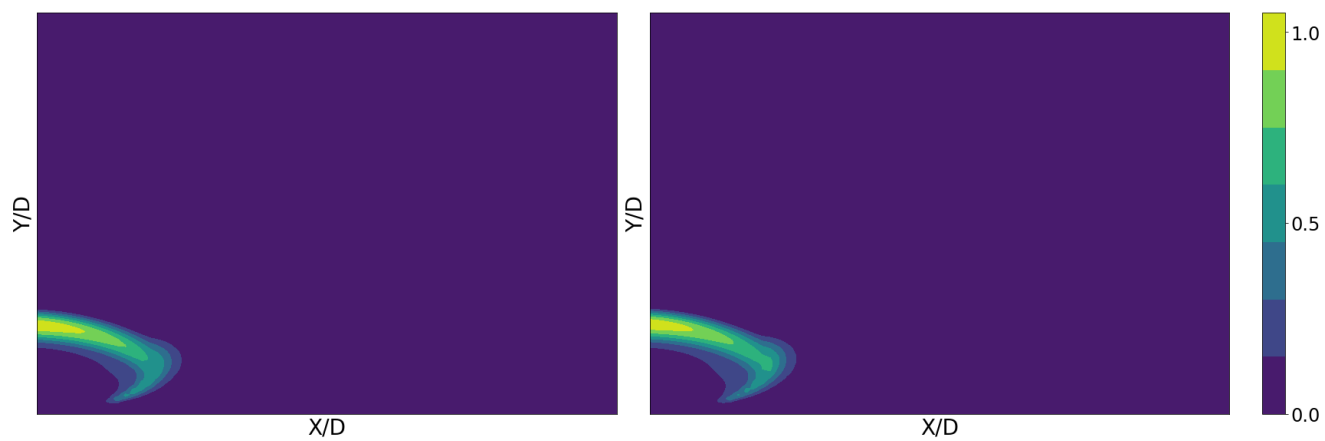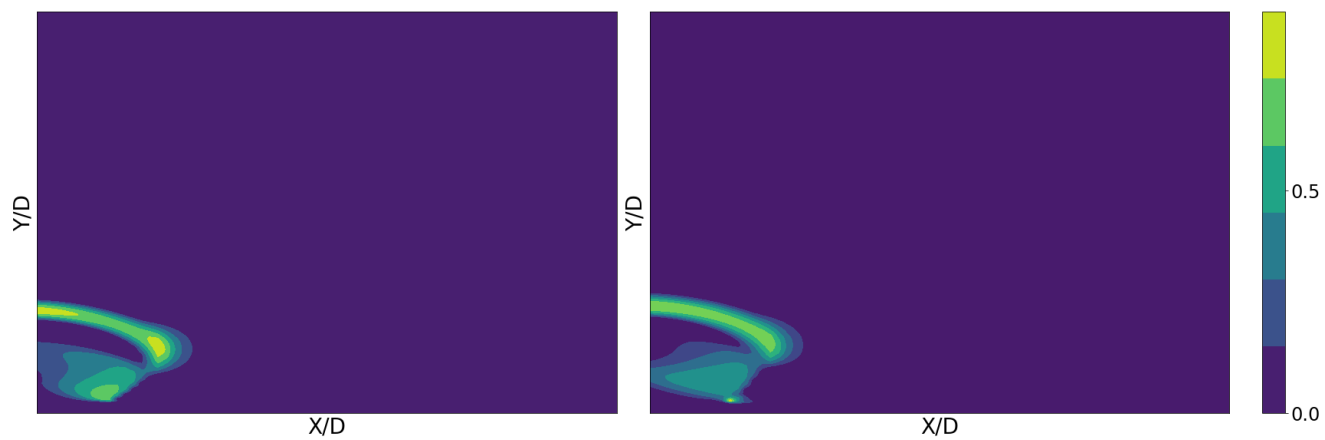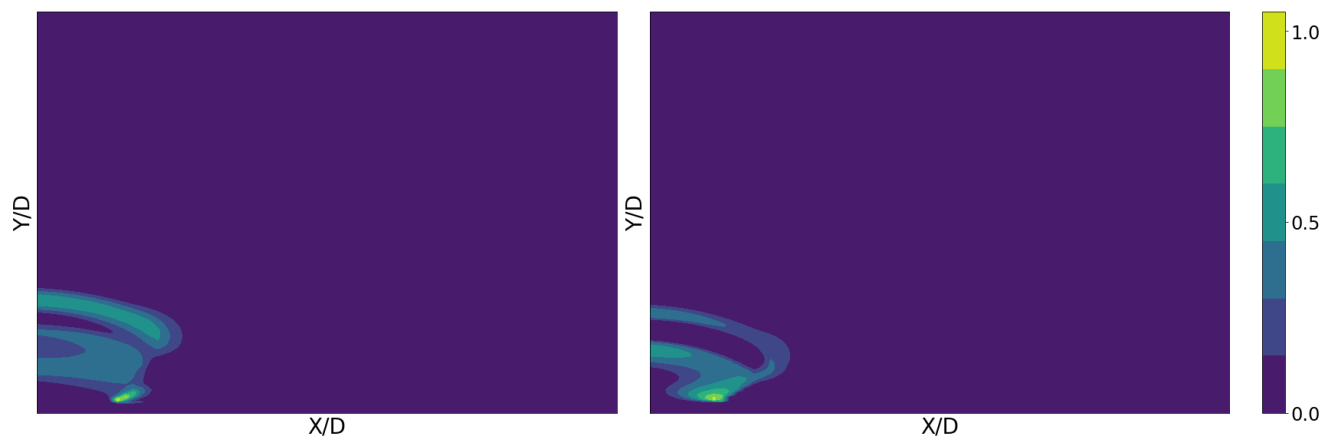

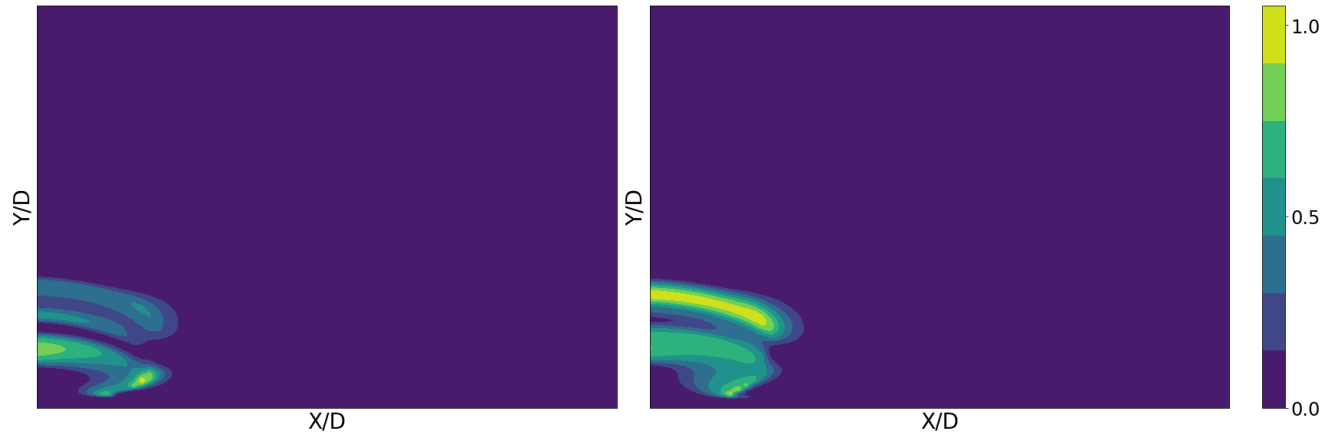

The normalized first five weighted 2D Proper Orthogonal Decomposition (POD) spatial modes, comparing lcSVD DA (left) with the ground truth (right) for the variable  $CO$  in the laminar co flow flame dataset. With 20\% of modes retained, the modes are arranged from top to bottom in order of decreasing energy.

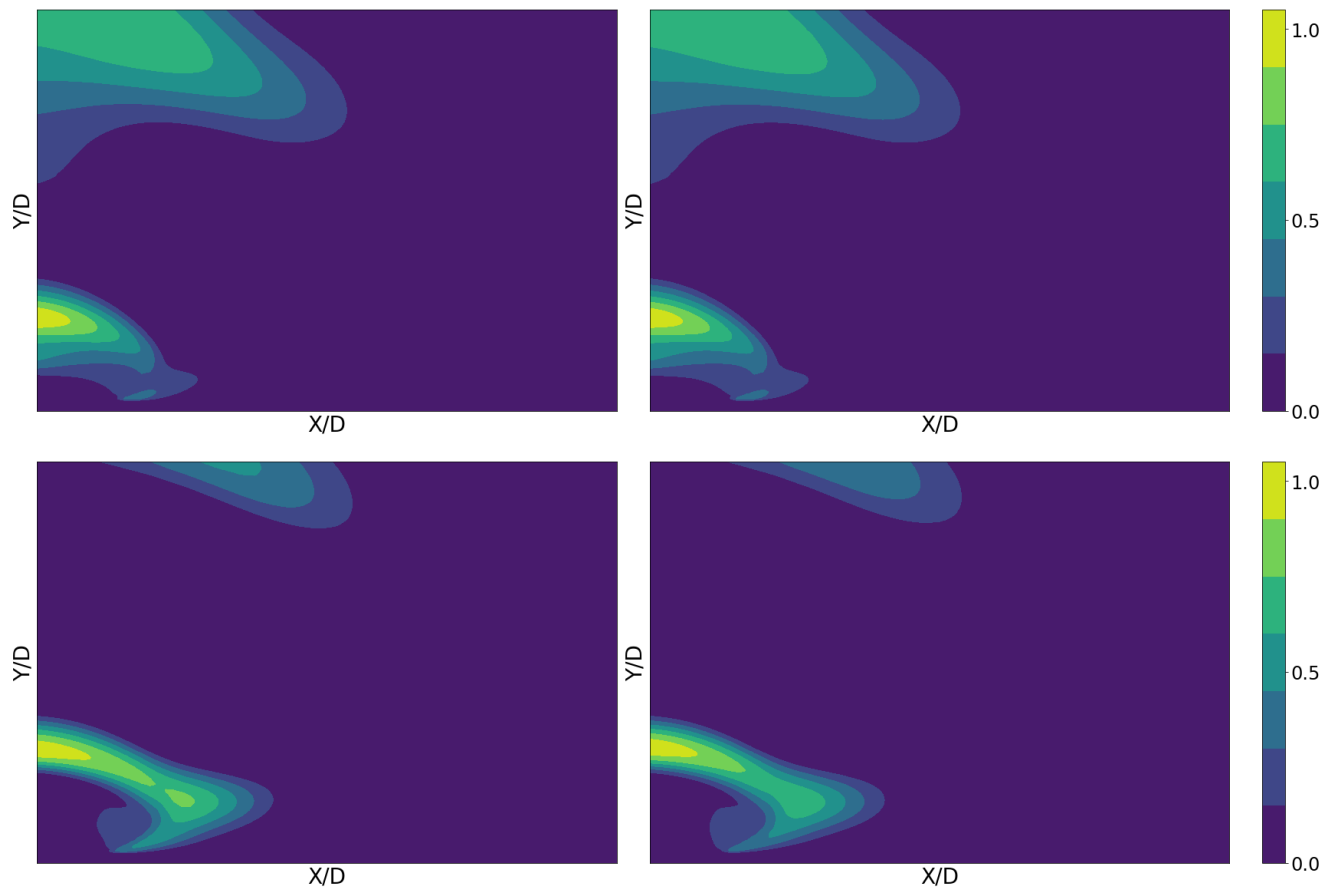

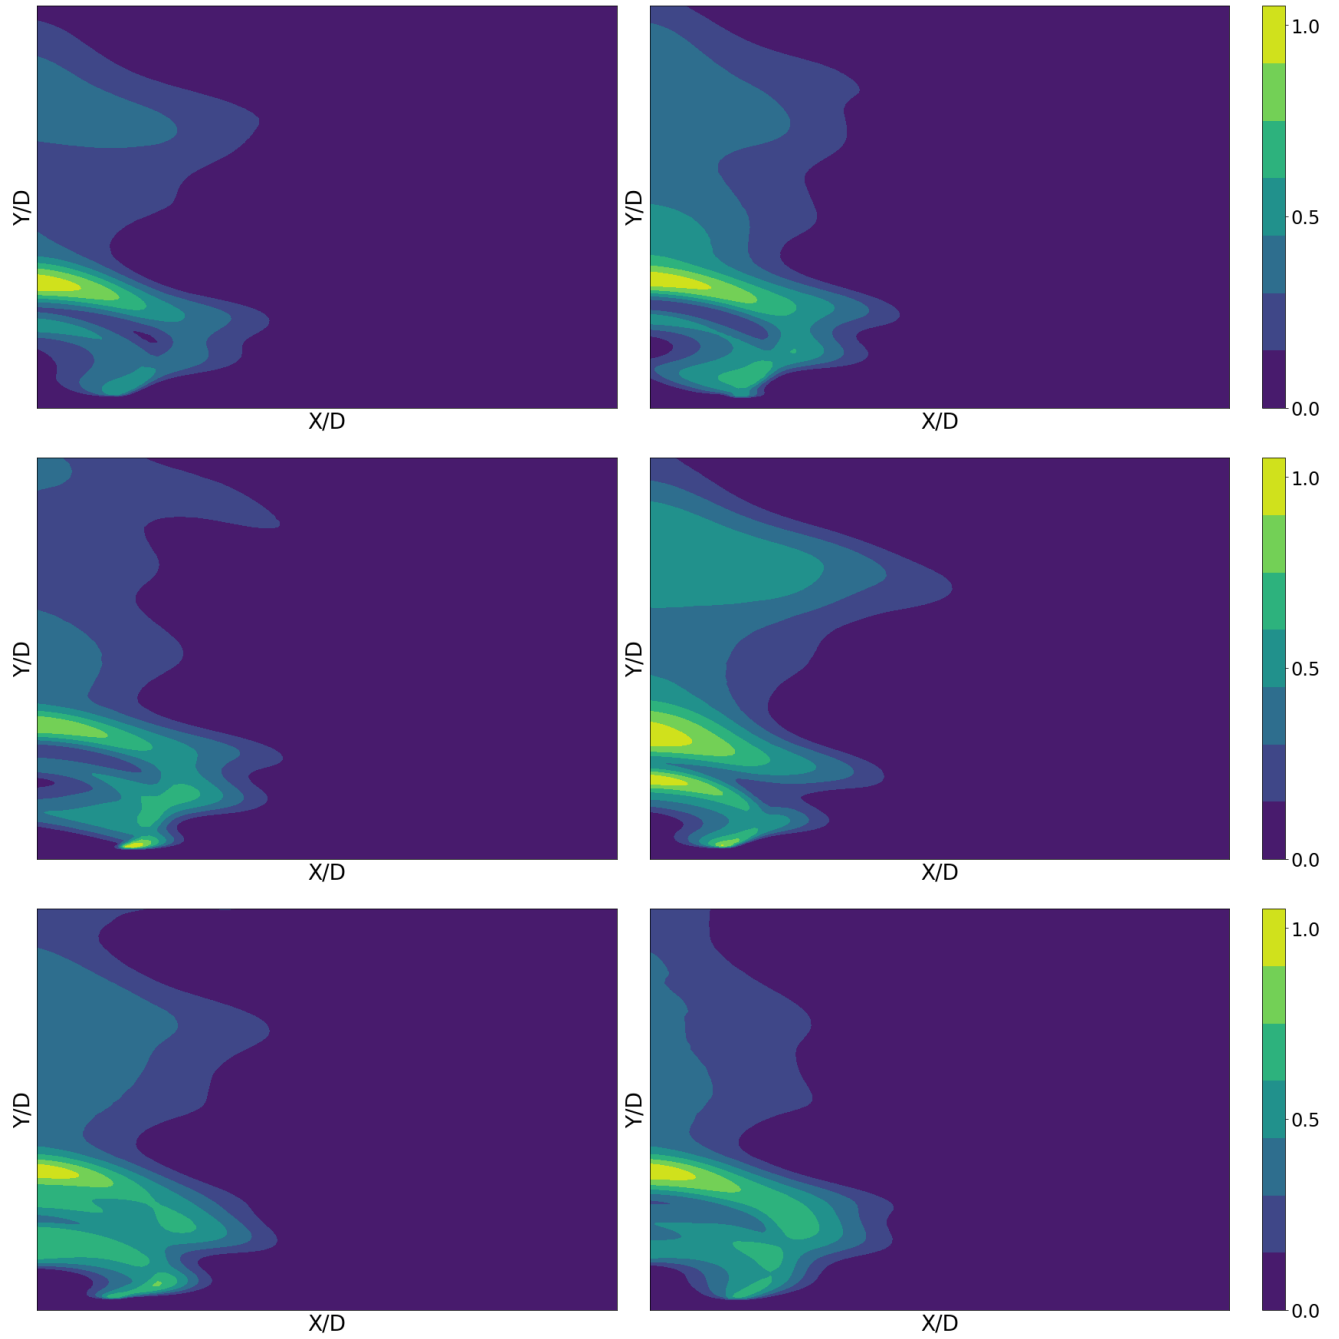

The normalized first five weighted 2D Proper Orthogonal Decomposition (POD) spatial modes, comparing lcSVD DA (left) with the ground truth (right) for the variable  $CO_2$  in the laminar co flow flame dataset. With 20\% of modes retained, the modes are arranged from top to bottom in order of decreasing energy.

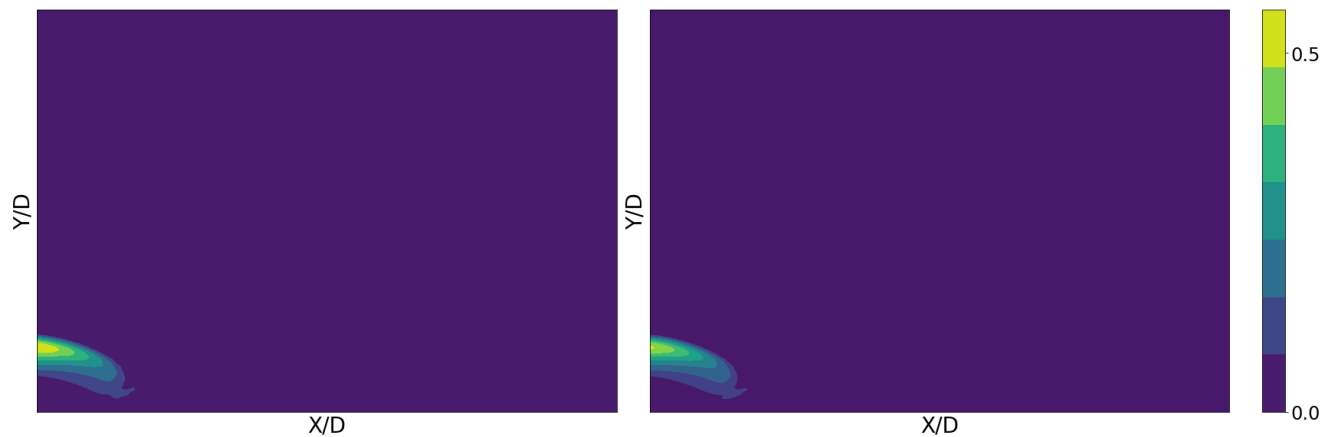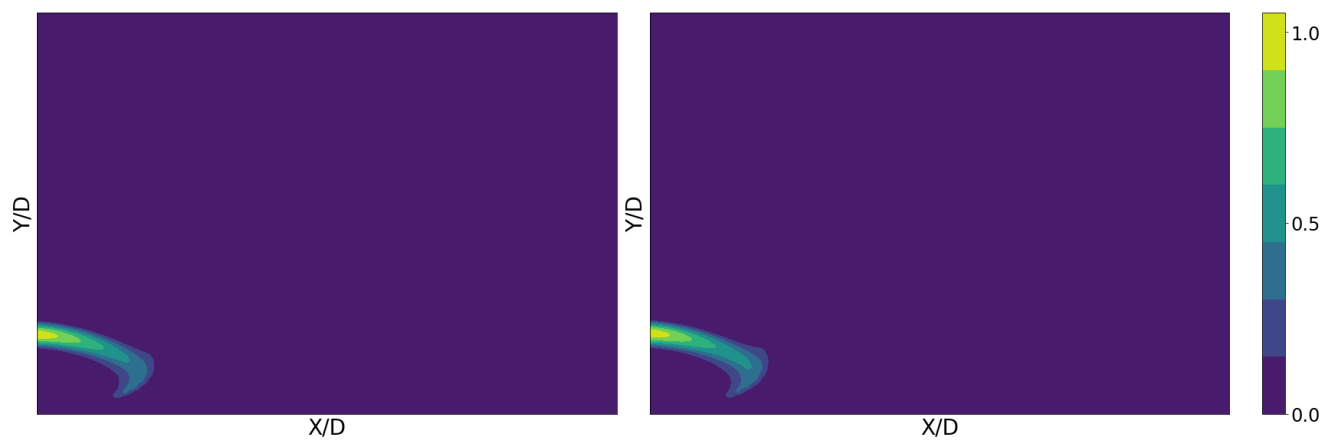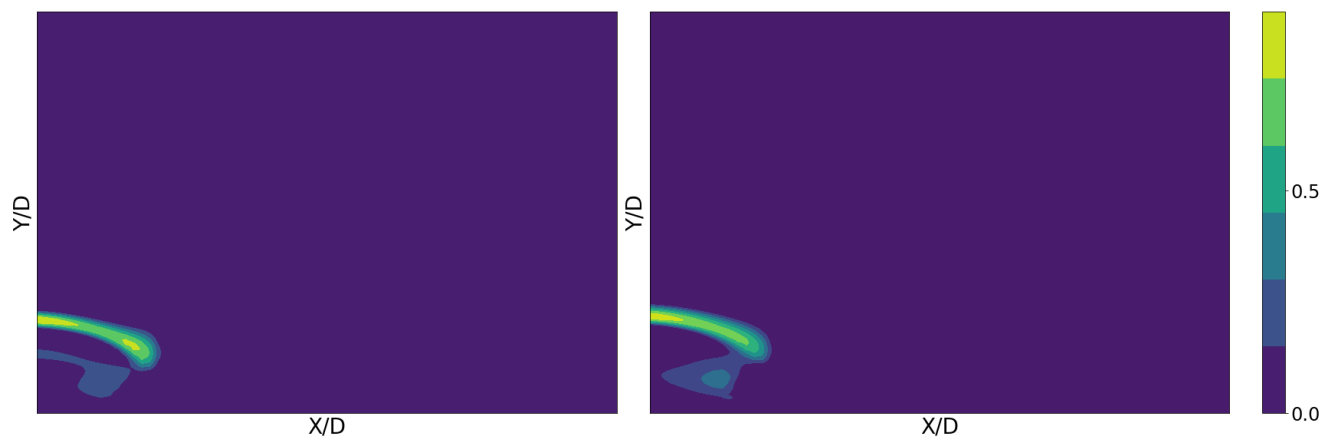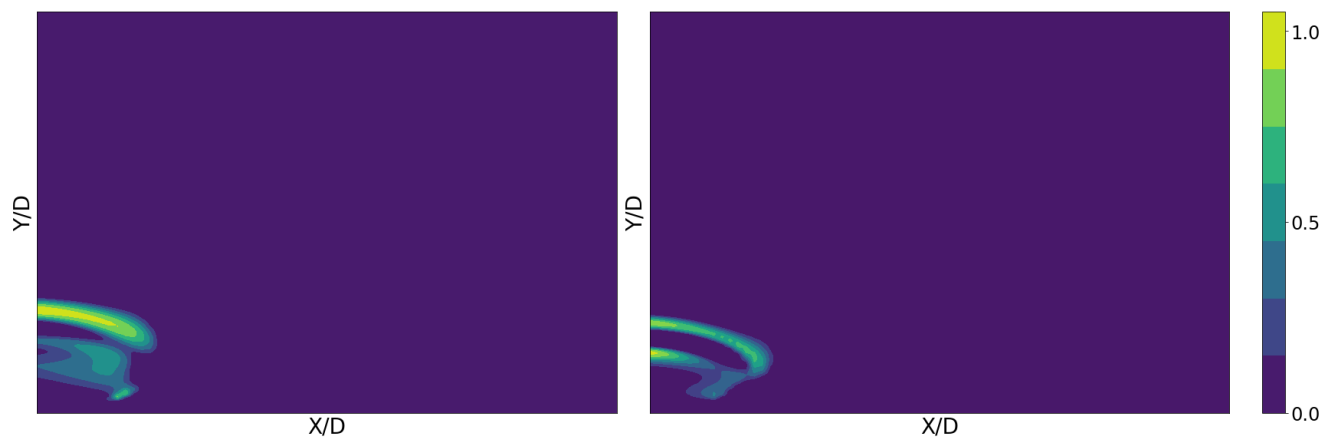

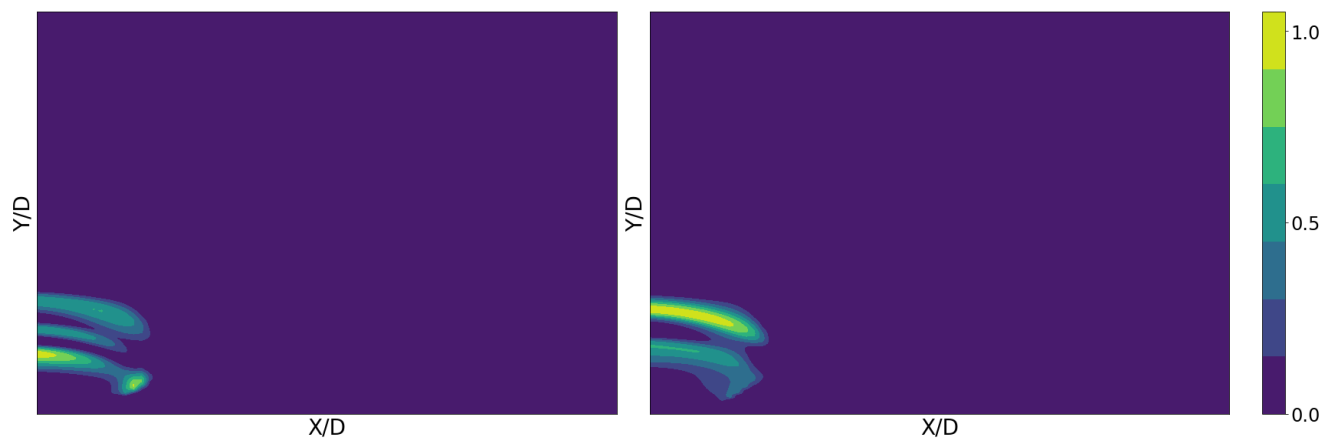

The normalized first five weighted 2D Proper Orthogonal Decomposition (POD) spatial modes, comparing lcSVD DA (left) with the ground truth (right) for the variable  $C_2H_2$  in the laminar co flow flame dataset. With 20\% of modes retained, the modes are arranged from top to bottom in order of decreasing energy.

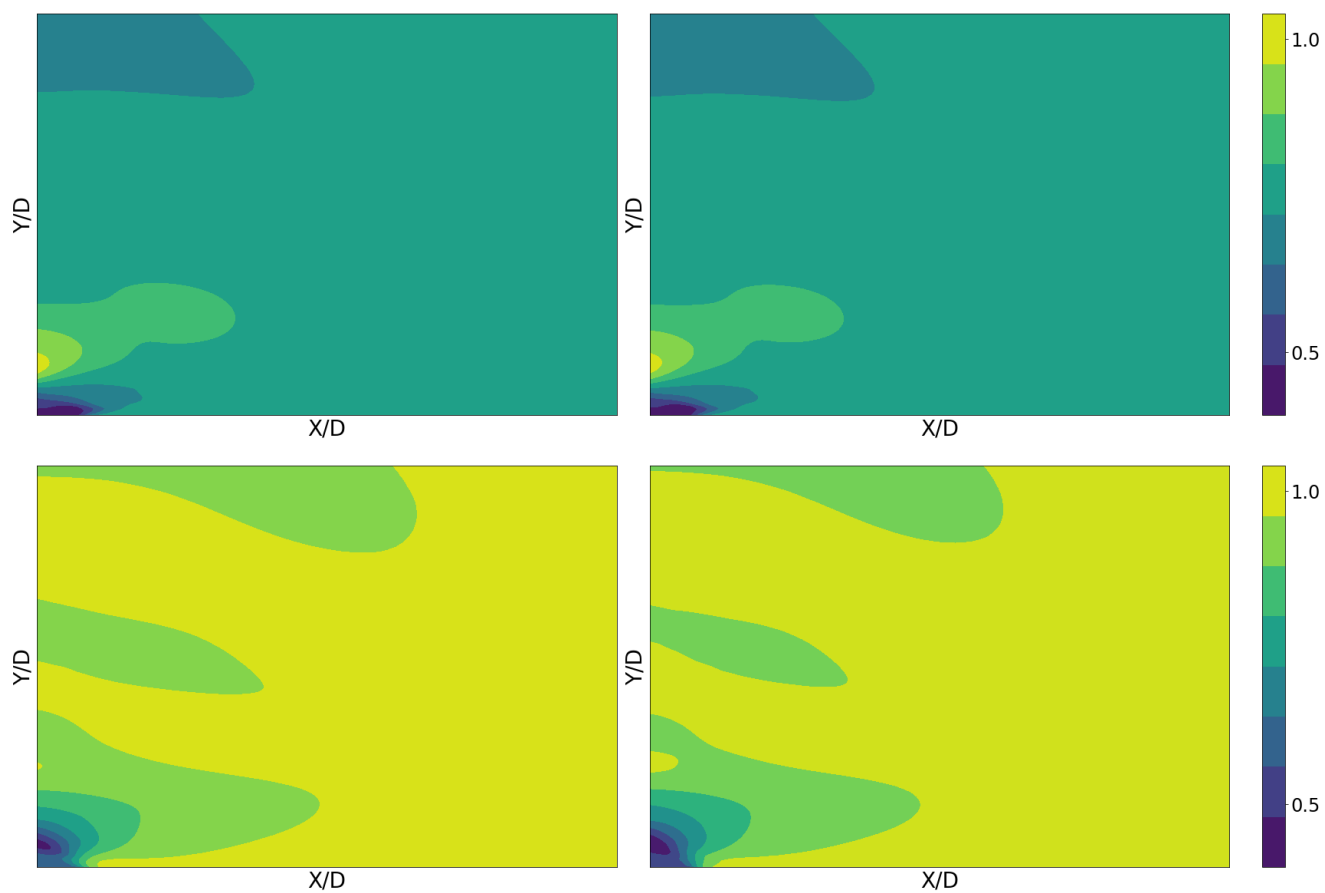

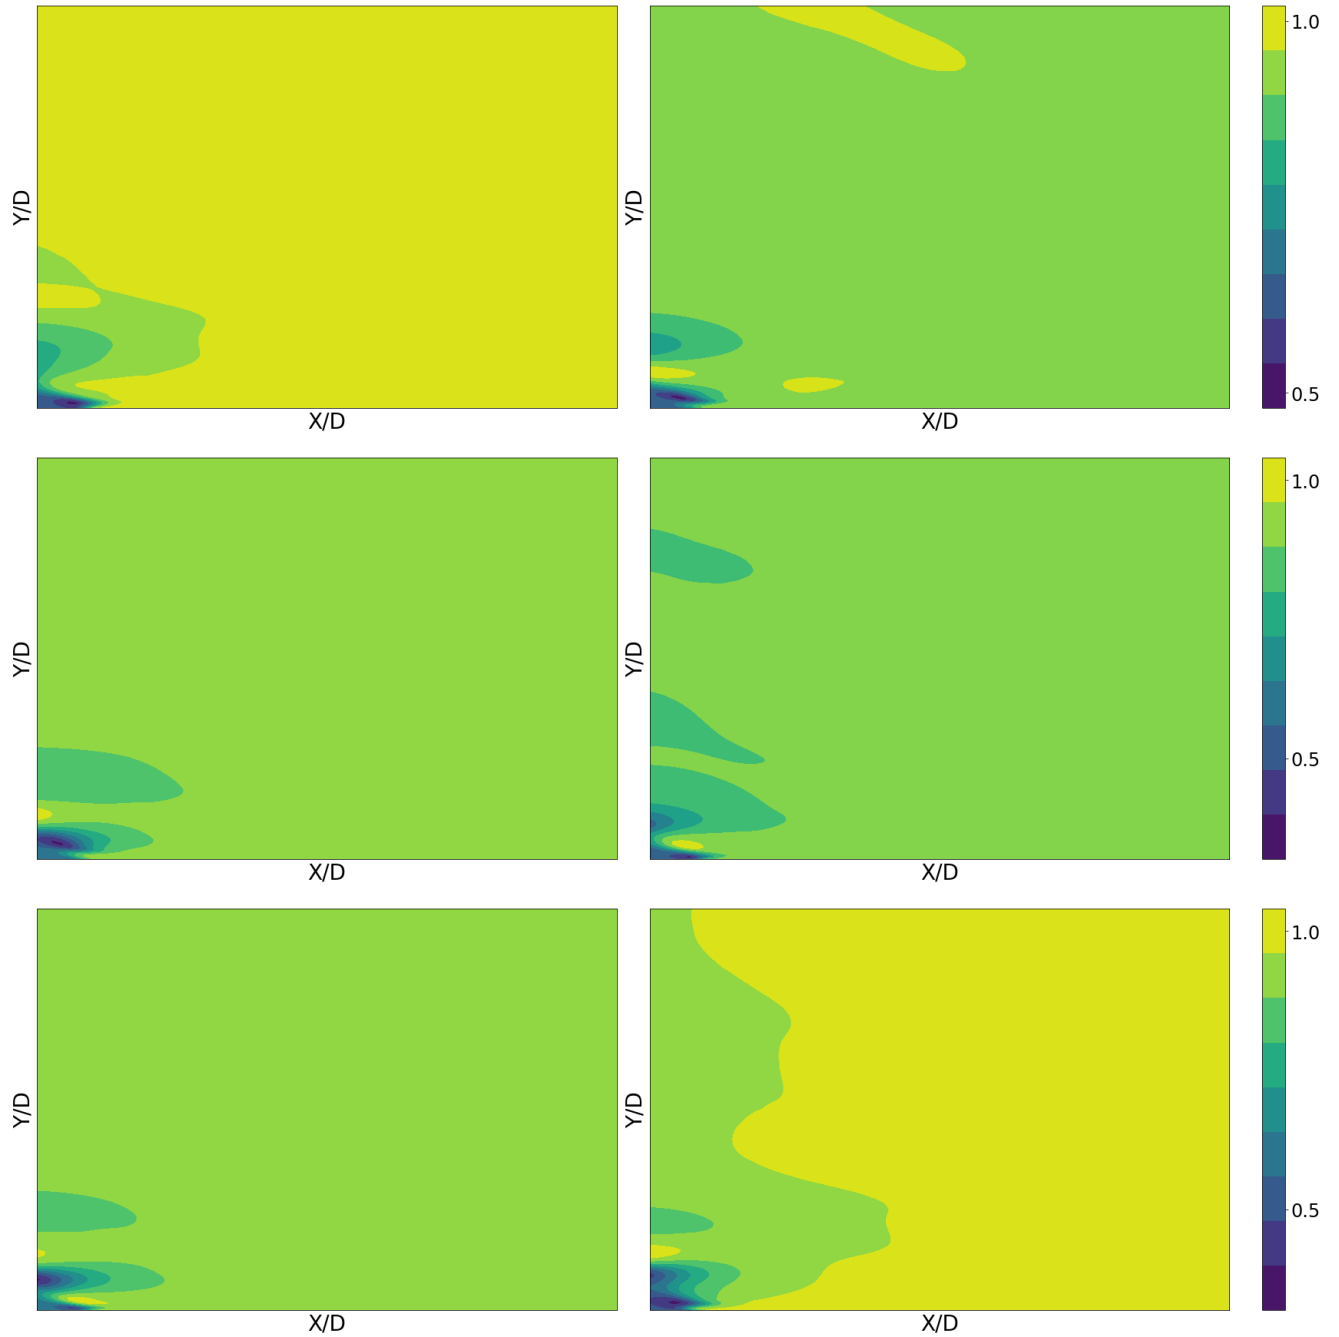

The normalized first five weighted 2D Proper Orthogonal Decomposition (POD) spatial modes, comparing lcSVD DA (left) with the ground truth (right) for the variable  $N_2$  in the laminar co flow flame dataset. With 20\% of modes retained, the modes are arranged from top to bottom in order of decreasing energy.

Turbulent bluff body stabilized flame with hydrogen as fuel. (2D POD modes comparison)

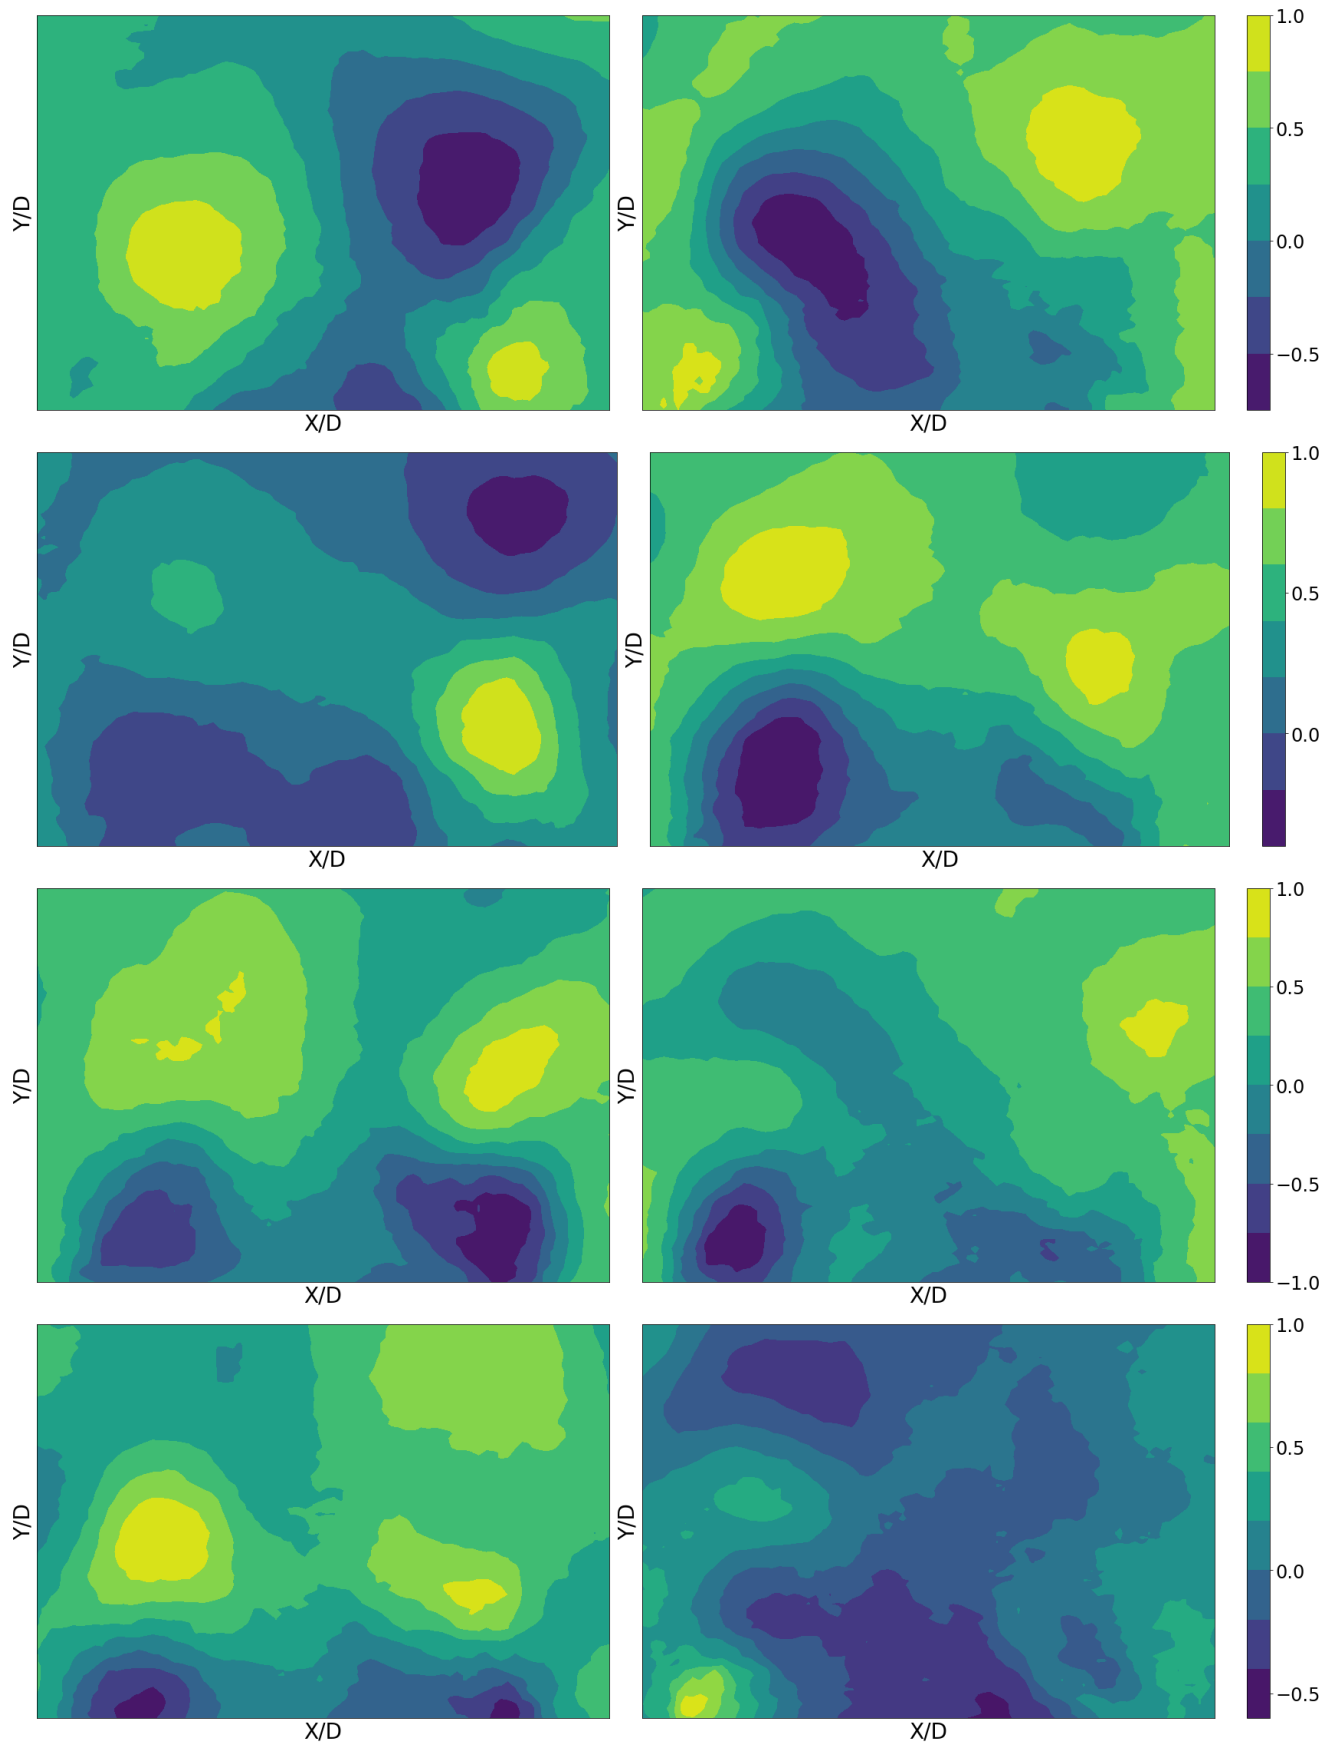

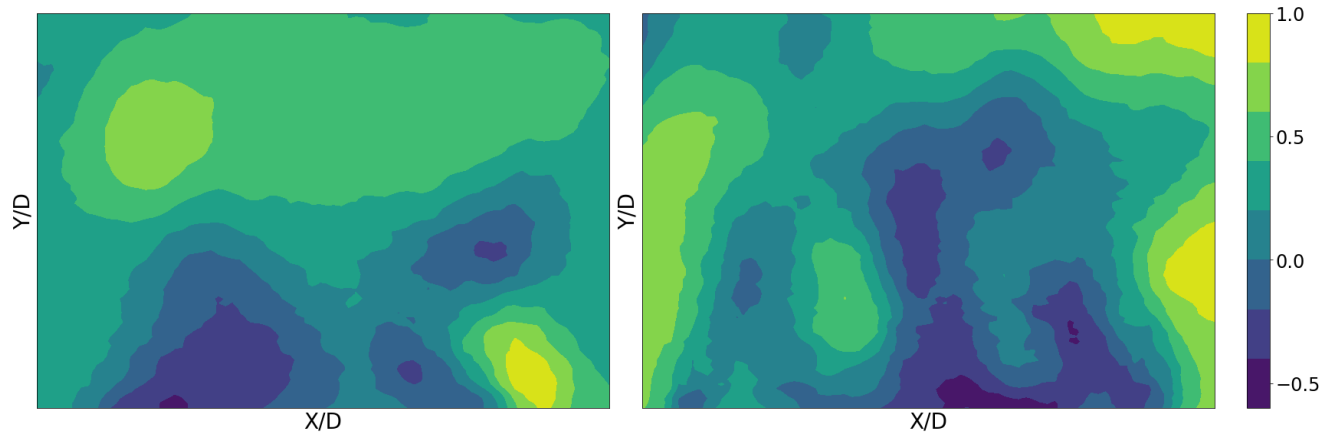

The normalized first five weighted 2D Proper Orthogonal Decomposition (POD) spatial modes, comparing lcSVD using optimum sensors (left) with the ground truth (right) for the variable normal velocity in the turbulent bluff body stabilized hydrogen flame dataset. With 20% of modes retained, the modes are arranged from top to bottom in order of decreasing energy.

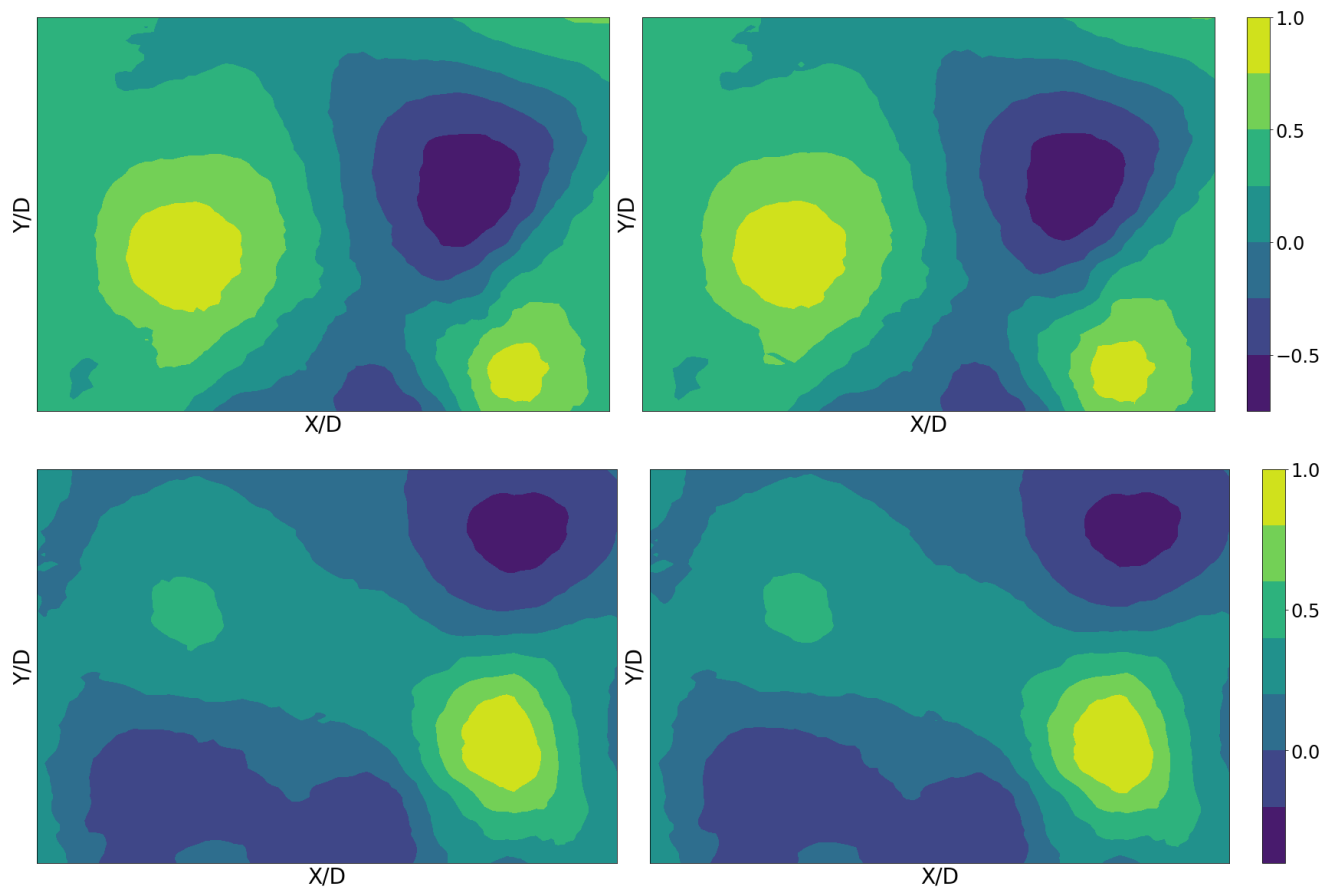

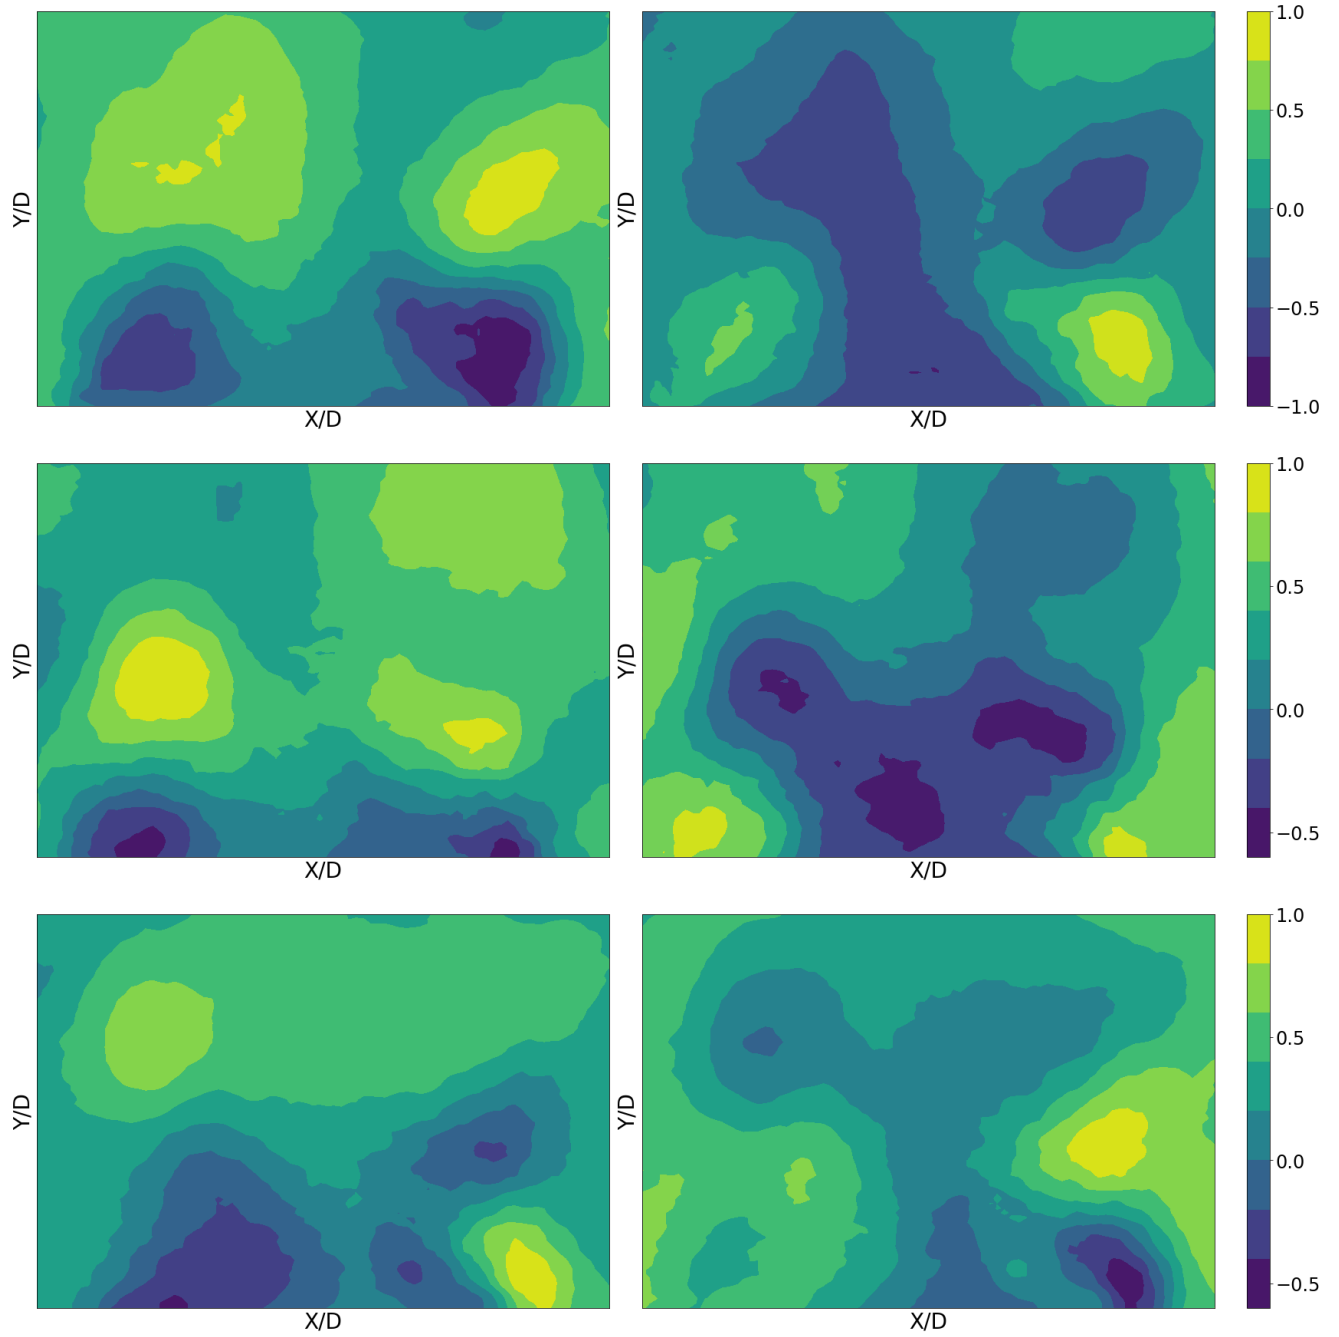

The normalized first five weighted 2D Proper Orthogonal Decomposition (POD) spatial modes, comparing lcSVD using equally spaced samples (left) with the ground truth (right) for the variable normal velocity in the turbulent bluff body stabilized hydrogen flame dataset. With 20% of modes retained, the modes are arranged from top to bottom in order of decreasing energy.

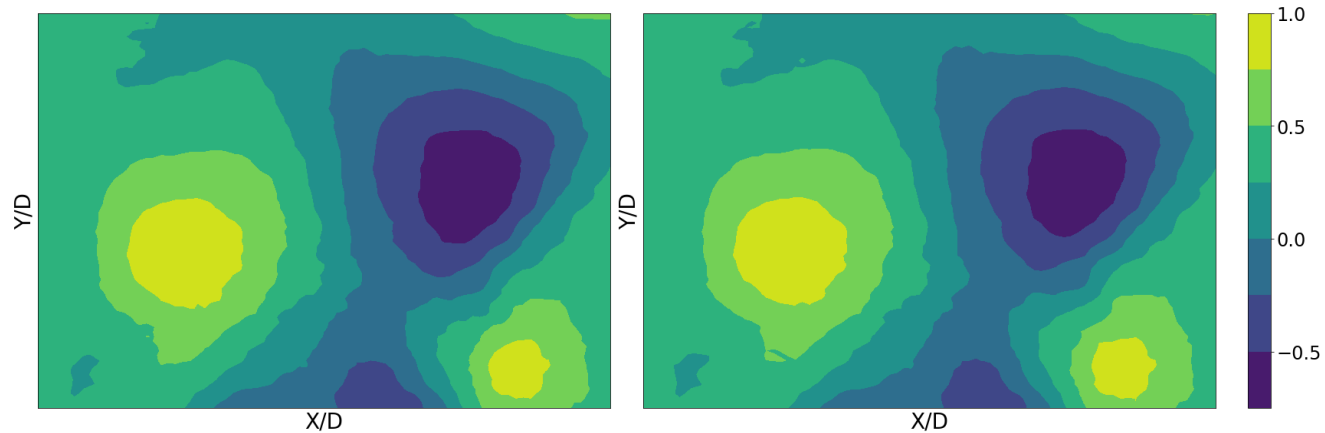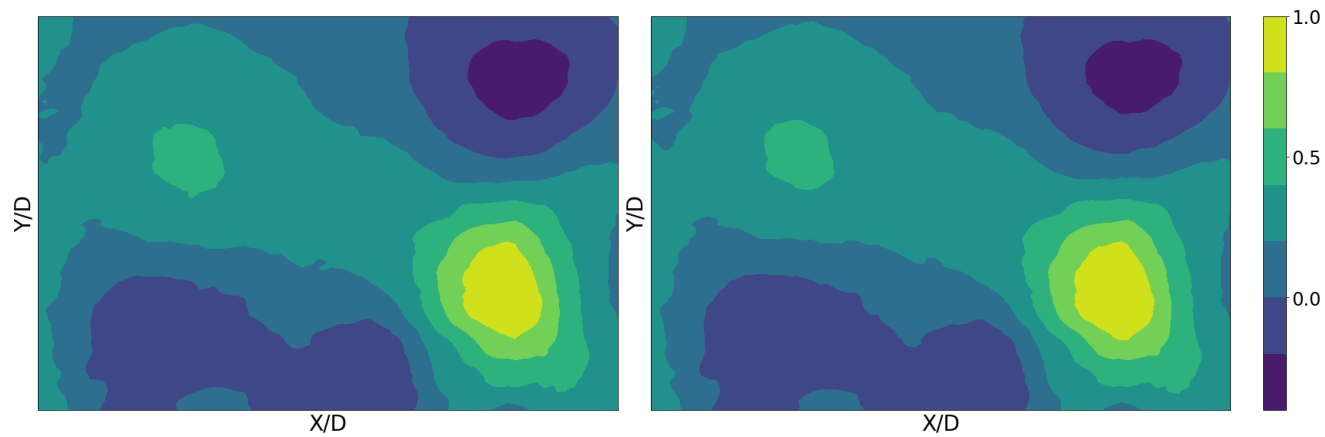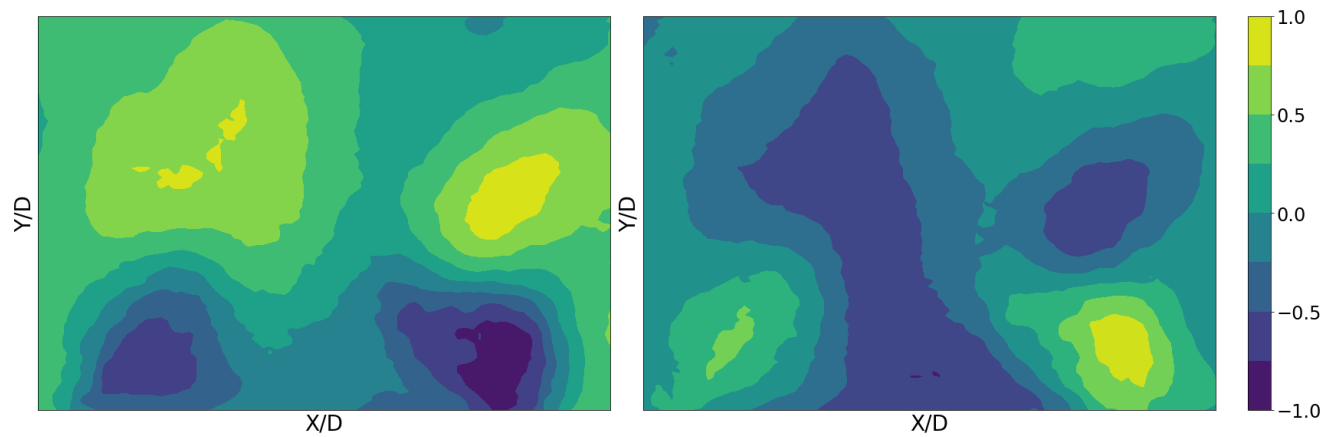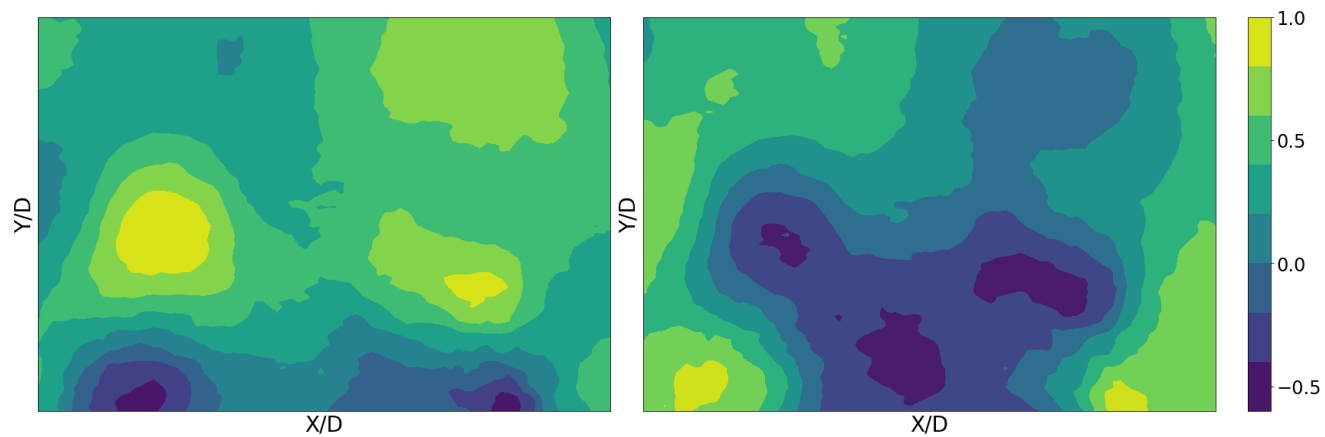

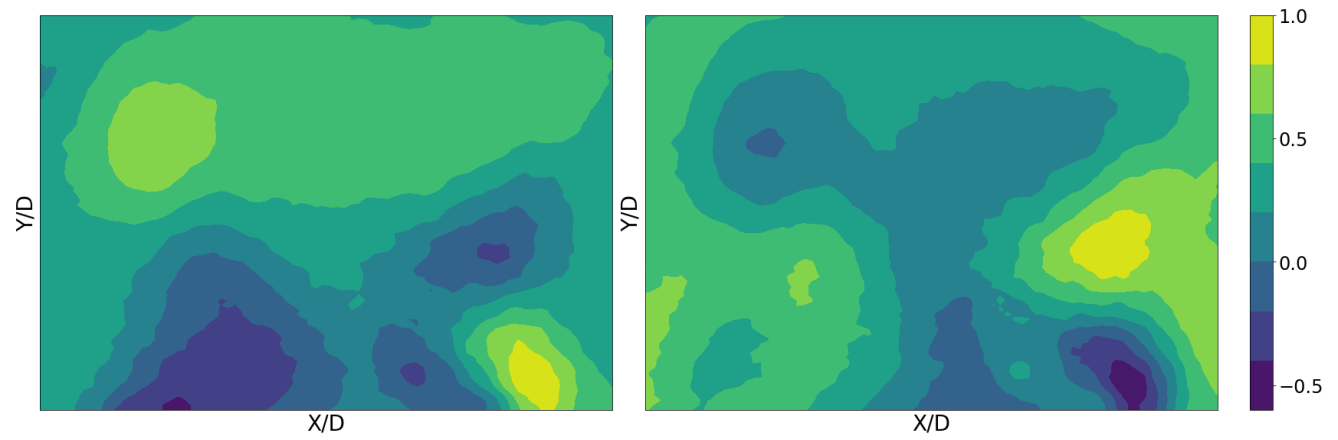

The normalized first five weighted 2D Proper Orthogonal Decomposition (POD) spatial modes, comparing lcSVD DA(left) with the ground truth (right) for the variable normal velocity in the turbulent bluff body stabilized hydrogen flame dataset. With 20% of modes retained, the modes are arranged from top to bottom in order of decreasing energy.
